# Supplementary material for: Excited State Absorption: Reference Oscillator Strengths, Wavefunction and TD-DFT Benchmarks
Source: arXiv:2501.17114 ancillary file (2025-01-28)
Supplement: Supplementary file 1 [file SI.pdf]

# Supporting Information for: Excited State Absorption: Reference Oscillator Strengths, Wavefunction and TD-DFT Benchmarks

Jakub Širůček,<sup>†,‡</sup> Boris Le Guennic,<sup>\*,‡</sup> Yann Damour,<sup>¶</sup> Pierre-François Loos,<sup>\*,¶</sup>  
and Denis Jacquemin<sup>\*,†,§</sup>

<sup>†</sup>*Nantes Université, CNRS, CEISAM UMR 6230, F-44000 Nantes, France*

<sup>‡</sup>*Univ Rennes, CNRS, ISCR UMR 6226, F-35042 Rennes, France*

<sup>¶</sup>*Université de Toulouse, CNRS, UPS, Laboratoire de Chimie et Physique Quantiques UMR  
5626, F-31062 Toulouse, France*

<sup>§</sup>*Institut Universitaire de France (IUF), F-75005 Paris, France*

E-mail: Boris.Leguennic@univ-rennes.fr; loos@irsamc.ups-tlse.fr; Denis.Jacquemin@univ-nantes.fr

## Contents

|                                |           |
|--------------------------------|-----------|
| <b>S1 Geometries</b>           | <b>S4</b> |
| S1.1 Acetone . . . . .         | S4        |
| S1.2 Acrolein . . . . .        | S4        |
| S1.3 Amonia . . . . .          | S4        |
| S1.4 Benzene . . . . .         | S5        |
| S1.5 Butadiene . . . . .       | S5        |
| S1.6 Carbon monoxide . . . . . | S6        |
| S1.7 Cyclopentadiene . . . . . | S6        |

|                                                                                                           |            |
|-----------------------------------------------------------------------------------------------------------|------------|
| S1.8 Cyclopropene . . . . .                                                                               | S6         |
| S1.9 Diazirine . . . . .                                                                                  | S6         |
| S1.10Diazomethane . . . . .                                                                               | S7         |
| S1.11Dinitrogen . . . . .                                                                                 | S7         |
| S1.12Ethylene . . . . .                                                                                   | S7         |
| S1.13Formaldehyde . . . . .                                                                               | S7         |
| S1.14Furan . . . . .                                                                                      | S8         |
| S1.15Glyoxal . . . . .                                                                                    | S8         |
| S1.16Hexatriene . . . . .                                                                                 | S8         |
| S1.17Ketene . . . . .                                                                                     | S9         |
| S1.18Methylenecyclopropene . . . . .                                                                      | S9         |
| S1.19Pyrazine . . . . .                                                                                   | S9         |
| S1.20Pyridazine . . . . .                                                                                 | S10        |
| S1.21Pyridine . . . . .                                                                                   | S10        |
| S1.22Pyrimidine . . . . .                                                                                 | S10        |
| S1.23Pyrrole . . . . .                                                                                    | S11        |
| S1.24Silylidene . . . . .                                                                                 | S11        |
| S1.25Tetrazine . . . . .                                                                                  | S11        |
| S1.26Thiophene . . . . .                                                                                  | S12        |
| S1.27Water . . . . .                                                                                      | S12        |
| <b>S2 Ground state absorption data</b>                                                                    | <b>S13</b> |
| S2.1 Small set of transitions, large basis sets . . . . .                                                 | S13        |
| S2.2 Full testing set, LR-CC3, LR-CCSD, LR-CC2, with AVDZ, dAVDZ, AVTZ,<br>and dAVTZ basis sets . . . . . | S20        |
| S2.3 Full testing set, ISR-ADC(2) with AVDZ, dAVDZ, AVTZ, and dAVTZ basis sets                            | S39        |
| S2.4 Full testing set ISR-ADC(3), EOM-CCSD, LR-TDDFT and LR-TDA (dAVTZ)                                   | S43        |

|                                                                                                           |             |
|-----------------------------------------------------------------------------------------------------------|-------------|
| <b>S3 Excited state absorption data</b>                                                                   | <b>S59</b>  |
| S3.1 Transition dipole moments, small set of transitions . . . . .                                        | S59         |
| S3.2 Small set of transitions, large basis sets . . . . .                                                 | S61         |
| S3.3 Full testing set, QR-CC3, QR-CCSD, QR-CC2, with AVDZ, dAVDZ, AVTZ,<br>and dAVTZ basis sets . . . . . | S68         |
| S3.4 Full testing set, ISR-ADC2 with AVDZ, dAVDZ, AVTZ, and dAVTZ basis sets                              | S87         |
| S3.5 Full testing set ISR-ADC(3), EOM-CCSD, QR-TDDFT and QR-TDA (dAVTZ)                                   | S91         |
| <b>S4 Statistics</b>                                                                                      | <b>S108</b> |
| S4.1 Reference Value . . . . .                                                                            | S108        |
| S4.2 Basis Set Effect . . . . .                                                                           | S108        |
| S4.3 Methods Benchmarks . . . . .                                                                         | S110        |
| <b>References</b>                                                                                         | <b>S114</b> |

## S1 Geometries

Below, we provide the Cartesian coordinates of the compounds investigated in this study. These are provided in atomic units (bohr) and they have been taken for the QUEST database (CC3/AVTZ).<sup>1</sup>

### S1.1 Acetone

|   |             |             |             |
|---|-------------|-------------|-------------|
| C | 0.00000000  | 0.00000000  | 0.18807702  |
| C | 0.00000000  | 2.42007545  | -1.31764698 |
| C | 0.00000000  | -2.42007545 | -1.31764698 |
| O | 0.00000000  | 0.00000000  | 2.48269094  |
| H | 0.00000000  | 4.03690733  | -0.05185132 |
| H | 0.00000000  | -4.03690733 | -0.05185132 |
| H | 1.66061256  | 2.48420530  | -2.53995285 |
| H | -1.66061256 | 2.48420530  | -2.53995285 |
| H | 1.66061256  | -2.48420530 | -2.53995285 |
| H | -1.66061256 | -2.48420530 | -2.53995285 |

### S1.2 Acrolein

|   |             |             |            |
|---|-------------|-------------|------------|
| C | -1.11645072 | -0.68348783 | 0.00000000 |
| C | 1.20647847  | 0.83714564  | 0.00000000 |
| C | 3.46831059  | -0.28872636 | 0.00000000 |
| O | -3.23666415 | 0.19187203  | 0.00000000 |
| H | -0.80613858 | -2.74747338 | 0.00000000 |
| H | 0.98699813  | 2.86613511  | 0.00000000 |
| H | 5.20930864  | 0.77443560  | 0.00000000 |
| H | 3.60951559  | -2.33000749 | 0.00000000 |

### S1.3 Amonia

|   |             |             |             |
|---|-------------|-------------|-------------|
| N | 0.12804615  | -0.00000000 | 0.00000000  |
| H | -0.59303935 | 0.88580079  | -1.53425197 |
| H | -0.59303935 | -1.77160157 | -0.00000000 |
| H | -0.59303935 | 0.88580079  | 1.53425197  |

## S1.4 Benzene

|   |             |             |            |
|---|-------------|-------------|------------|
| C | 0.00000000  | 2.63144965  | 0.00000000 |
| C | -2.27890225 | 1.31572483  | 0.00000000 |
| C | -2.27890225 | -1.31572483 | 0.00000000 |
| C | 0.00000000  | -2.63144965 | 0.00000000 |
| C | 2.27890225  | -1.31572483 | 0.00000000 |
| C | 2.27890225  | 1.31572483  | 0.00000000 |
| H | -4.04725813 | 2.33668557  | 0.00000000 |
| H | -4.04725813 | -2.33668557 | 0.00000000 |
| H | -0.00000000 | -4.67337115 | 0.00000000 |
| H | 4.04725813  | -2.33668557 | 0.00000000 |
| H | 4.04725813  | 2.33668557  | 0.00000000 |
| H | 0.00000000  | 4.67337115  | 0.00000000 |

## S1.5 Butadiene

|   |             |            |             |
|---|-------------|------------|-------------|
| C | 1.14656244  | 0.00000000 | 0.75468820  |
| C | -1.14656244 | 0.00000000 | -0.75468820 |
| C | 3.48132647  | 0.00000000 | -0.22482805 |
| C | -3.48132647 | 0.00000000 | 0.22482805  |
| H | 0.90770978  | 0.00000000 | 2.78883925  |
| H | -0.90770978 | 0.00000000 | -2.78883925 |
| H | 3.77525814  | 0.00000000 | -2.24895470 |
| H | -3.77525814 | 0.00000000 | 2.24895470  |
| H | 5.13664967  | 0.00000000 | 0.96861890  |
| H | -5.13664967 | 0.00000000 | -0.96861890 |

## S1.6 Carbon monoxide

|   |              |              |               |
|---|--------------|--------------|---------------|
| C | 0.0000000000 | 0.0000000000 | -1.2494205467 |
| O | 0.0000000000 | 0.0000000000 | 0.8926669184  |

## S1.7 Cyclopentadiene

|   |             |             |             |
|---|-------------|-------------|-------------|
| C | 0.00000000  | 0.00000000  | -2.33113051 |
| C | 0.00000000  | 2.22209092  | -0.56871188 |
| C | 0.00000000  | -2.22209092 | -0.56871188 |
| C | 0.00000000  | 1.38514451  | 1.83772922  |
| C | 0.00000000  | -1.38514451 | 1.83772922  |
| H | 1.66130504  | 0.00000000  | -3.56414299 |
| H | -1.66130504 | 0.00000000  | -3.56414299 |
| H | 0.00000000  | 4.16550405  | -1.18116624 |
| H | 0.00000000  | -4.16550405 | -1.18116624 |
| H | 0.00000000  | 2.54514584  | 3.51352303  |
| H | 0.00000000  | -2.54514584 | 3.51352303  |

## S1.8 Cyclopropene

|   |               |               |               |
|---|---------------|---------------|---------------|
| C | 0.0000000000  | 0.0000000000  | -1.6682088006 |
| C | 0.0000000000  | 1.2252390588  | 0.9068141947  |
| C | 0.0000000000  | -1.2252390588 | 0.9068141947  |
| H | 1.7225544623  | 0.0000000000  | -2.7788114942 |
| H | -1.7225544623 | 0.0000000000  | -2.7788114942 |
| H | 0.0000000000  | 2.9784451947  | 1.9207677091  |
| H | 0.0000000000  | -2.9784451947 | 1.9207677091  |

## S1.9 Diazirine

|   |               |               |               |
|---|---------------|---------------|---------------|
| C | 0.0000000000  | 0.0000000000  | -0.2669609897 |
| H | 0.0000000000  | 1.7589089506  | -1.2861647760 |
| H | 0.0000000000  | -1.7589089506 | -1.2861647760 |
| N | 1.1605810005  | 0.0000000000  | 2.2718300657  |
| N | -1.1605810005 | 0.0000000000  | 2.2718300657  |

### S1.10 Diazomethane

|   |              |               |               |
|---|--------------|---------------|---------------|
| C | 0.0000000000 | 0.0000000000  | -2.3083000493 |
| N | 0.0000000000 | 0.0000000000  | 0.1445788951  |
| N | 0.0000000000 | 0.0000000000  | 2.2992321564  |
| H | 0.0000000000 | 1.7987520141  | -3.2427231720 |
| H | 0.0000000000 | -1.7987520141 | -3.2427231720 |

### S1.11 Dinitrogen

|   |              |              |               |
|---|--------------|--------------|---------------|
| N | 0.0000000000 | 0.0000000000 | 1.0400863228  |
| N | 0.0000000000 | 0.0000000000 | -1.0400863228 |

### S1.12 Ethylene

|   |              |               |               |
|---|--------------|---------------|---------------|
| C | 0.0000000000 | 1.2602658282  | 0.0000000000  |
| C | 0.0000000000 | -1.2602658282 | 0.0000000000  |
| H | 0.0000000000 | 2.3234597643  | 1.7428767216  |
| H | 0.0000000000 | 2.3234597643  | -1.7428767216 |
| H | 0.0000000000 | -2.3234597643 | 1.7428767216  |
| H | 0.0000000000 | -2.3234597643 | -1.7428767216 |

### S1.13 Formaldehyde

|   |              |               |               |
|---|--------------|---------------|---------------|
| C | 0.0000000000 | 0.0000000000  | -1.1394766614 |
| O | 0.0000000000 | 0.0000000000  | 1.1440288250  |
| H | 0.0000000000 | 1.7662762344  | -2.2339865296 |
| H | 0.0000000000 | -1.7662762344 | -2.2339865296 |

### S1.14 Furan

|   |            |             |             |
|---|------------|-------------|-------------|
| C | 0.00000000 | 2.06365826  | -0.60051250 |
| C | 0.00000000 | -2.06365826 | -0.60051250 |
| C | 0.00000000 | 1.35348578  | 1.86336416  |
| C | 0.00000000 | -1.35348578 | 1.86336416  |
| O | 0.00000000 | 0.00000000  | -2.13945332 |
| H | 0.00000000 | 3.86337287  | -1.53765695 |
| H | 0.00000000 | -3.86337287 | -1.53765695 |
| H | 0.00000000 | 2.59168789  | 3.47168051  |
| H | 0.00000000 | -2.59168789 | 3.47168051  |

### S1.15 Glyoxal

|   |             |             |            |
|---|-------------|-------------|------------|
| C | 1.21360282  | 0.75840215  | 0.00000000 |
| C | -1.21360282 | -0.75840215 | 0.00000000 |
| O | 3.25581408  | -0.26453186 | 0.00000000 |
| O | -3.25581408 | 0.26453186  | 0.00000000 |
| H | 0.96135276  | 2.81883243  | 0.00000000 |
| H | -0.96135276 | -2.81883243 | 0.00000000 |

### S1.16 Hexatriene

|   |             |             |             |
|---|-------------|-------------|-------------|
| C | 1.14024826  | 0.56596845  | -0.00000000 |
| C | -1.14024826 | -0.56596845 | -0.00000000 |
| C | 3.51540649  | -0.78907931 | 0.00000000  |
| C | -3.51540649 | 0.78907931  | 0.00000000  |
| C | 5.78668151  | 0.33754155  | -0.00000000 |
| C | -5.78668151 | -0.33754155 | -0.00000000 |
| H | 1.23448067  | 2.61584039  | 0.00000000  |
| H | -1.23448067 | -2.61584039 | 0.00000000  |
| H | 3.40773630  | -2.83459321 | 0.00000000  |
| H | -3.40773630 | 2.83459321  | 0.00000000  |
| H | 5.95047109  | 2.37626316  | -0.00000000 |
| H | -5.95047109 | -2.37626316 | -0.00000000 |
| H | 7.51470672  | -0.74809921 | 0.00000000  |
| H | -7.51470672 | 0.74809921  | 0.00000000  |



### S1.17 Ketene

|   |              |               |               |
|---|--------------|---------------|---------------|
| C | 0.0000000000 | 0.0000000000  | -2.4481015147 |
| C | 0.0000000000 | 0.0000000000  | 0.0349854474  |
| O | 0.0000000000 | 0.0000000000  | 2.2366391419  |
| H | 0.0000000000 | 1.7743207921  | -3.4370598798 |
| H | 0.0000000000 | -1.7743207921 | -3.4370598798 |

### S1.18 Methylenecyclopropene

|   |            |             |             |
|---|------------|-------------|-------------|
| C | 0.00000000 | 0.00000000  | 0.53512883  |
| C | 0.00000000 | 0.00000000  | 3.04739824  |
| C | 0.00000000 | 1.25042956  | -1.88571561 |
| C | 0.00000000 | -1.25042956 | -1.88571561 |
| H | 0.00000000 | 2.96887531  | -2.96270271 |
| H | 0.00000000 | -2.96887531 | -2.96270271 |
| H | 0.00000000 | 1.75335023  | 4.08608382  |
| H | 0.00000000 | -1.75335023 | 4.08608382  |

### S1.19 Pyrazine

|   |            |             |             |
|---|------------|-------------|-------------|
| C | 0.00000000 | 2.13188686  | 1.31510863  |
| C | 0.00000000 | -2.13188686 | 1.31510863  |
| C | 0.00000000 | 2.13188686  | -1.31510863 |
| C | 0.00000000 | -2.13188686 | -1.31510863 |
| N | 0.00000000 | 0.00000000  | 2.66620111  |
| N | 0.00000000 | 0.00000000  | -2.66620111 |
| H | 0.00000000 | 3.88751412  | 2.35234226  |
| H | 0.00000000 | -3.88751412 | 2.35234226  |
| H | 0.00000000 | 3.88751412  | -2.35234226 |
| H | 0.00000000 | -3.88751412 | -2.35234226 |

## S1.20 Pyridazine

|   |            |             |             |
|---|------------|-------------|-------------|
| C | 0.00000000 | 1.30150855  | -2.31552865 |
| C | 0.00000000 | -1.30150855 | -2.31552865 |
| C | 0.00000000 | 2.49271907  | 0.03513416  |
| C | 0.00000000 | -2.49271907 | 0.03513416  |
| N | 0.00000000 | 1.26228251  | 2.23104685  |
| N | 0.00000000 | -1.26228251 | 2.23104685  |
| H | 0.00000000 | 4.52804172  | 0.19299731  |
| H | 0.00000000 | -4.52804172 | 0.19299731  |
| H | 0.00000000 | 2.39011496  | -4.03967703 |
| H | 0.00000000 | -2.39011496 | -4.03967703 |

## S1.21 Pyridine

|   |            |             |             |
|---|------------|-------------|-------------|
| C | 0.00000000 | 0.00000000  | -2.66451139 |
| C | 0.00000000 | 2.25494985  | -1.32069889 |
| C | 0.00000000 | -2.25494985 | -1.32069889 |
| C | 0.00000000 | 2.15398594  | 1.30669632  |
| C | 0.00000000 | -2.15398594 | 1.30669632  |
| N | 0.00000000 | 0.00000000  | 2.62778932  |
| H | 0.00000000 | 0.00000000  | -4.70641516 |
| H | 0.00000000 | 4.05768507  | -2.27625442 |
| H | 0.00000000 | -4.05768507 | -2.27625442 |
| H | 0.00000000 | 3.88059079  | 2.40341581  |
| H | 0.00000000 | -3.88059079 | 2.40341581  |

## S1.22 Pyrimidine

|   |            |             |             |
|---|------------|-------------|-------------|
| C | 0.00000000 | 0.00000000  | 2.41518350  |
| C | 0.00000000 | -0.00000000 | -2.60410885 |
| C | 0.00000000 | 2.23272561  | -1.22869402 |
| C | 0.00000000 | -2.23272561 | -1.22869402 |
| N | 0.00000000 | 2.26214196  | 1.29619742  |
| N | 0.00000000 | -2.26214196 | 1.29619742  |
| H | 0.00000000 | 0.00000000  | 4.45780256  |
| H | 0.00000000 | 0.00000000  | -4.64120942 |
| H | 0.00000000 | 4.05149341  | -2.16351748 |
| H | 0.00000000 | -4.05149341 | -2.16351748 |

### S1.23 Pyrrole

|   |            |             |             |
|---|------------|-------------|-------------|
| C | 0.00000000 | 2.11924634  | 0.62676569  |
| C | 0.00000000 | -2.11924634 | 0.62676569  |
| C | 0.00000000 | 1.34568862  | -1.85506908 |
| C | 0.00000000 | -1.34568862 | -1.85506908 |
| N | 0.00000000 | 0.00000000  | 2.10934391  |
| H | 0.00000000 | 0.00000000  | 4.00257355  |
| H | 0.00000000 | 3.97648410  | 1.44830201  |
| H | 0.00000000 | -3.97648410 | 1.44830201  |
| H | 0.00000000 | 2.56726559  | -3.47837232 |
| H | 0.00000000 | -2.56726559 | -3.47837232 |

### S1.24 Silylidene

|    |              |               |               |
|----|--------------|---------------|---------------|
| C  | 0.0000000000 | 0.0000000000  | -2.0953992754 |
| Si | 0.0000000000 | 0.0000000000  | 1.1499292968  |
| H  | 0.0000000000 | 1.7092952389  | -3.2289448066 |
| H  | 0.0000000000 | -1.7092952389 | -3.2289448066 |

### S1.25 Tetrazine

|   |             |            |             |
|---|-------------|------------|-------------|
| C | 0.00000000  | 0.00000000 | 2.38208164  |
| C | 0.00000000  | 0.00000000 | -2.38208164 |
| N | 2.25673244  | 0.00000000 | 1.24973261  |
| N | -2.25673244 | 0.00000000 | 1.24973261  |
| N | 2.25673244  | 0.00000000 | -1.24973261 |
| N | -2.25673244 | 0.00000000 | -1.24973261 |
| H | 0.00000000  | 0.00000000 | 4.41850901  |
| H | 0.00000000  | 0.00000000 | -4.41850901 |

## S1.26 Thiophene

|   |            |             |             |
|---|------------|-------------|-------------|
| C | 0.00000000 | 2.33342542  | -0.09858421 |
| C | 0.00000000 | -2.33342542 | -0.09858421 |
| C | 0.00000000 | 1.34371718  | -2.48297725 |
| C | 0.00000000 | -1.34371718 | -2.48297725 |
| S | 0.00000000 | 0.00000000  | 2.17250692  |
| H | 0.00000000 | 4.29028016  | 0.44577296  |
| H | 0.00000000 | -4.29028016 | 0.44577296  |
| H | 0.00000000 | 2.48760051  | -4.16768392 |
| H | 0.00000000 | -2.48760051 | -4.16768392 |

## S1.27 Water

|   |              |               |               |
|---|--------------|---------------|---------------|
| O | 0.0000000000 | 0.0000000000  | -0.1320966888 |
| H | 0.0000000000 | 1.4315287786  | 0.9797000618  |
| H | 0.0000000000 | -1.4315287786 | 0.9797000618  |

## S2 Ground state absorption data

### S2.1 Small set of transitions, large basis sets

Table S1: Ground state absorption data for LR-CC3/dAVQZ and LR-CCSD/dAVQZ calculations.  $\Delta E_{0,n}$  [eV] and oscillator strengths in length, velocity, and mixed gauges,  $f^l$ ,  $f^v$ , and  $f^m$ , respectively. Rydberg = R, valence = V.

| Molecule        | State                                  | LR-CC3/dAVQZ     |       |       |       | LR-CCSD/dAVQZ    |       |       |       |
|-----------------|----------------------------------------|------------------|-------|-------|-------|------------------|-------|-------|-------|
|                 |                                        | $\Delta E_{0,n}$ | $f^l$ | $f^v$ | $f^m$ | $\Delta E_{0,n}$ | $f^l$ | $f^v$ | $f^m$ |
| Ammonia         | 1A <sub>2</sub> (R, n-3s)              | 6.611            | 0.084 | 0.086 | 0.085 | 6.651            | 0.082 | 0.085 | 0.084 |
|                 | 1E (R, n-3p)                           | 8.158            | 0.003 | 0.003 | 0.003 | 8.173            | 0.003 | 0.003 | 0.003 |
|                 | 2A <sub>1</sub> (R, n-3p)              | 8.606            | 0.000 | 0.000 | 0.000 | 8.620            | 0.000 | 0.000 | 0.000 |
|                 | 2A <sub>2</sub> (R, n-4s)              | 9.163            | 0.001 | 0.001 | 0.001 | 9.166            | 0.001 | 0.001 | 0.001 |
| Carbon monoxide | 2Σ <sup>+</sup> (R. n.d.)              | 10.720           | 0.007 | 0.007 | 0.007 | 11.010           | 0.011 | 0.010 | 0.011 |
|                 | 3Σ <sup>+</sup> (R. n.d.)              | 11.330           | 0.128 | 0.129 | 0.128 | 11.617           | 0.134 | 0.134 | 0.134 |
|                 | 1Π (V, n-π <sup>*</sup> )              | 8.470            | 0.084 | 0.086 | 0.085 | 8.572            | 0.080 | 0.075 | 0.078 |
|                 | 2Π (R, n.d.)                           | 11.457           | 0.034 | 0.033 | 0.033 | 11.749           | 0.037 | 0.037 | 0.037 |
| Diazirine       | 1B <sub>1</sub> (V, n-π <sup>*</sup> ) | 4.105            |       |       |       | 4.176            |       |       |       |
|                 | 1B <sub>2</sub> (R, n-3s)              | 7.476            |       |       |       | 7.594            |       |       |       |
|                 | 2A <sub>1</sub> (V, π-π <sup>*</sup> ) | 8.013            |       |       |       | 8.099            |       |       |       |
|                 | 1A <sub>2</sub> (V, π-π <sup>*</sup> ) | 2.162            | 0.000 | 0.000 | 0.000 | 2.301            | 0.000 | 0.000 | 0.000 |
| Silylidene      | 1B <sub>2</sub> (V, n-π <sup>*</sup> ) | 3.787            | 0.034 | 0.031 | 0.032 | 3.890            | 0.037 | 0.028 | 0.032 |
| Water           | 1A <sub>2</sub> (R, n-3p)              | 9.418            | 0.000 | 0.000 | 0.000 | 9.416            | 0.000 | 0.000 | 0.000 |
|                 | 1B <sub>1</sub> (R, n-3s)              | 7.650            | 0.052 | 0.053 | 0.053 | 7.659            | 0.051 | 0.055 | 0.053 |

Table S2: Ground state absorption data for LR-CC2/dAVQZ and LR-CC3/AVQZ calculations.

| Molecule        | State                     | LR-CC2/dAVQZ     |       |       |       | LR-CC3/AVQZ      |       |       |       |
|-----------------|---------------------------|------------------|-------|-------|-------|------------------|-------|-------|-------|
|                 |                           | $\Delta E_{0,n}$ | $f^l$ | $f^v$ | $f^m$ | $\Delta E_{0,n}$ | $f^l$ | $f^v$ | $f^m$ |
| Ammonia         | 1A <sub>2</sub> (R, n-3s) | 6.438            | 0.086 | 0.085 | 0.085 | 6.611            | 0.084 | 0.086 | 0.085 |
|                 | 1E (R, n-3p)              | 7.860            | 0.002 | 0.002 | 0.002 | 8.176            | 0.003 | 0.003 | 0.003 |
|                 | 2A <sub>1</sub> (R, n-3p) | 8.233            | 0.000 | 0.000 | 0.000 | 9.106            | 0.002 | 0.002 | 0.002 |
|                 | 2A <sub>2</sub> (R, n-4s) | 8.723            | 0.003 | 0.003 | 0.003 | 9.774            | 0.005 | 0.006 | 0.005 |
| Carbon monoxide | 2Σ <sup>+</sup> (R. n.d.) | 10.867           | 0.008 | 0.008 | 0.008 | 10.905           | 0.005 | 0.005 | 0.005 |
|                 | 3Σ <sup>+</sup> (R. n.d.) | 11.449           | 0.127 | 0.123 | 0.125 | 11.458           | 0.177 | 0.178 | 0.177 |
|                 | 1Π (V, n-π*)              | 8.617            | 0.080 | 0.068 | 0.074 | 8.472            | 0.084 | 0.086 | 0.085 |
|                 | 2Π (R, n.d.)              | 11.569           | 0.037 | 0.036 | 0.037 | 11.634           | 0.048 | 0.047 | 0.048 |
| Diazirine       | 1B <sub>1</sub> (V, n-π*) | 4.194            |       |       |       | 4.105            | 0.002 | 0.003 | 0.002 |
|                 | 1B <sub>2</sub> (R, n-3s) | 7.303            |       |       |       | 7.481            |       |       |       |
|                 | 2A <sub>1</sub> (V, π-π*) | 7.780            |       |       |       |                  |       |       |       |
| Silylidene      | 1A <sub>2</sub> (V, π-π*) | 2.373            | 0.000 | 0.000 | 0.000 | 2.161            | 0.000 | 0.000 | 0.000 |
|                 | 1B <sub>2</sub> (V, n-π*) | 3.857            | 0.037 | 0.021 | 0.028 | 3.788            | 0.034 | 0.031 | 0.032 |
| Water           | 1A <sub>2</sub> (R, n-3p) | 8.937            | 0.000 | 0.000 | 0.000 | 9.425            | 0.000 | 0.000 | 0.000 |
|                 | 1B <sub>1</sub> (R, n-3s) | 7.291            | 0.054 | 0.054 | 0.054 | 7.651            | 0.053 | 0.054 | 0.054 |

Table S3: Ground state absorption data for LR-CCSD/AVQZ and LR-CC2/AVQZ calculations.

| Molecule        | State                     | LR-CCSD/AVQZ     |       |       |       | LR-CC2/AVQZ      |       |       |       |
|-----------------|---------------------------|------------------|-------|-------|-------|------------------|-------|-------|-------|
|                 |                           | $\Delta E_{0,n}$ | $f^l$ | $f^v$ | $f^m$ | $\Delta E_{0,n}$ | $f^l$ | $f^v$ | $f^m$ |
| Ammonia         | 1A <sub>2</sub> (R, n-3s) | 6.651            | 0.083 | 0.086 | 0.084 | 6.439            | 0.086 | 0.085 | 0.086 |
|                 | 1E (R, n-3p)              | 8.192            | 0.003 | 0.003 | 0.003 | 7.891            | 0.003 | 0.002 | 0.003 |
|                 | 2A <sub>1</sub> (R, n-3p) | 9.132            | 0.002 | 0.002 | 0.002 | 8.828            | 0.001 | 0.001 | 0.001 |
|                 | 2A <sub>2</sub> (R, n-4s) | 9.791            | 0.005 | 0.007 | 0.006 | 9.468            | 0.010 | 0.011 | 0.010 |
| Carbon monoxide | 2Σ <sup>+</sup> (R, n.d.) | 11.190           | 0.010 | 0.009 | 0.009 | 11.070           | 0.006 | 0.007 | 0.006 |
|                 | 3Σ <sup>+</sup> (R, n.d.) | 11.733           | 0.183 | 0.182 | 0.183 | 11.599           | 0.185 | 0.180 | 0.183 |
|                 | 1Π (V, n-π*)              | 8.574            | 0.080 | 0.075 | 0.078 | 8.620            | 0.080 | 0.068 | 0.074 |
|                 | 2Π (R, n.d.)              | 11.916           | 0.051 | 0.051 | 0.051 | 11.772           | 0.053 | 0.054 | 0.054 |
|                 | 1B <sub>1</sub> (V, n-π*) | 4.177            | 0.002 | 0.002 | 0.002 | 4.195            | 0.002 | 0.002 | 0.002 |
| Diazirine       | 1B <sub>2</sub> (R, n-3s) | 7.600            |       |       |       | 7.313            |       |       |       |
|                 | 2A <sub>1</sub> (V, π-π*) | 8.138            | 0.127 | 0.113 | 0.120 | 7.832            | 0.125 | 0.110 | 0.117 |
| Silylidene      | 1A <sub>2</sub> (V, π-π*) | 2.301            | 0.000 | 0.000 | 0.000 | 2.373            | 0.000 | 0.000 | 0.000 |
|                 | 1B <sub>2</sub> (V, n-π*) | 3.891            | 0.037 | 0.028 | 0.032 | 3.858            | 0.037 | 0.021 | 0.028 |
| Water           | 1A <sub>2</sub> (R, n-3p) | 9.422            | 0.000 | 0.000 | 0.000 | 8.949            | 0.000 | 0.000 | 0.000 |
|                 | 1B <sub>1</sub> (R, n-3s) | 7.660            | 0.052 | 0.056 | 0.054 | 7.294            | 0.056 | 0.055 | 0.056 |



Table S4: Ground state absorption data for LR-CC3/tAVTZ and LR-CCSD/tAVTZ calculations.

| Molecule        | State                     | LR-CC3/tAVTZ     |       |       |       | LR-CCSD/tAVTZ    |       |       |       |
|-----------------|---------------------------|------------------|-------|-------|-------|------------------|-------|-------|-------|
|                 |                           | $\Delta E_{0,n}$ | $f^l$ | $f^v$ | $f^m$ | $\Delta E_{0,n}$ | $f^l$ | $f^v$ | $f^m$ |
| Ammonia         | 1A <sub>2</sub> (R, n-3s) | 6.572            | 0.084 | 0.087 | 0.085 | 6.600            | 0.082 | 0.086 | 0.084 |
|                 | 1E (R, n-3p)              | 8.117            | 0.003 | 0.003 | 0.003 | 8.119            | 0.003 | 0.003 | 0.003 |
|                 | 2A <sub>1</sub> (R, n-3p) | 8.560            | 0.000 | 0.000 | 0.000 | 8.560            | 0.000 | 0.000 | 0.000 |
|                 | 2A <sub>2</sub> (R, n-4s) | 9.117            | 0.000 | 0.000 | 0.000 | 9.105            | 0.000 | 0.000 | 0.000 |
| Carbon monoxide | 2Σ <sup>+</sup> (R. n.d.) | 10.675           | 0.006 | 0.006 | 0.006 | 10.960           | 0.010 | 0.009 | 0.010 |
|                 | 3Σ <sup>+</sup> (R. n.d.) | 11.282           | 0.128 | 0.128 | 0.128 | 11.564           | 0.134 | 0.134 | 0.134 |
|                 | 1Π (V, n-π*)              | 8.481            | 0.084 | 0.086 | 0.085 | 8.582            | 0.080 | 0.075 | 0.078 |
|                 | 2Π (R, n.d.)              | 11.412           | 0.033 | 0.033 | 0.033 | 11.698           | 0.037 | 0.036 | 0.037 |
| Diazirine       | 1B <sub>1</sub> (V, n-π*) | 4.112            | 0.002 | 0.003 | 0.002 | 4.183            | 0.002 | 0.002 | 0.002 |
|                 | 1B <sub>2</sub> (R, n-3s) | 7.442            |       |       |       | 7.544            |       |       |       |
| Silylidene      | 2A <sub>1</sub> (V, π-π*) | 7.972            | 0.114 | 0.114 | 0.114 | 8.047            | 0.113 | 0.101 | 0.107 |
|                 | 1A <sub>2</sub> (V, π-π*) | 2.155            | 0.000 | 0.000 | 0.000 | 2.287            | 0.000 | 0.000 | 0.000 |
| Water           | 1B <sub>2</sub> (V, n-π*) | 3.779            | 0.033 | 0.030 | 0.032 | 3.877            | 0.036 | 0.027 | 0.031 |
|                 | 1A <sub>2</sub> (R, n-3p) | 9.367            | 0.000 | 0.000 | 0.000 | 9.347            | 0.000 | 0.000 | 0.000 |
|                 | 1B <sub>1</sub> (R, n-3s) | 7.599            | 0.052 | 0.054 | 0.053 | 7.592            | 0.051 | 0.055 | 0.053 |

Table S5: Ground state absorption data for LR-CC2/tAVTZ and LR-CC3/tAVDZ calculations.

| Molecule        | State                                  | LR-CC2/tAVTZ     |       |       |       | LR-CC3/tAVDZ     |       |       |       |
|-----------------|----------------------------------------|------------------|-------|-------|-------|------------------|-------|-------|-------|
|                 |                                        | $\Delta E_{0,n}$ | $f^l$ | $f^v$ | $f^m$ | $\Delta E_{0,n}$ | $f^l$ | $f^v$ | $f^m$ |
| Ammonia         | 1A <sub>2</sub> (R, n-3s)              | 6.384            | 0.086 | 0.086 | 0.086 | 6.457            | 0.085 | 0.088 | 0.087 |
|                 | 1E (R, n-3p)                           | 7.800            | 0.002 | 0.002 | 0.002 | 7.993            | 0.003 | 0.003 | 0.003 |
|                 | 2A <sub>1</sub> (R, n-3p)              | 8.164            | 0.000 | 0.000 | 0.000 | 8.427            | 0.000 | 0.000 | 0.000 |
|                 | 2A <sub>2</sub> (R, n-4s)              | 8.657            | 0.002 | 0.002 | 0.002 | 8.981            | 0.000 | 0.001 | 0.000 |
| Carbon monoxide | 2Σ <sup>+</sup> (R. n.d.)              | 10.812           | 0.007 | 0.008 | 0.008 | 10.532           | 0.006 | 0.005 | 0.006 |
|                 | 3Σ <sup>+</sup> (R. n.d.)              | 11.391           | 0.127 | 0.123 | 0.125 | 11.129           | 0.126 | 0.125 | 0.125 |
|                 | 1Π (V, n-π <sup>*</sup> )              | 8.633            | 0.081 | 0.068 | 0.074 | 8.561            | 0.088 | 0.091 | 0.090 |
|                 | 2Π (R, n.d.)                           | 11.513           | 0.036 | 0.036 | 0.036 | 11.269           | 0.030 | 0.028 | 0.029 |
|                 | 1B <sub>1</sub> (V, n-π <sup>*</sup> ) | 4.203            | 0.002 | 0.002 | 0.002 | 4.162            | 0.002 | 0.004 | 0.003 |
| Diazirine       | 1B <sub>2</sub> (R, n-3s)              | 7.241            |       |       |       | 7.335            |       |       |       |
|                 | 2A <sub>1</sub> (V, π-π <sup>*</sup> ) | 7.720            | 0.107 | 0.094 | 0.100 | 7.846            | 0.106 | 0.103 | 0.105 |
| Silylidene      | 1A <sub>2</sub> (V, π-π <sup>*</sup> ) | 2.366            | 0.000 | 0.000 | 0.000 | 2.179            | 0.000 | 0.000 | 0.000 |
|                 | 1B <sub>2</sub> (V, n-π <sup>*</sup> ) | 3.851            | 0.037 | 0.020 | 0.028 | 3.801            | 0.034 | 0.030 | 0.032 |
| Water           | 1A <sub>2</sub> (R, n-3p)              | 8.867            | 0.000 | 0.000 | 0.000 | 9.257            | 0.000 | 0.000 | 0.000 |
|                 | 1B <sub>1</sub> (R, n-3s)              | 7.226            | 0.054 | 0.054 | 0.054 | 7.492            | 0.053 | 0.055 | 0.054 |

Table S6: Ground state absorption data for LR-CCSD/tAVDZ and LR-CC2/tAVDZ calculations.

| Molecule        | State                     | LR-CCSD/tAVDZ    |       |       |       | LR-CC2/tAVDZ     |       |       |       |
|-----------------|---------------------------|------------------|-------|-------|-------|------------------|-------|-------|-------|
|                 |                           | $\Delta E_{0,n}$ | $f^l$ | $f^v$ | $f^m$ | $\Delta E_{0,n}$ | $f^l$ | $f^v$ | $f^m$ |
| Ammonia         | 1A <sub>2</sub> (R, n-3s) | 6.446            | 0.083 | 0.088 | 0.086 | 6.236            | 0.086 | 0.088 | 0.087 |
|                 | 1E (R, n-3p)              | 7.954            | 0.002 | 0.002 | 0.002 | 7.634            | 0.002 | 0.002 | 0.002 |
|                 | 2A <sub>1</sub> (R, n-3p) | 8.386            | 0.000 | 0.000 | 0.000 | 7.993            | 0.000 | 0.000 | 0.000 |
|                 | 2A <sub>2</sub> (R, n-4s) | 8.928            | 0.001 | 0.001 | 0.001 | 8.482            | 0.003 | 0.003 | 0.003 |
| Carbon monoxide | 2Σ <sup>+</sup> (R. n.d.) | 10.794           | 0.009 | 0.008 | 0.008 | 10.670           | 0.006 | 0.007 | 0.007 |
|                 | 3Σ <sup>+</sup> (R. n.d.) | 11.388           | 0.133 | 0.131 | 0.132 | 11.237           | 0.125 | 0.120 | 0.122 |
|                 | 1Π (V, n-π*)              | 8.660            | 0.084 | 0.080 | 0.082 | 8.713            | 0.085 | 0.072 | 0.078 |
|                 | 2Π (R, n.d.)              | 11.531           | 0.034 | 0.033 | 0.034 | 11.366           | 0.033 | 0.032 | 0.033 |
| Diazirine       | 1B <sub>1</sub> (V, n-π*) | 4.236            | 0.002 | 0.004 | 0.003 | 4.252            | 0.002 | 0.003 | 0.003 |
|                 | 1B <sub>2</sub> (R, n-3s) | 7.391            |       |       |       | 7.077            |       |       |       |
| Silylidene      | 2A <sub>1</sub> (V, π-π*) | 7.885            | 0.104 | 0.092 | 0.098 | 7.557            | 0.098 | 0.085 | 0.091 |
|                 | 1A <sub>2</sub> (V, π-π*) | 2.289            | 0.000 | 0.000 | 0.000 | 2.379            | 0.000 | 0.000 | 0.000 |
| Water           | 1B <sub>2</sub> (V, n-π*) | 3.875            | 0.036 | 0.027 | 0.031 | 3.856            | 0.038 | 0.020 | 0.028 |
|                 | 1A <sub>2</sub> (R, n-3p) | 9.178            | 0.000 | 0.000 | 0.000 | 8.693            | 0.000 | 0.000 | 0.000 |
|                 | 1B <sub>1</sub> (R, n-3s) | 7.428            | 0.052 | 0.057 | 0.054 | 7.066            | 0.055 | 0.056 | 0.055 |

**S2.2 Full testing set, LR-CC3, LR-CCSD, LR-CC2, with AVDZ, dAVDZ, AVTZ, and dAVTZ basis sets**

Table S7: Ground state absorption data for LR-CC3/AVDZ and LR-CCSD/AVDZ calculations.  $\Delta E_{0,n}$  [eV] and oscillator strengths in length, velocity, and mixed gauges,  $f^l$ ,  $f^v$ , and  $f^m$ , respectively. Rydberg = R, valence = V.

| Molecule        | State                                 | LR-CC3/AVDZ      |       |       |       |                  | LR-CCSD/AVDZ |        |       |       |       |
|-----------------|---------------------------------------|------------------|-------|-------|-------|------------------|--------------|--------|-------|-------|-------|
|                 |                                       | $\Delta E_{0,n}$ | $f^l$ | $f^v$ | $f^m$ | $\Delta E_{0,n}$ | $f^l$        | $f^v$  | $f^m$ | $f^l$ | $f^m$ |
| Acetone         | 2A <sub>1</sub> (R, n-3p)             | 7.388            | 0.000 | 0.000 | 0.000 | 7.460            | 0.000        | -0.000 | 0.000 | 0.000 | 0.000 |
|                 | 1B <sub>2</sub> (R, n-3s)             | 6.306            | 0.030 | 0.031 | 0.031 | 6.395            | 0.031        | 0.034  | 0.032 | 0.034 | 0.032 |
|                 | 2B <sub>2</sub> (R, n-3p)             | 7.560            | 0.008 | 0.009 | 0.008 | 7.594            | 0.007        | 0.007  | 0.007 | 0.007 | 0.007 |
|                 | 2A <sub>2</sub> (R, n-3p)             | 7.370            | 0.000 | 0.000 | 0.000 | 7.425            | 0.000        | 0.000  | 0.000 | 0.000 | 0.000 |
| Acrolein        | 1A'' (V, n- $\pi^*$ )                 | 3.767            | 0.000 | 0.000 | 0.000 | 3.906            | 0.000        | 0.001  | 0.000 | 0.000 | 0.000 |
|                 | 2A'' (V, n- $\pi^*$ )                 | 6.754            | 0.000 | 0.000 | 0.000 | 7.200            | 0.000        | -0.000 | 0.000 | 0.000 | 0.000 |
| Ammonia         | 1A <sub>2</sub> (R, n-3s)             | 6.464            | 0.090 | 0.089 | 0.089 | 6.455            | 0.088        | 0.089  | 0.089 | 0.089 | 0.089 |
|                 | 1E (R, n-3p)                          | 8.061            | 0.004 | 0.003 | 0.003 | 8.024            | 0.003        | 0.003  | 0.003 | 0.003 | 0.003 |
|                 | 2A <sub>1</sub> (R, n-3p)             | 9.664            | 0.003 | 0.002 | 0.003 | 9.649            | 0.003        | 0.002  | 0.003 | 0.002 | 0.003 |
|                 | 2A <sub>2</sub> (R, n-4s)             | 10.396           | 0.018 | 0.027 | 0.022 | 10.376           | 0.020        | 0.029  | 0.025 | 0.020 | 0.025 |
| Benzene         | 1E <sub>1g</sub> (R, $\pi$ -3s)       | 6.456            | 0.000 | 0.000 | 0.000 | 6.485            | 0.000        | 0.000  | 0.000 | 0.000 | 0.000 |
|                 | 1E <sub>2u</sub> (R, $\pi$ -3p)       | 7.087            | 0.000 | 0.000 | 0.000 | 7.108            | 0.000        | 0.000  | 0.000 | 0.000 | 0.000 |
|                 | 1A <sub>2u</sub> (R, $\pi$ -3p)       | 7.020            | 0.070 | 0.069 | 0.070 | 7.030            | 0.070        | 0.067  | 0.069 | 0.070 | 0.069 |
| Butadiene       | 1B <sub>g</sub> (R, $\pi$ -3s)        | 6.252            | 0.673 | 0.619 | 0.645 | 6.370            | 0.703        | 0.556  | 0.625 | 0.703 | 0.625 |
|                 | 2B <sub>g</sub> (R, $\pi$ -3d)        | 7.512            | 0.000 | 0.000 | 0.000 | 7.552            | 0.000        | 0.000  | 0.000 | 0.000 | 0.000 |
|                 | 1A <sub>u</sub> (R, $\pi$ -3p)        | 6.574            | 0.001 | 0.001 | 0.001 | 6.619            | 0.001        | 0.001  | 0.001 | 0.001 | 0.001 |
|                 | 2A <sub>u</sub> (R, $\pi$ -3p)        | 6.731            | 0.053 | 0.052 | 0.053 | 6.780            | 0.054        | 0.052  | 0.053 | 0.054 | 0.053 |
| Carbon monoxide | 2 $\Sigma^+$ (R, n.d.)                | 10.917           | 0.001 | 0.000 | 0.000 | 11.171           | 0.003        | 0.002  | 0.002 | 0.003 | 0.002 |
|                 | 3 $\Sigma^+$ (R, n.d.)                | 11.483           | 0.237 | 0.231 | 0.234 | 11.710           | 0.248        | 0.238  | 0.243 | 0.248 | 0.243 |
|                 | 1 $\Pi$ (V, n- $\pi^*$ )              | 8.572            | 0.088 | 0.092 | 0.090 | 8.671            | 0.084        | 0.081  | 0.083 | 0.084 | 0.083 |
|                 | 2 $\Pi$ (R, n.d.)                     | 11.737           | 0.061 | 0.058 | 0.059 | 11.973           | 0.066        | 0.063  | 0.064 | 0.066 | 0.063 |
| Cyclopentadiene | 2A <sub>1</sub> (V, $\pi$ - $\pi^*$ ) | 6.595            | 0.001 | 0.001 | 0.001 | 6.949            | 0.001        | 0.000  | 0.001 | 0.001 | 0.001 |

| Molecule     | State                                 | LR-CC3/AVDZ      |       |       |       | LR-CCSD/AVDZ     |       |       |       |
|--------------|---------------------------------------|------------------|-------|-------|-------|------------------|-------|-------|-------|
|              |                                       | $\Delta E_{0,n}$ | $f^l$ | $f^v$ | $f^m$ | $\Delta E_{0,n}$ | $f^l$ | $f^v$ | $f^m$ |
| Cyclopropene | 1A <sub>2</sub> (R, $\pi$ -3s)        | 5.705            | 0.000 | 0.000 | 0.000 | 5.737            | 0.000 | 0.000 | 0.000 |
|              | 2A <sub>2</sub> (R, $\pi$ -3p)        | 6.390            | 0.000 | 0.000 | 0.000 | 6.415            | 0.000 | 0.000 | 0.000 |
|              | 1B <sub>1</sub> (R, $\pi$ -3p)        | 6.342            | 0.041 | 0.039 | 0.040 | 6.358            | 0.041 | 0.038 | 0.039 |
|              | 1B <sub>2</sub> (V, $\pi$ - $\pi^*$ ) | 5.588            | 0.087 | 0.081 | 0.084 | 5.708            | 0.091 | 0.056 | 0.072 |
|              | 2B <sub>2</sub> (R, $\pi$ -3p)        | 6.550            | 0.051 | 0.046 | 0.048 | 6.576            | 0.050 | 0.044 | 0.047 |
|              | 2B <sub>1</sub> (R, $\pi$ -3s)        | 6.864            | 0.008 | 0.007 | 0.007 | 6.890            | 0.008 | 0.006 | 0.007 |
|              | 3B <sub>1</sub> (R, $\pi$ -3p)        | 7.261            | 0.030 | 0.031 | 0.030 | 7.293            | 0.030 | 0.033 | 0.031 |
|              | 1B <sub>1</sub> (V, n- $\pi^*$ )      | 4.164            | 0.002 | 0.004 | 0.003 | 4.238            | 0.002 | 0.004 | 0.003 |
| Diazirine    | 1B <sub>2</sub> (R, n-3s)             | 7.361            | 0.000 | 0.001 | 0.000 | 7.421            | 0.001 | 0.002 | 0.001 |
| Diazomethane | 2A <sub>1</sub> (V, $\pi$ - $\pi^*$ ) | 7.972            | 0.138 | 0.134 | 0.136 | 8.017            | 0.137 | 0.121 | 0.129 |
|              | 1B <sub>1</sub> (R, $\pi$ -3s)        | 5.323            | 0.017 | 0.017 | 0.017 | 5.423            | 0.018 | 0.017 | 0.017 |
|              | 1A <sub>2</sub> (V, $\pi$ - $\pi^*$ ) | 3.102            | 0.000 | 0.000 | 0.000 | 3.227            | 0.000 | 0.000 | 0.000 |
| Formaldehyde | 2A <sub>1</sub> (R, n-3p)             | 8.081            | 0.057 | 0.053 | 0.055 | 8.052            | 0.058 | 0.057 | 0.058 |
|              | 1B <sub>2</sub> (R, n-3s)             | 7.051            | 0.021 | 0.020 | 0.021 | 7.043            | 0.018 | 0.017 | 0.017 |
|              | 2B <sub>2</sub> (R, n-3p)             | 8.017            | 0.041 | 0.041 | 0.041 | 7.993            | 0.044 | 0.046 | 0.045 |
|              | 1A <sub>2</sub> (V, n- $\pi^*$ )      | 4.004            | 0.000 | 0.000 | 0.000 | 4.020            | 0.000 | 0.000 | 0.000 |
| Furane       | 2A <sub>2</sub> (R, n-3p)             | 8.655            | 0.000 | 0.000 | 0.000 | 8.614            | 0.000 | 0.000 | 0.000 |
|              | 1B <sub>1</sub> (R, $\pi$ -3p)        | 6.554            | 0.042 | 0.041 | 0.041 | 6.604            | 0.043 | 0.041 | 0.042 |
|              | 2B <sub>2</sub> (R, $\pi$ -3p)        | 7.392            | 0.011 | 0.010 | 0.010 | 7.466            | 0.009 | 0.013 | 0.011 |
| Glyoxal      | 1A <sub>2</sub> (R, $\pi$ -3s)        | 5.999            | 0.000 | 0.000 | 0.000 | 6.064            | 0.000 | 0.000 | 0.000 |
|              | 2A <sub>2</sub> (R, $\pi$ -3p)        | 6.732            | 0.000 | 0.000 | 0.000 | 6.795            | 0.000 | 0.000 | 0.000 |
|              | 1A <sub>u</sub> (V, n- $\pi^*$ )      | 2.900            | 0.000 | 0.000 | 0.000 | 3.010            | 0.000 | 0.001 | 0.001 |
|              | 1B <sub>g</sub> (V, n- $\pi^*$ )      | 4.300            | 0.000 | 0.000 | 0.000 | 4.421            | 0.000 | 0.000 | 0.000 |
| Ketene       | 2B <sub>g</sub> (V, n- $\pi^*$ )      | 6.588            | 0.000 | 0.000 | 0.000 | 7.067            | 0.000 | 0.000 | 0.000 |
|              | 2A <sub>1</sub> (V, $\pi$ - $\pi^*$ ) | 7.242            | 0.167 | 0.152 | 0.159 | 7.336            | 0.181 | 0.149 | 0.164 |
|              | 1B <sub>1</sub> (R, $\pi$ -3s)        | 5.832            | 0.036 | 0.034 | 0.035 | 5.938            | 0.035 | 0.031 | 0.033 |

| Molecule              | State                                  | LR-CC3/AVDZ      |       |       |       | LR-CCSD/AVDZ     |       |       |       |
|-----------------------|----------------------------------------|------------------|-------|-------|-------|------------------|-------|-------|-------|
|                       |                                        | $\Delta E_{0,n}$ | $f^l$ | $f^v$ | $f^m$ | $\Delta E_{0,n}$ | $f^l$ | $f^v$ | $f^m$ |
| Methylenecyclopropene | 2A <sub>2</sub> (R, $\pi$ -3p)         | 7.049            | 0.000 | 0.000 | 0.000 | 7.148            | 0.000 | 0.000 | 0.000 |
|                       | 1B <sub>1</sub> (R, $\pi$ -3s)         | 5.353            | 0.005 | 0.004 | 0.004 | 5.368            | 0.005 | 0.005 | 0.005 |
|                       | 1B <sub>2</sub> (V, $\pi$ - $\pi^*$ )  | 4.321            | 0.011 | 0.010 | 0.011 | 4.553            | 0.013 | 0.005 | 0.008 |
|                       | 1A <sub>2</sub> (R, $\pi$ -3p)         | 5.876            | 0.000 | 0.000 | 0.000 | 5.895            | 0.000 | 0.000 | 0.000 |
| Pyrazine              | 2A <sub>g</sub> (R, n-3s)              | 6.541            | 0.000 | 0.000 | 0.000 | 6.662            | 0.000 | 0.000 | 0.000 |
|                       | 1B <sub>1u</sub> (V, $\pi$ - $\pi^*$ ) | 6.925            | 0.062 | 0.059 | 0.060 | 7.017            | 0.057 | 0.043 | 0.050 |
|                       | 2B <sub>1u</sub> (R, n-3p)             | 7.378            | 0.108 | 0.104 | 0.106 | 7.469            | 0.114 | 0.095 | 0.104 |
|                       | 2B <sub>2u</sub> (R, n-3p)             | 7.139            | 0.040 | 0.038 | 0.039 | 7.270            | 0.040 | 0.039 | 0.039 |
| Pyridazine            | 1B <sub>3g</sub> (R, n.d.)             | 7.906            | 0.000 | 0.000 | 0.000 | 8.005            | 0.000 | 0.000 | 0.000 |
|                       | 2B <sub>1</sub> (V, n- $\pi^*$ )       | 6.412            | 0.004 | 0.006 | 0.005 | 6.665            | 0.005 | 0.006 | 0.005 |
|                       | 1A <sub>2</sub> (V, n- $\pi^*$ )       | 4.394            | 0.000 | 0.000 | 0.000 | 4.628            | 0.000 | 0.000 | 0.000 |
|                       | 1B <sub>1</sub> (R, mixed)             | 5.888            | 0.013 | 0.011 | 0.012 | 5.910            | 0.013 | 0.010 | 0.011 |
| Pyrrole               | 1A <sub>2</sub> (R, $\pi$ -3s)         | 5.149            | 0.000 | 0.000 | 0.000 | 5.221            | 0.000 | 0.000 | 0.000 |
|                       | 2A <sub>2</sub> (R, $\pi$ -3p)         | 5.940            | 0.000 | 0.000 | 0.000 | 5.987            | 0.000 | 0.000 | 0.000 |
|                       | 1A <sub>2</sub> (V, $\pi$ - $\pi^*$ )  | 2.179            | 0.000 | 0.000 | 0.000 | 2.289            | 0.000 | 0.000 | 0.000 |
|                       | 1B <sub>2</sub> (V, n- $\pi^*$ )       | 3.802            | 0.034 | 0.030 | 0.032 | 3.875            | 0.036 | 0.027 | 0.031 |
| Tetrazine             | 1B <sub>2g</sub> (V, n- $\pi^*$ )      | 5.533            | 0.000 | 0.000 | 0.000 | 5.880            | 0.000 | 0.000 | 0.000 |
|                       | 1B <sub>1g</sub> (V, n- $\pi^*$ )      | 4.966            | 0.000 | 0.000 | 0.000 | 5.302            | 0.000 | 0.000 | 0.000 |
|                       | 1B <sub>3u</sub> (V, n- $\pi^*$ )      | 2.488            | 0.006 | 0.012 | 0.009 | 2.650            | 0.007 | 0.009 | 0.008 |
|                       | 1A <sub>2</sub> (R, $\pi$ -3s)         | 6.070            | 0.000 | 0.000 | 0.000 | 6.124            | 0.000 | 0.000 | 0.000 |
| Thiophene             | 1B <sub>1</sub> (R, $\pi$ -3p)         | 6.189            | 0.015 | 0.015 | 0.015 | 6.306            | 0.018 | 0.018 | 0.018 |
|                       | 1A <sub>2</sub> (R, n-3p)              | 9.293            | 0.000 | 0.000 | 0.000 | 9.213            | 0.000 | 0.000 | 0.000 |
|                       | 1B <sub>1</sub> (R, n-3s)              | 7.511            | 0.058 | 0.059 | 0.059 | 7.447            | 0.057 | 0.061 | 0.059 |
|                       |                                        |                  |       |       |       |                  |       |       |       |

Table S8: Ground state absorption data for LR-CC2/AVDZ and LR-CC3/dAVDZ calculations.

| Molecule        | State                                 | LR-CC2/AVDZ      |       |       |       | LR-CC3/dAVDZ     |       |       |       |
|-----------------|---------------------------------------|------------------|-------|-------|-------|------------------|-------|-------|-------|
|                 |                                       | $\Delta E_{0,n}$ | $f^l$ | $f^v$ | $f^m$ | $\Delta E_{0,n}$ | $f^l$ | $f^v$ | $f^m$ |
| Acetone         | 2A <sub>1</sub> (R, n-3p)             | 6.753            | 0.003 | 0.003 | 0.003 | 7.307            |       |       |       |
|                 | 1B <sub>2</sub> (R, n-3s)             | 5.747            | 0.031 | 0.031 | 0.031 | 6.282            |       |       |       |
|                 | 2B <sub>2</sub> (R, n-3p)             | 6.959            | 0.011 | 0.011 | 0.011 | 7.307            |       |       |       |
|                 | 2A <sub>2</sub> (R, n-3p)             | 6.726            | 0.000 | 0.000 | 0.000 | 7.237            |       |       |       |
| Acrolein        | 1A'' (V, n- $\pi^*$ )                 | 3.873            | 0.000 | 0.000 | 0.000 | 3.761            |       |       |       |
|                 | 2A'' (V, n- $\pi^*$ )                 | 6.654            | 0.000 | 0.000 | 0.000 | 6.731            |       |       |       |
| Ammonia         | 1A <sub>2</sub> (R, n-3s)             | 6.249            | 0.091 | 0.088 | 0.089 | 6.457            | 0.085 | 0.088 | 0.087 |
|                 | 1E (R, n-3p)                          | 7.733            | 0.003 | 0.003 | 0.003 | 7.993            | 0.003 | 0.003 | 0.003 |
|                 | 2A <sub>1</sub> (R, n-3p)             | 9.400            | 0.001 | 0.001 | 0.001 | 8.436            | 0.000 | 0.000 | 0.000 |
| Benzene         | 2A <sub>2</sub> (R, n-4s)             | 10.148           | 0.028 | 0.036 | 0.032 | 8.988            | 0.001 | 0.002 | 0.001 |
|                 | 1E <sub>1g</sub> (R, $\pi$ -3s)       | 6.356            | 0.000 | 0.000 | 0.000 | 6.419            |       |       |       |
|                 | 1E <sub>2u</sub> (R, $\pi$ -3p)       | 6.953            | 0.000 | 0.000 | 0.000 | 7.025            |       |       |       |
| Butadiene       | 1A <sub>2u</sub> (R, $\pi$ -3p)       | 6.889            | 0.069 | 0.069 | 0.069 | 6.963            |       |       |       |
|                 | 1B <sub>g</sub> (R, $\pi$ -3s)        | 6.167            | 0.745 | 0.559 | 0.648 | 6.215            |       |       |       |
|                 | 2B <sub>g</sub> (R, $\pi$ -3d)        | 7.350            | 0.000 | 0.000 | 0.000 | 7.347            |       |       |       |
|                 | 1A <sub>u</sub> (R, $\pi$ -3p)        | 6.450            | 0.001 | 0.001 | 0.001 | 6.534            |       |       |       |
| Carbon monoxide | 2A <sub>u</sub> (R, $\pi$ -3p)        | 6.580            | 0.054 | 0.053 | 0.053 | 6.686            |       |       |       |
|                 | 2 $\Sigma^+$ (R, n.d.)                | 11.089           | 0.001 | 0.001 | 0.001 | 10.533           | 0.006 | 0.005 | 0.005 |
|                 | 3 $\Sigma^+$ (R, n.d.)                | 11.628           | 0.250 | 0.238 | 0.244 | 11.135           | 0.127 | 0.125 | 0.126 |
|                 | 1 $\Pi$ (V, n- $\pi^*$ )              | 8.724            | 0.085 | 0.073 | 0.079 | 8.563            | 0.088 | 0.091 | 0.090 |
| Cyclopentadiene | 2 $\Pi$ (R, n.d.)                     | 11.878           | 0.068 | 0.066 | 0.067 | 11.273           | 0.029 | 0.028 | 0.029 |
|                 | 2A <sub>1</sub> (V, $\pi$ - $\pi^*$ ) | 6.891            | 0.001 | 0.000 | 0.000 | 6.585            |       |       |       |
|                 | 1A <sub>2</sub> (R, $\pi$ -3s)        | 5.535            | 0.000 | 0.000 | 0.000 | 5.671            |       |       |       |



| Molecule     | State                                 | LR-CC2/AVDZ      |       |       |       | LR-CC3/dAVDZ     |       |       |       |
|--------------|---------------------------------------|------------------|-------|-------|-------|------------------|-------|-------|-------|
|              |                                       | $\Delta E_{0,n}$ | $f^l$ | $f^v$ | $f^m$ | $\Delta E_{0,n}$ | $f^l$ | $f^v$ | $f^m$ |
| Cyclopropene | 2A <sub>2</sub> (R, $\pi$ -3p)        | 6.189            | 0.000 | 0.000 | 0.000 | 6.318            |       |       |       |
|              | 1B <sub>1</sub> (R, $\pi$ -3p)        | 6.135            | 0.041 | 0.040 | 0.040 | 6.281            |       |       |       |
|              | 1B <sub>2</sub> (V, $\pi$ - $\pi^*$ ) | 5.548            | 0.103 | 0.082 | 0.092 | 5.581            |       |       |       |
|              | 2B <sub>2</sub> (R, $\pi$ -3p)        | 6.361            | 0.051 | 0.044 | 0.047 | 6.353            |       |       |       |
|              | 2B <sub>1</sub> (R, $\pi$ -3s)        | 6.763            | 0.006 | 0.005 | 0.006 | 6.831            |       |       |       |
|              | 3B <sub>1</sub> (R, $\pi$ -3p)        | 7.117            | 0.031 | 0.032 | 0.031 | 7.208            |       |       |       |
| Diazirine    | 1B <sub>1</sub> (V, $\pi$ - $\pi^*$ ) | 4.254            | 0.002 | 0.003 | 0.003 | 4.162            | 0.002 | 0.004 | 0.003 |
|              | 1B <sub>2</sub> (R, $\pi$ -3s)        | 7.117            | 0.002 | 0.004 | 0.003 | 7.335            |       |       |       |
| Diazomethane | 2A <sub>1</sub> (V, $\pi$ - $\pi^*$ ) | 7.723            | 0.138 | 0.119 | 0.129 | 7.846            | 0.106 | 0.103 | 0.105 |
|              | 1B <sub>1</sub> (R, $\pi$ -3s)        | 5.378            | 0.021 | 0.020 | 0.020 | 5.289            |       |       |       |
| Formaldehyde | 1A <sub>2</sub> (V, $\pi$ - $\pi^*$ ) | 3.407            | 0.000 | 0.000 | 0.000 | 3.103            |       |       |       |
|              | 2A <sub>1</sub> (R, $\pi$ -3p)        | 7.384            | 0.060 | 0.057 | 0.059 | 7.998            |       |       |       |
|              | 1B <sub>2</sub> (R, $\pi$ -3s)        | 6.397            | 0.022 | 0.019 | 0.021 | 7.036            |       |       |       |
|              | 2B <sub>2</sub> (R, $\pi$ -3p)        | 7.477            | 0.036 | 0.036 | 0.036 | 7.862            |       |       |       |
| Furane       | 1A <sub>2</sub> (V, $\pi$ - $\pi^*$ ) | 4.092            | 0.000 | 0.000 | 0.000 | 3.996            |       |       |       |
|              | 2A <sub>2</sub> (R, $\pi$ -3p)        | 8.061            | 0.000 | 0.000 | 0.000 | 8.235            |       |       |       |
|              | 1B <sub>1</sub> (R, $\pi$ -3p)        | 6.458            | 0.042 | 0.042 | 0.042 | 6.498            |       |       |       |
|              | 2B <sub>2</sub> (R, $\pi$ -3p)        | 7.390            | 0.007 | 0.006 | 0.007 | 6.800            |       |       |       |
|              | 1A <sub>2</sub> (R, $\pi$ -3s)        | 5.929            | 0.000 | 0.000 | 0.000 | 5.957            |       |       |       |
|              | 2A <sub>2</sub> (R, $\pi$ -3p)        | 6.634            | 0.000 | 0.000 | 0.000 | 6.643            |       |       |       |
| Glyoxal      | 1A <sub>u</sub> (V, $\pi$ - $\pi^*$ ) | 2.929            | 0.000 | 0.001 | 0.000 | 2.895            |       |       |       |
|              | 1B <sub>g</sub> (V, $\pi$ - $\pi^*$ ) | 4.462            | 0.000 | 0.000 | 0.000 | 4.294            |       |       |       |
|              | 2B <sub>g</sub> (V, $\pi$ - $\pi^*$ ) | 6.516            | 0.000 | 0.000 | 0.000 | 6.556            |       |       |       |
| Ketene       | 2A <sub>1</sub> (V, $\pi$ - $\pi^*$ ) | 7.267            | 0.191 | 0.161 | 0.175 | 6.964            |       |       |       |
|              | 1B <sub>1</sub> (R, $\pi$ -3s)        | 5.786            | 0.036 | 0.032 | 0.034 | 5.809            |       |       |       |
|              | 2A <sub>2</sub> (R, $\pi$ -3p)        | 6.939            | 0.000 | 0.000 | 0.000 | 6.953            |       |       |       |

| Molecule              | State                                  | LR-CC2/AVDZ      |       |       |       | LR-CC3/dAVDZ     |       |       |       |
|-----------------------|----------------------------------------|------------------|-------|-------|-------|------------------|-------|-------|-------|
|                       |                                        | $\Delta E_{0,n}$ | $f^l$ | $f^v$ | $f^m$ | $\Delta E_{0,n}$ | $f^l$ | $f^v$ | $f^m$ |
| Methylenecyclopropene | 1B <sub>1</sub> (R, $\pi$ -3s)         | 5.223            | 0.005 | 0.005 | 0.005 | 5.310            |       |       |       |
|                       | 1B <sub>2</sub> (V, $\pi$ - $\pi^*$ )  | 4.510            | 0.013 | 0.008 | 0.011 | 4.316            |       |       |       |
|                       | 1A <sub>2</sub> (R, $\pi$ -3p)         | 5.727            | 0.000 | 0.000 | 0.000 | 5.816            |       |       |       |
| Pyrazine              | 2A <sub>g</sub> (R, n-3s)              | 6.070            | 0.000 | 0.000 | 0.000 | 6.499            |       |       |       |
|                       | 1B <sub>1u</sub> (V, $\pi$ - $\pi^*$ ) | 6.855            | 0.000 | 0.000 | 0.000 | 6.920            |       |       |       |
|                       | 2B <sub>1u</sub> (R, n-3p)             | 7.014            | 0.138 | 0.126 | 0.132 | 7.280            |       |       |       |
|                       | 2B <sub>2u</sub> (R, n-3p)             | 6.605            | 0.045 | 0.041 | 0.043 | 7.089            |       |       |       |
| Pyridazine            | 1B <sub>3g</sub> (R, n.d.)             | 7.364            | 0.000 | 0.000 | 0.000 | 7.807            |       |       |       |
|                       | 2B <sub>1</sub> (V, n- $\pi^*$ )       | 6.383            | 0.005 | 0.005 | 0.005 | 6.406            |       |       |       |
|                       | 1A <sub>2</sub> (V, n- $\pi^*$ )       | 4.285            | 0.000 | 0.000 | 0.000 | 4.389            |       |       |       |
|                       | 1B <sub>1</sub> (R, mixed)             | 5.767            | 0.008 | 0.006 | 0.007 | 5.853            |       |       |       |
| Pyrrole               | 1A <sub>2</sub> (R, $\pi$ -3s)         | 5.089            | 0.000 | 0.000 | 0.000 | 5.125            |       |       |       |
|                       | 2A <sub>2</sub> (R, $\pi$ -3p)         | 5.845            | 0.000 | 0.000 | 0.000 | 5.869            |       |       |       |
|                       | 1A <sub>2</sub> (V, $\pi$ - $\pi^*$ )  | 2.379            | 0.000 | 0.000 | 0.000 | 2.180            | 0.000 | 0.000 | 0.000 |
| Silylidene            | 1B <sub>2</sub> (V, n- $\pi^*$ )       | 3.857            | 0.038 | 0.020 | 0.028 | 3.802            | 0.034 | 0.030 | 0.032 |
|                       | 1B <sub>2g</sub> (V, n- $\pi^*$ )      | 5.722            | 0.000 | 0.000 | 0.000 | 5.530            |       |       |       |
|                       | 1B <sub>1g</sub> (V, n- $\pi^*$ )      | 5.095            | 0.000 | 0.000 | 0.000 | 4.963            |       |       |       |
| Tetrazine             | 1B <sub>3u</sub> (V, n- $\pi^*$ )      | 2.420            | 0.006 | 0.005 | 0.007 | 2.486            |       |       |       |
|                       | 1A <sub>2</sub> (R, $\pi$ -3s)         | 5.957            | 0.000 | 0.000 | 0.000 | 6.023            |       |       |       |
|                       | 1B <sub>1</sub> (R, $\pi$ -3p)         | 6.146            | 0.020 | 0.021 | 0.020 | 6.169            |       |       |       |
| Thiophene             | 1A <sub>2</sub> (R, n-3p)              | 8.743            | 0.000 | 0.000 | 0.000 | 9.258            | 0.000 | 0.000 | 0.000 |
|                       | 1B <sub>1</sub> (R, n-3s)              | 7.089            | 0.060 | 0.061 | 0.061 | 7.493            | 0.053 | 0.055 | 0.054 |

Table S9: Ground state absorption data for LR-CCSD/dAVDZ and LR-CC2/dAVDZ calculations.

| Molecule        | State                                 | LR-CCSD/dAVDZ    |       |       |       | LR-CC2/dAVDZ     |       |       |       |
|-----------------|---------------------------------------|------------------|-------|-------|-------|------------------|-------|-------|-------|
|                 |                                       | $\Delta E_{0,n}$ | $f^l$ | $f^v$ | $f^m$ | $\Delta E_{0,n}$ | $f^l$ | $f^v$ | $f^m$ |
| Acetone         | 2A <sub>1</sub> (R, n-3p)             | 7.368            |       |       |       | 6.625            |       |       |       |
|                 | 1B <sub>2</sub> (R, n-3s)             | 6.365            |       |       |       | 5.710            |       |       |       |
|                 | 2B <sub>2</sub> (R, n-3p)             | 7.342            |       |       |       | 6.629            |       |       |       |
|                 | 2A <sub>2</sub> (R, n-3p)             | 7.266            |       |       |       | 6.551            |       |       |       |
| Acrolein        | 1A'' (V, n- $\pi^*$ )                 | 3.901            |       |       |       | 3.867            |       |       |       |
|                 | 2A'' (V, n- $\pi^*$ )                 | 7.164            |       |       |       | 6.581            |       |       |       |
| Ammonia         | 1A <sub>2</sub> (R, n-3s)             | 6.447            | 0.083 | 0.088 | 0.086 | 6.236            | 0.086 | 0.088 | 0.087 |
|                 | 1E (R, n-3p)                          | 7.955            | 0.002 | 0.002 | 0.002 | 7.635            | 0.002 | 0.002 | 0.002 |
|                 | 2A <sub>1</sub> (R, n-3p)             | 8.395            | 0.000 | 0.000 | 0.000 | 8.008            | 0.000 | 0.000 | 0.000 |
|                 | 2A <sub>2</sub> (R, n-4s)             | 8.935            | 0.001 | 0.002 | 0.002 | 8.491            | 0.004 | 0.004 | 0.004 |
| Benzene         | 1E <sub>1g</sub> (R, $\pi$ -3s)       | 6.443            |       |       |       | 6.307            |       |       |       |
|                 | 1E <sub>2u</sub> (R, $\pi$ -3p)       | 7.039            |       |       |       | 6.871            |       |       |       |
| Butadiene       | 1A <sub>2u</sub> (R, $\pi$ -3p)       | 6.968            |       |       |       | 6.814            |       |       |       |
|                 | 1B <sub>g</sub> (R, $\pi$ -3s)        | 6.256            |       |       |       | 6.074            |       |       |       |
|                 | 2B <sub>g</sub> (R, $\pi$ -3d)        | 7.379            |       |       |       | 7.140            |       |       |       |
|                 | 1A <sub>u</sub> (R, $\pi$ -3p)        | 6.575            |       |       |       | 6.392            |       |       |       |
| Carbon monoxide | 2A <sub>u</sub> (R, $\pi$ -3p)        | 6.730            |       |       |       | 6.518            |       |       |       |
|                 | 2 $\Sigma^+$ (R, n.d.)                | 10.794           | 0.009 | 0.008 | 0.008 | 10.670           | 0.006 | 0.007 | 0.006 |
|                 | 3 $\Sigma^+$ (R, n.d.)                | 11.393           | 0.134 | 0.131 | 0.133 | 11.241           | 0.126 | 0.120 | 0.123 |
|                 | 1 $\Pi$ (V, n- $\pi^*$ )              | 8.663            | 0.084 | 0.080 | 0.082 | 8.714            | 0.085 | 0.072 | 0.078 |
| Cyclopentadiene | 2 $\Pi$ (R, n.d.)                     | 11.535           | 0.034 | 0.033 | 0.033 | 11.369           | 0.032 | 0.032 | 0.032 |
|                 | 2A <sub>1</sub> (V, $\pi$ - $\pi^*$ ) | 6.918            |       |       |       | 6.794            |       |       |       |
|                 | 1A <sub>2</sub> (R, $\pi$ -3s)        | 5.699            |       |       |       | 5.488            |       |       |       |

| Molecule     | State                                 | LR-CCSD/dAVDZ    |       |       |       | LR-CC2/dAVDZ     |       |       |       |
|--------------|---------------------------------------|------------------|-------|-------|-------|------------------|-------|-------|-------|
|              |                                       | $\Delta E_{0,n}$ | $f^l$ | $f^v$ | $f^m$ | $\Delta E_{0,n}$ | $f^l$ | $f^v$ | $f^m$ |
| Cyclopropene | 2A <sub>2</sub> (R, $\pi$ -3p)        | 6.337            |       |       |       | 6.093            |       |       |       |
|              | 1B <sub>1</sub> (R, $\pi$ -3p)        | 6.292            |       |       |       | 6.054            |       |       |       |
|              | 1B <sub>2</sub> (V, $\pi$ - $\pi^*$ ) | 5.700            |       |       |       | 5.540            |       |       |       |
|              | 2B <sub>2</sub> (R, $\pi$ -3p)        | 6.365            |       |       |       | 6.132            |       |       |       |
|              | 2B <sub>1</sub> (R, $\pi$ -3s)        | 6.856            |       |       |       | 6.754            |       |       |       |
|              | 3B <sub>1</sub> (R, $\pi$ -3p)        | 7.236            |       |       |       | 7.047            |       |       |       |
| Diazirine    | 1B <sub>1</sub> (V, n- $\pi^*$ )      | 4.236            | 0.002 | 0.004 | 0.003 | 4.253            | 0.002 | 0.003 | 0.003 |
|              | 1B <sub>2</sub> (R, n-3s)             | 7.391            |       |       |       | 7.077            |       |       |       |
| Diazomethane | 2A <sub>1</sub> (V, $\pi$ - $\pi^*$ ) | 7.885            | 0.104 | 0.092 | 0.098 | 7.558            | 0.098 | 0.085 | 0.091 |
|              | 1B <sub>1</sub> (R, $\pi$ -3s)        | 5.389            |       |       |       | 5.337            |       |       |       |
| Formaldehyde | 1A <sub>2</sub> (V, $\pi$ - $\pi^*$ ) | 3.228            |       |       |       | 3.408            |       |       |       |
|              | 2A <sub>1</sub> (R, n-3p)             | 7.962            |       |       |       | 7.287            |       |       |       |
|              | 1B <sub>2</sub> (R, n-3s)             | 7.027            |       |       |       | 6.374            |       |       |       |
|              | 2B <sub>2</sub> (R, n-3p)             | 7.834            |       |       |       | 7.249            |       |       |       |
|              | 1A <sub>2</sub> (V, n- $\pi^*$ )      | 4.012            |       |       |       | 4.083            |       |       |       |
|              | 2A <sub>2</sub> (R, n-3p)             | 8.181            |       |       |       | 7.525            |       |       |       |
| Furane       | 1B <sub>1</sub> (R, $\pi$ -3p)        | 6.546            |       |       |       | 6.386            |       |       |       |
|              | 2B <sub>2</sub> (R, $\pi$ -3p)        | 6.870            |       |       |       | 6.737            |       |       |       |
|              | 1A <sub>2</sub> (R, $\pi$ -3s)        | 6.019            |       |       |       | 5.877            |       |       |       |
|              | 2A <sub>2</sub> (R, $\pi$ -3p)        | 6.703            |       |       |       | 6.526            |       |       |       |
| Glyoxal      | 1A <sub>u</sub> (V, n- $\pi^*$ )      | 3.006            |       |       |       | 2.924            |       |       |       |
|              | 1B <sub>g</sub> (V, n- $\pi^*$ )      | 4.416            |       |       |       | 4.455            |       |       |       |
|              | 2B <sub>g</sub> (V, n- $\pi^*$ )      | 7.022            |       |       |       | 6.465            |       |       |       |
| Ketene       | 2A <sub>1</sub> (V, $\pi$ - $\pi^*$ ) | 7.060            |       |       |       | 6.881            |       |       |       |
|              | 1B <sub>1</sub> (R, $\pi$ -3s)        | 5.917            |       |       |       | 5.760            |       |       |       |
|              | 2A <sub>2</sub> (R, $\pi$ -3p)        | 7.056            |       |       |       | 6.832            |       |       |       |

| Molecule              | State                                  | LR-CCSD/dAVDZ    |       |       |       | LR-CC2/dAVDZ     |       |       |       |
|-----------------------|----------------------------------------|------------------|-------|-------|-------|------------------|-------|-------|-------|
|                       |                                        | $\Delta E_{0,n}$ | $f^l$ | $f^v$ | $f^m$ | $\Delta E_{0,n}$ | $f^l$ | $f^v$ | $f^m$ |
| Methylenecyclopropene | 1B <sub>1</sub> (R, $\pi$ -3s)         | 5.322            |       |       |       | 5.168            |       |       |       |
|                       | 1B <sub>2</sub> (V, $\pi$ - $\pi^*$ )  | 4.547            |       |       |       | 4.503            |       |       |       |
|                       | 1A <sub>2</sub> (R, $\pi$ -3p)         | 5.829            |       |       |       | 5.651            |       |       |       |
| Pyrazine              | 2A <sub>g</sub> (R, n-3s)              | 6.616            |       |       |       | 6.012            |       |       |       |
|                       | 1B <sub>1u</sub> (V, $\pi$ - $\pi^*$ ) | 7.011            |       |       |       | 6.729            |       |       |       |
|                       | 2B <sub>1u</sub> (R, n-3p)             | 7.365            |       |       |       | 6.986            |       |       |       |
|                       | 2B <sub>2u</sub> (R, n-3p)             | 7.213            |       |       |       | 6.530            |       |       |       |
|                       | 1B <sub>3g</sub> (R, n.d.)             | 7.896            |       |       |       | 7.207            |       |       |       |
| Pyridazine            | 2B <sub>1</sub> (V, n- $\pi^*$ )       | 6.660            |       |       |       | 6.377            |       |       |       |
|                       | 1A <sub>2</sub> (V, n- $\pi^*$ )       | 4.624            |       |       |       | 4.280            |       |       |       |
| Pyrrole               | 1B <sub>1</sub> (R, mixed)             | 5.873            |       |       |       | 5.724            |       |       |       |
|                       | 1A <sub>2</sub> (R, $\pi$ -3s)         | 5.194            |       |       |       | 5.055            |       |       |       |
|                       | 2A <sub>2</sub> (R, $\pi$ -3p)         | 5.911            |       |       |       | 5.755            |       |       |       |
| Silylidene            | 1A <sub>2</sub> (V, $\pi$ - $\pi^*$ )  | 2.289            | 0.000 | 0.000 | 0.000 | 2.379            | 0.000 | 0.000 | 0.000 |
|                       | 1B <sub>2</sub> (V, n- $\pi^*$ )       | 3.876            | 0.036 | 0.027 | 0.031 | 3.857            | 0.038 | 0.020 | 0.028 |
| Tetrazine             | 1B <sub>2g</sub> (V, n- $\pi^*$ )      | 5.878            |       |       |       | 5.719            |       |       |       |
|                       | 1B <sub>1g</sub> (V, n- $\pi^*$ )      | 5.300            |       |       |       | 5.092            |       |       |       |
|                       | 1B <sub>3u</sub> (V, n- $\pi^*$ )      | 2.648            |       |       |       | 2.419            |       |       |       |
| Thiophene             | 1A <sub>2</sub> (R, $\pi$ -3s)         | 6.075            |       |       |       | 5.898            |       |       |       |
|                       | 1B <sub>1</sub> (R, $\pi$ -3p)         | 6.281            |       |       |       | 6.113            |       |       |       |
| Water                 | 1A <sub>2</sub> (R, n-3p)              | 9.179            | 0.000 | 0.000 | 0.000 | 8.694            | 0.000 | 0.000 | 0.000 |
|                       | 1B <sub>1</sub> (R, n-3s)              | 7.429            | 0.052 | 0.057 | 0.054 | 7.067            | 0.055 | 0.056 | 0.055 |

Table S10: Ground state absorption data for LR-CC3/AVTZ and LR-CCSD/AVTZ calculations.

| Molecule        | State                                 | LR-CC3/AVTZ      |       |       |       | LR-CCSD/AVTZ     |       |       |       |
|-----------------|---------------------------------------|------------------|-------|-------|-------|------------------|-------|-------|-------|
|                 |                                       | $\Delta E_{0,n}$ | $f^l$ | $f^v$ | $f^m$ | $\Delta E_{0,n}$ | $f^l$ | $f^v$ | $f^m$ |
| Acetone         | 2A <sub>1</sub> (R, n-3p)             | 7.484            |       |       |       | 7.626            |       |       |       |
|                 | 1B <sub>2</sub> (R, n-3s)             | 6.427            |       |       |       | 6.586            |       |       |       |
|                 | 2B <sub>2</sub> (R, n-3p)             | 7.595            |       |       |       | 7.701            |       |       |       |
|                 | 2A <sub>2</sub> (R, n-3p)             | 7.449            |       |       |       | 7.567            |       |       |       |
| Acrolein        | 1A'' (V, n- $\pi^*$ )                 | 3.743            |       |       |       | 3.913            |       |       |       |
|                 | 2A'' (V, n- $\pi^*$ )                 | 6.752            |       |       |       | 7.269            |       |       |       |
| Ammonia         | 1A <sub>2</sub> (R, n-3s)             | 6.573            | 0.085 | 0.087 | 0.086 | 6.600            | 0.084 | 0.086 | 0.085 |
|                 | 1E (R, n-3p)                          | 8.146            | 0.003 | 0.003 | 0.003 | 8.148            | 0.003 | 0.003 | 0.003 |
|                 | 2A <sub>1</sub> (R, n-3p)             | 9.318            | 0.003 | 0.003 | 0.003 | 9.334            | 0.003 | 0.003 | 0.003 |
|                 | 2A <sub>2</sub> (R, n-4s)             | 9.945            | 0.008 | 0.010 | 0.009 | 9.953            | 0.009 | 0.012 | 0.010 |
| Benzene         | 1E <sub>1g</sub> (R, $\pi$ -3s)       | 6.520            |       |       |       | 6.577            |       |       |       |
|                 | 1E <sub>2u</sub> (R, $\pi$ -3p)       | 7.147            |       |       |       | 7.197            |       |       |       |
| Butadiene       | 1A <sub>2u</sub> (R, $\pi$ -3p)       | 7.079            |       |       |       | 7.117            |       |       |       |
|                 | 1B <sub>g</sub> (R, $\pi$ -3s)        | 6.329            |       |       |       | 6.398            |       |       |       |
|                 | 2B <sub>g</sub> (R, $\pi$ -3d)        | 7.447            |       |       |       | 7.508            |       |       |       |
|                 | 1A <sub>u</sub> (R, $\pi$ -3p)        | 6.643            |       |       |       | 6.713            |       |       |       |
| Carbon monoxide | 2A <sub>u</sub> (R, $\pi$ -3p)        | 6.799            |       |       |       | 6.874            |       |       |       |
|                 | 2 $\Sigma^+$ (R, n.d.)                | 10.944           |       |       |       | 11.222           |       |       |       |
|                 | 3 $\Sigma^+$ (R, n.d.)                | 11.489           |       |       |       | 11.751           |       |       |       |
|                 | 1 $\Pi$ (V, n- $\pi^*$ )              | 8.486            |       |       |       | 8.587            |       |       |       |
| Cyclopentadiene | 2 $\Pi$ (R, n.d.)                     | 11.690           |       |       |       | 11.960           |       |       |       |
|                 | 2A <sub>1</sub> (V, $\pi$ - $\pi^*$ ) | 6.570            |       |       |       | 6.963            |       |       |       |
|                 | 1A <sub>2</sub> (R, $\pi$ -3s)        | 5.773            |       |       |       | 5.833            |       |       |       |

| Molecule     | State                                 | LR-CC3/AVTZ      |       |       |       | LR-CCSD/AVTZ     |       |       |       |
|--------------|---------------------------------------|------------------|-------|-------|-------|------------------|-------|-------|-------|
|              |                                       | $\Delta E_{0,n}$ | $f^l$ | $f^v$ | $f^m$ | $\Delta E_{0,n}$ | $f^l$ | $f^v$ | $f^m$ |
| Cyclopropene | 2A <sub>2</sub> (R, $\pi$ -3p)        | 6.447            |       |       |       | 6.502            |       |       |       |
|              | 1B <sub>1</sub> (R, $\pi$ -3p)        | 6.403            |       |       |       | 6.449            |       |       |       |
|              | 1B <sub>2</sub> (V, $\pi$ - $\pi^*$ ) | 5.540            |       |       |       | 5.668            |       |       |       |
|              | 2B <sub>2</sub> (R, $\pi$ -3p)        | 6.556            |       |       |       | 6.608            |       |       |       |
| Diazirine    | 2B <sub>1</sub> (R, $\pi$ -3s)        | 6.934            | 0.007 | 0.007 | 0.007 | 6.990            | 0.007 | 0.006 | 0.006 |
|              | 3B <sub>1</sub> (R, $\pi$ -3p)        | 7.320            | 0.028 | 0.030 | 0.029 | 7.382            | 0.028 | 0.031 | 0.030 |
|              | 1B <sub>1</sub> (V, $\pi$ - $\pi^*$ ) | 4.114            | 0.002 | 0.003 | 0.002 | 4.184            | 0.002 | 0.002 | 0.002 |
|              | 1B <sub>2</sub> (R, $\pi$ -3s)        | 7.450            | 0.000 | 0.000 | 0.000 | 7.554            | 0.000 | 0.001 | 0.000 |
| Diazomethane | 2A <sub>1</sub> (V, $\pi$ - $\pi^*$ ) | 8.037            | 0.132 | 0.132 | 0.132 | 8.115            | 0.132 | 0.118 | 0.125 |
|              | 1B <sub>1</sub> (R, $\pi$ -3s)        | 5.450            | 0.016 | 0.016 | 0.016 | 5.570            | 0.016 | 0.016 | 0.016 |
|              | 1A <sub>2</sub> (V, $\pi$ - $\pi^*$ ) | 3.070            | 0.000 | 0.000 | 0.000 | 3.191            | 0.000 | 0.000 | 0.000 |
|              | 2A <sub>1</sub> (R, $\pi$ -3p)        | 8.182            | 0.052 | 0.051 | 0.052 | 8.210            | 0.054 | 0.055 | 0.054 |
| Formaldehyde | 1B <sub>2</sub> (R, $\pi$ -3s)        | 7.179            | 0.021 | 0.021 | 0.021 | 7.231            | 0.018 | 0.018 | 0.018 |
|              | 2B <sub>2</sub> (R, $\pi$ -3p)        | 8.086            | 0.037 | 0.038 | 0.038 | 8.120            | 0.040 | 0.042 | 0.041 |
|              | 1A <sub>2</sub> (V, $\pi$ - $\pi^*$ ) | 3.970            |       |       |       | 4.013            |       |       |       |
|              | 2A <sub>2</sub> (R, $\pi$ -3p)        | 8.636            |       |       |       | 8.650            |       |       |       |
| Furane       | 1B <sub>1</sub> (R, $\pi$ -3p)        | 6.629            |       |       |       | 6.708            |       |       |       |
|              | 2B <sub>2</sub> (R, $\pi$ -3p)        | 7.233            |       |       |       | 7.324            |       |       |       |
|              | 1A <sub>2</sub> (R, $\pi$ -3s)        | 6.078            |       |       |       | 6.168            |       |       |       |
|              | 2A <sub>2</sub> (R, $\pi$ -3p)        | 6.799            |       |       |       | 6.890            |       |       |       |
| Glyoxal      | 1A <sub>u</sub> (V, $\pi$ - $\pi^*$ ) | 2.876            |       |       |       | 3.009            |       |       |       |
|              | 1B <sub>g</sub> (V, $\pi$ - $\pi^*$ ) | 4.269            |       |       |       | 4.418            |       |       |       |
|              | 2B <sub>g</sub> (V, $\pi$ - $\pi^*$ ) | 6.578            |       |       |       | 7.123            |       |       |       |
|              | 2A <sub>1</sub> (V, $\pi$ - $\pi^*$ ) | 7.231            | 0.154 | 0.149 | 0.151 | 7.356            | 0.168 | 0.145 | 0.157 |
| Ketene       | 1B <sub>1</sub> (R, $\pi$ -3s)        | 5.956            | 0.035 | 0.035 | 0.035 | 6.093            | 0.034 | 0.032 | 0.033 |
|              | 2A <sub>2</sub> (R, $\pi$ -3p)        | 7.157            | 0.000 | 0.000 | 0.000 | 7.292            | 0.000 | 0.000 | 0.000 |

| Molecule              | State                                  | LR-CC3/AVTZ      |       |       |       | LR-CCSD/AVTZ     |       |       |       |
|-----------------------|----------------------------------------|------------------|-------|-------|-------|------------------|-------|-------|-------|
|                       |                                        | $\Delta E_{0,n}$ | $f^l$ | $f^v$ | $f^m$ | $\Delta E_{0,n}$ | $f^l$ | $f^v$ | $f^m$ |
| Methylenecyclopropene | 1B <sub>1</sub> (R, $\pi$ -3s)         | 5.439            |       |       |       | 5.479            |       |       |       |
|                       | 1B <sub>2</sub> (V, $\pi$ - $\pi^*$ )  | 4.312            |       |       |       | 4.583            |       |       |       |
|                       | 1A <sub>2</sub> (R, $\pi$ -3p)         | 5.954            |       |       |       | 5.999            |       |       |       |
| Pyrazine              | 2A <sub>g</sub> (R, n-3s)              | 6.656            |       |       |       | 6.830            |       |       |       |
|                       | 1B <sub>1u</sub> (V, $\pi$ - $\pi^*$ ) | 6.862            |       |       |       | 6.958            |       |       |       |
|                       | 2B <sub>1u</sub> (R, n-3p)             | 7.453            |       |       |       | 7.596            |       |       |       |
|                       | 2B <sub>2u</sub> (R, n-3p)             | 7.253            |       |       |       | 7.441            |       |       |       |
|                       | 1B <sub>3g</sub> (R, n.d.)             | 8.001            |       |       |       | 8.156            |       |       |       |
| Pyridazine            | 2B <sub>1</sub> (V, n- $\pi^*$ )       | 6.369            |       |       |       | 6.667            |       |       |       |
|                       | 1A <sub>2</sub> (V, n- $\pi^*$ )       | 4.373            |       |       |       | 4.653            |       |       |       |
| Pyrrole               | 1B <sub>1</sub> (R, mixed)             | 5.982            |       |       |       | 6.038            |       |       |       |
|                       | 1A <sub>2</sub> (R, $\pi$ -3s)         | 5.241            |       |       |       | 5.340            |       |       |       |
| Silylidene            | 2A <sub>2</sub> (R, $\pi$ -3p)         | 6.013            |       |       |       | 6.088            |       |       |       |
|                       | 1A <sub>2</sub> (V, $\pi$ - $\pi^*$ )  | 2.154            |       |       |       | 2.286            |       |       |       |
|                       | 1B <sub>2</sub> (V, n- $\pi^*$ )       | 3.780            |       |       |       | 3.877            |       |       |       |
| Tetrazine             | 1B <sub>2g</sub> (V, n- $\pi^*$ )      | 5.464            |       |       |       | 5.836            |       |       |       |
|                       | 1B <sub>1g</sub> (V, n- $\pi^*$ )      | 4.910            |       |       |       | 5.264            |       |       |       |
|                       | 1B <sub>3u</sub> (V, n- $\pi^*$ )      | 2.455            |       |       |       | 2.635            |       |       |       |
| Thiophene             | 1A <sub>2</sub> (R, $\pi$ -3s)         | 6.141            |       |       |       | 6.218            |       |       |       |
|                       | 1B <sub>1</sub> (R, $\pi$ -3p)         | 6.136            |       |       |       | 6.307            |       |       |       |
| Water                 | 1A <sub>2</sub> (R, n-3p)              | 9.382            | 0.000 | 0.000 | 0.000 | 9.361            | 0.000 | 0.000 | 0.000 |
|                       | 1B <sub>1</sub> (R, n-3s)              | 7.605            | 0.055 | 0.056 | 0.055 | 7.596            | 0.053 | 0.057 | 0.055 |



Table S11: Ground state absorption data for LR-CC2/AVTZ and LR-CC3/dAVTZ calculations.

| Molecule        | State                                 | LR-CC2/AVTZ      |       |       |       | LR-CC3/dAVTZ     |       |       |       |
|-----------------|---------------------------------------|------------------|-------|-------|-------|------------------|-------|-------|-------|
|                 |                                       | $\Delta E_{0,n}$ | $f^l$ | $f^v$ | $f^m$ | $\Delta E_{0,n}$ | $f^l$ | $f^v$ | $f^m$ |
| Acetone         | 2A <sub>1</sub> (R, n-3p)             | 6.887            |       |       |       | 7.450            |       |       |       |
|                 | 1B <sub>2</sub> (R, n-3s)             | 5.912            |       |       |       | 6.418            |       |       |       |
|                 | 2B <sub>2</sub> (R, n-3p)             | 7.024            |       |       |       | 7.456            |       |       |       |
|                 | 2A <sub>2</sub> (R, n-3p)             | 6.842            |       |       |       | 7.382            |       |       |       |
| Acrolein        | 1A'' (V, n- $\pi^*$ )                 | 3.853            |       |       |       | 3.741            |       |       |       |
|                 | 2A'' (V, n- $\pi^*$ )                 | 6.681            |       |       |       | 6.743            |       |       |       |
| Ammonia         | 1A <sub>2</sub> (R, n-3s)             | 6.387            | 0.087 | 0.086 | 0.086 | 6.572            | 0.084 | 0.087 | 0.085 |
|                 | 1E (R, n-3p)                          | 7.847            | 0.003 | 0.002 | 0.003 | 8.117            | 0.003 | 0.003 | 0.003 |
|                 | 2A <sub>1</sub> (R, n-3p)             | 9.051            | 0.002 | 0.002 | 0.002 | 8.565            | 0.000 | 0.000 | 0.000 |
|                 | 2A <sub>2</sub> (R, n-4s)             | 9.654            | 0.014 | 0.017 | 0.015 | 9.120            | 0.001 | 0.001 | 0.001 |
| Benzene         | 1E <sub>1g</sub> (R, $\pi$ -3s)       | 6.470            |       |       |       | 6.504            |       |       |       |
|                 | 1E <sub>2u</sub> (R, $\pi$ -3p)       | 7.064            |       |       |       | 7.117            |       |       |       |
| Butadiene       | 1A <sub>2u</sub> (R, $\pi$ -3p)       | 7.002            |       |       |       | 7.053            |       |       |       |
|                 | 1B <sub>g</sub> (R, $\pi$ -3s)        | 6.256            |       |       |       | 6.311            |       |       |       |
|                 | 2B <sub>g</sub> (R, $\pi$ -3d)        | 7.305            |       |       |       | 7.447            |       |       |       |
|                 | 1A <sub>u</sub> (R, $\pi$ -3p)        | 6.572            |       |       |       | 6.626            |       |       |       |
| Carbon monoxide | 2A <sub>u</sub> (R, $\pi$ -3p)        | 6.702            |       |       |       | 6.780            |       |       |       |
|                 | 2 $\Sigma^+$ (R, n.d.)                | 11.106           |       |       |       | 10.676           |       |       |       |
|                 | 3 $\Sigma^+$ (R, n.d.)                | 11.626           |       |       |       | 11.285           |       |       |       |
|                 | 1 $\Pi$ (V, n- $\pi^*$ )              | 8.638            |       |       |       | 8.481            |       |       |       |
| Cyclopentadiene | 2 $\Pi$ (R, n.d.)                     | 11.825           |       |       |       | 11.414           |       |       |       |
|                 | 2A <sub>1</sub> (V, $\pi$ - $\pi^*$ ) | 6.860            |       |       |       | 6.567            |       |       |       |
|                 | 1A <sub>2</sub> (R, $\pi$ -3s)        | 5.659            |       |       |       | 5.759            |       |       |       |

| Molecule     | State                                 | LR-CC2/AVTZ      |       |       |       | LR-CC3/dAVTZ     |       |       |       |
|--------------|---------------------------------------|------------------|-------|-------|-------|------------------|-------|-------|-------|
|              |                                       | $\Delta E_{0,n}$ | $f^l$ | $f^v$ | $f^m$ | $\Delta E_{0,n}$ | $f^l$ | $f^v$ | $f^m$ |
| Cyclopropene | 2A <sub>2</sub> (R, $\pi$ -3p)        | 6.303            |       |       |       | 6.412            |       |       |       |
|              | 1B <sub>1</sub> (R, $\pi$ -3p)        | 6.256            |       |       |       | 6.375            |       |       |       |
|              | 1B <sub>2</sub> (V, $\pi$ - $\pi^*$ ) | 5.522            |       |       |       | 5.538            |       |       |       |
|              | 2B <sub>2</sub> (R, $\pi$ -3p)        | 6.421            |       |       |       | 6.448            |       |       |       |
|              | 2B <sub>1</sub> (R, $\pi$ -3s)        | 6.832            | 0.007 | 0.007 | 0.007 | 6.921            |       |       |       |
|              | 3B <sub>1</sub> (R, $\pi$ -3p)        | 7.228            | 0.030 | 0.030 | 0.030 | 7.294            |       |       |       |
|              | 1B <sub>1</sub> (V, n- $\pi^*$ )      | 4.204            | 0.002 | 0.002 | 0.002 | 4.112            | 0.002 | 0.003 | 0.002 |
|              | 1B <sub>2</sub> (R, n-3s)             | 7.257            | 0.001 | 0.002 | 0.002 | 7.442            |       |       |       |
| Diazirine    | 2A <sub>1</sub> (V, $\pi$ - $\pi^*$ ) | 7.808            | 0.130 | 0.115 | 0.122 | 7.972            | 0.113 | 0.114 | 0.114 |
|              | 1B <sub>1</sub> (R, $\pi$ -3s)        | 5.528            | 0.019 | 0.019 | 0.019 | 5.436            |       |       |       |
| Diazomethane | 1A <sub>2</sub> (V, $\pi$ - $\pi^*$ ) | 3.367            | 0.000 | 0.000 | 0.000 | 3.071            |       |       |       |
|              | 2A <sub>1</sub> (R, n-3p)             | 7.518            | 0.055 | 0.054 | 0.054 | 8.145            |       |       |       |
| Formaldehyde | 1B <sub>2</sub> (R, n-3s)             | 6.558            | 0.022 | 0.020 | 0.021 | 7.173            |       |       |       |
|              | 2B <sub>2</sub> (R, n-3p)             | 7.568            | 0.033 | 0.032 | 0.032 | 7.995            |       |       |       |
| Furane       | 1A <sub>2</sub> (V, n- $\pi^*$ )      | 4.072            |       |       |       | 3.968            |       |       |       |
|              | 2A <sub>2</sub> (R, n-3p)             | 8.043            |       |       |       | 8.386            |       |       |       |
|              | 1B <sub>1</sub> (R, $\pi$ -3p)        | 6.586            |       |       |       | 6.606            |       |       |       |
|              | 2B <sub>2</sub> (R, $\pi$ -3p)        | 7.246            |       |       |       | 6.883            |       |       |       |
|              | 1A <sub>2</sub> (R, $\pi$ -3s)        | 6.057            |       |       |       | 6.061            |       |       |       |
|              | 2A <sub>2</sub> (R, $\pi$ -3p)        | 6.751            |       |       |       | 6.754            |       |       |       |
|              | 1A <sub>u</sub> (V, n- $\pi^*$ )      | 2.913            |       |       |       | 2.874            |       |       |       |
|              | 1B <sub>g</sub> (V, n- $\pi^*$ )      | 4.438            |       |       |       | 4.267            |       |       |       |
| Glyoxal      | 2B <sub>g</sub> (V, n- $\pi^*$ )      | 6.511            |       |       |       | 6.566            |       |       |       |
|              | 2A <sub>1</sub> (V, $\pi$ - $\pi^*$ ) | 7.260            | 0.175 | 0.156 | 0.165 | 7.085            |       |       |       |
| Ketene       | 1B <sub>1</sub> (R, $\pi$ -3s)        | 5.942            | 0.034 | 0.032 | 0.033 | 5.948            |       |       |       |
|              | 2A <sub>2</sub> (R, $\pi$ -3p)        | 7.086            | 0.000 | 0.000 | 0.000 | 7.109            |       |       |       |

| Molecule              | State                                  | LR-CC2/AVTZ      |       |       |       | LR-CC3/dAVTZ     |       |       |       |
|-----------------------|----------------------------------------|------------------|-------|-------|-------|------------------|-------|-------|-------|
|                       |                                        | $\Delta E_{0,n}$ | $f^l$ | $f^v$ | $f^m$ | $\Delta E_{0,n}$ | $f^l$ | $f^v$ | $f^m$ |
| Methylenecyclopropene | 1B <sub>1</sub> (R, $\pi$ -3s)         | 5.355            |       |       |       | 5.422            |       |       |       |
|                       | 1B <sub>2</sub> (V, $\pi$ - $\pi^*$ )  | 4.507            |       |       |       | 4.311            |       |       |       |
|                       | 1A <sub>2</sub> (R, $\pi$ -3p)         | 5.852            |       |       |       | 5.928            |       |       |       |
| Pyrazine              | 2A <sub>g</sub> (R, n-3s)              | 6.205            |       |       |       | 6.638            |       |       |       |
|                       | 1B <sub>1u</sub> (V, $\pi$ - $\pi^*$ ) | 6.889            |       |       |       | 6.860            |       |       |       |
|                       | 2B <sub>1u</sub> (R, n-3p)             | 7.032            |       |       |       | 7.410            |       |       |       |
|                       | 2B <sub>2u</sub> (R, n-3p)             | 6.742            |       |       |       | 7.229            |       |       |       |
|                       | 1B <sub>3g</sub> (R, n.d.)             | 7.474            |       |       |       | 7.951            |       |       |       |
| Pyridazine            | 2B <sub>1</sub> (V, n- $\pi^*$ )       | 6.334            |       |       |       | 6.366            |       |       |       |
|                       | 1A <sub>2</sub> (V, n- $\pi^*$ )       | 4.260            |       |       |       | 4.372            |       |       |       |
| Pyrrole               | 1B <sub>1</sub> (R, mixed)             | 5.909            |       |       |       | 5.967            |       |       |       |
|                       | 1A <sub>2</sub> (R, $\pi$ -3s)         | 5.225            |       |       |       | 5.233            |       |       |       |
| Silylidene            | 2A <sub>2</sub> (R, $\pi$ -3p)         | 5.965            |       |       |       | 5.980            |       |       |       |
|                       | 1A <sub>2</sub> (V, $\pi$ - $\pi^*$ )  | 2.366            |       |       |       | 2.155            | 0.000 | 0.000 | 0.000 |
|                       | 1B <sub>2</sub> (V, n- $\pi^*$ )       | 3.852            |       |       |       | 3.780            | 0.033 | 0.030 | 0.032 |
|                       | 1B <sub>2g</sub> (V, n- $\pi^*$ )      | 5.641            |       |       |       | 5.463            |       |       |       |
|                       | 1B <sub>1g</sub> (V, n- $\pi^*$ )      | 5.016            |       |       |       | 4.910            |       |       |       |
| Tetrazine             | 1B <sub>3u</sub> (V, n- $\pi^*$ )      | 2.379            |       |       |       | 2.454            |       |       |       |
|                       | 1A <sub>2</sub> (R, $\pi$ -3s)         | 6.071            |       |       |       | 6.121            |       |       |       |
|                       | 1B <sub>1</sub> (R, $\pi$ -3p)         | 6.155            |       |       |       | 6.130            |       |       |       |
| Thiophene             | 1A <sub>2</sub> (R, n-3p)              | 8.889            | 0.000 | 0.000 | 0.000 | 9.368            | 0.000 | 0.000 | 0.000 |
|                       | 1B <sub>1</sub> (R, n-3s)              | 7.234            | 0.057 | 0.057 | 0.057 | 7.600            | 0.052 | 0.054 | 0.053 |

Table S12: Ground state absorption data for LR-CCSD/dAVTZ and LR-CC2/dAVTZ calculations.

| Molecule        | State                                 | LR-CCSD/dAVTZ    |       |       |       | LR-CC2/dAVTZ     |       |       |       |
|-----------------|---------------------------------------|------------------|-------|-------|-------|------------------|-------|-------|-------|
|                 |                                       | $\Delta E_{0,n}$ | $f^l$ | $f^v$ | $f^m$ | $\Delta E_{0,n}$ | $f^l$ | $f^v$ | $f^m$ |
| Acetone         | 2A <sub>1</sub> (R, n-3p)             | 7.585            |       |       |       | 6.826            |       |       |       |
|                 | 1B <sub>2</sub> (R, n-3s)             | 6.574            |       |       |       | 5.897            |       |       |       |
|                 | 2B <sub>2</sub> (R, n-3p)             | 7.563            |       |       |       | 6.832            |       |       |       |
|                 | 2A <sub>2</sub> (R, n-3p)             | 7.484            |       |       |       | 6.749            |       |       |       |
| Acrolein        | 1A'' (V, n- $\pi^*$ )                 | 3.911            |       |       |       | 3.851            |       |       |       |
|                 | 2A'' (V, n- $\pi^*$ )                 | 7.254            |       |       |       | 6.649            |       |       |       |
| Ammonia         | 1A <sub>2</sub> (R, n-3s)             | 6.600            | 0.082 | 0.086 | 0.084 | 6.384            | 0.086 | 0.086 | 0.086 |
|                 | 1E (R, n-3p)                          | 8.119            | 0.003 | 0.003 | 0.003 | 7.801            | 0.002 | 0.002 | 0.002 |
|                 | 2A <sub>1</sub> (R, n-3p)             | 8.565            | 0.000 | 0.000 | 0.000 | 8.174            | 0.000 | 0.000 | 0.000 |
|                 | 2A <sub>2</sub> (R, n-4s)             | 9.109            | 0.001 | 0.001 | 0.001 | 8.661            | 0.003 | 0.003 | 0.003 |
| Benzene         | 1E <sub>1g</sub> (R, $\pi$ -3s)       | 6.559            |       |       |       | 6.448            |       |       |       |
|                 | 1E <sub>2u</sub> (R, $\pi$ -3p)       | 7.165            |       |       |       | 7.024            |       |       |       |
|                 | 1A <sub>2u</sub> (R, $\pi$ -3p)       | 7.090            |       |       |       | 6.966            |       |       |       |
| Butadiene       | 1B <sub>g</sub> (R, $\pi$ -3s)        | 6.378            |       |       |       | 6.229            |       |       |       |
|                 | 2B <sub>g</sub> (R, $\pi$ -3d)        | 7.508            |       |       |       | 7.305            |       |       |       |
|                 | 1A <sub>u</sub> (R, $\pi$ -3p)        | 6.695            |       |       |       | 6.547            |       |       |       |
|                 | 2A <sub>u</sub> (R, $\pi$ -3p)        | 6.854            |       |       |       | 6.676            |       |       |       |
| Carbon monoxide | 2 $\Sigma^+$ (R, n.d.)                | 10.960           |       |       |       | 10.813           |       |       |       |
|                 | 3 $\Sigma^+$ (R, n.d.)                | 11.567           |       |       |       | 11.393           |       |       |       |
|                 | 1 $\Pi$ (V, n- $\pi^*$ )              | 8.582            |       |       |       | 8.633            |       |       |       |
| Cyclopentadiene | 2 $\Pi$ (R, n.d.)                     | 11.700           |       |       |       | 11.514           |       |       |       |
|                 | 2A <sub>1</sub> (V, $\pi$ - $\pi^*$ ) | 6.950            |       |       |       | 6.835            |       |       |       |
|                 | 1A <sub>2</sub> (R, $\pi$ -3s)        | 5.818            |       |       |       | 5.639            |       |       |       |

| Molecule     | State                                 | LR-CCSD/dAVTZ    |       |       |       | LR-CC2/dAVTZ     |       |       |       |
|--------------|---------------------------------------|------------------|-------|-------|-------|------------------|-------|-------|-------|
|              |                                       | $\Delta E_{0,n}$ | $f^l$ | $f^v$ | $f^m$ | $\Delta E_{0,n}$ | $f^l$ | $f^v$ | $f^m$ |
| Cyclopropene | 2A <sub>2</sub> (R, $\pi$ -3p)        | 6.465            |       |       |       | 6.255            |       |       |       |
|              | 1B <sub>1</sub> (R, $\pi$ -3p)        | 6.418            |       |       |       | 6.216            |       |       |       |
|              | 1B <sub>2</sub> (V, $\pi$ - $\pi^*$ ) | 5.666            |       |       |       | 5.520            |       |       |       |
|              | 2B <sub>2</sub> (R, $\pi$ -3p)        | 6.491            |       |       |       | 6.291            |       |       |       |
|              | 2B <sub>1</sub> (R, $\pi$ -3s)        | 6.976            |       |       |       | 6.814            |       |       |       |
|              | 3B <sub>1</sub> (R, $\pi$ -3p)        | 7.353            |       |       |       | 7.192            |       |       |       |
| Diazirine    | 1B <sub>1</sub> (V, n- $\pi^*$ )      | 4.184            | 0.002 | 0.002 | 0.002 | 4.203            | 0.002 | 0.002 | 0.002 |
|              | 1B <sub>2</sub> (R, n-3s)             | 7.543            |       |       |       | 7.241            |       |       |       |
| Diazomethane | 2A <sub>1</sub> (V, $\pi$ - $\pi^*$ ) | 8.046            | 0.113 | 0.101 | 0.107 | 7.720            | 0.107 | 0.094 | 0.100 |
|              | 1B <sub>1</sub> (R, $\pi$ -3s)        | 5.555            |       |       |       | 5.509            |       |       |       |
| Formaldehyde | 1A <sub>2</sub> (V, $\pi$ - $\pi^*$ ) | 3.192            |       |       |       | 3.368            |       |       |       |
|              | 2A <sub>1</sub> (R, n-3p)             | 8.169            |       |       |       | 7.472            |       |       |       |
|              | 1B <sub>2</sub> (R, n-3s)             | 7.224            |       |       |       | 6.549            |       |       |       |
|              | 2B <sub>2</sub> (R, n-3p)             | 8.026            |       |       |       | 7.425            |       |       |       |
| Furane       | 1A <sub>2</sub> (V, n- $\pi^*$ )      | 4.011            |       |       |       | 4.069            |       |       |       |
|              | 2A <sub>2</sub> (R, n-3p)             | 8.392            |       |       |       | 7.713            |       |       |       |
|              | 1B <sub>1</sub> (R, $\pi$ -3p)        | 6.683            |       |       |       | 6.554            |       |       |       |
|              | 2B <sub>2</sub> (R, $\pi$ -3p)        | 6.969            |       |       |       | 6.848            |       |       |       |
| Glyoxal      | 1A <sub>2</sub> (R, $\pi$ -3s)        | 6.151            |       |       |       | 6.035            |       |       |       |
|              | 2A <sub>2</sub> (R, $\pi$ -3p)        | 6.843            |       |       |       | 6.696            |       |       |       |
|              | 1A <sub>u</sub> (V, n- $\pi^*$ )      | 3.007            |       |       |       | 2.910            |       |       |       |
|              | 1B <sub>g</sub> (V, n- $\pi^*$ )      | 4.416            |       |       |       | 4.435            |       |       |       |
| Ketene       | 2B <sub>g</sub> (V, n- $\pi^*$ )      | 7.105            |       |       |       | 6.490            |       |       |       |
|              | 2A <sub>1</sub> (V, $\pi$ - $\pi^*$ ) | 7.212            |       |       |       | 7.048            |       |       |       |
|              | 1B <sub>1</sub> (R, $\pi$ -3s)        | 6.086            |       |       |       | 5.933            |       |       |       |
|              | 2A <sub>2</sub> (R, $\pi$ -3p)        | 7.246            |       |       |       | 7.030            |       |       |       |

| Molecule              | State                                  | LR-CCSD/dAVTZ    |       |       | LR-CC2/dAVTZ     |       |       |
|-----------------------|----------------------------------------|------------------|-------|-------|------------------|-------|-------|
|                       |                                        | $\Delta E_{0,n}$ | $f^l$ | $f^v$ | $\Delta E_{0,n}$ | $f^l$ | $f^m$ |
| Methylenecyclopropene | 1B <sub>1</sub> (R, $\pi$ -3s)         | 5.460            |       |       | 5.331            |       |       |
|                       | 1B <sub>2</sub> (V, $\pi$ - $\pi^*$ )  | 4.582            |       |       | 4.506            |       |       |
|                       | 1A <sub>2</sub> (R, $\pi$ -3p)         | 5.970            |       |       | 5.817            |       |       |
| Pyrazine              | 2A <sub>g</sub> (R, n-3s)              | 6.810            |       |       | 6.178            |       |       |
|                       | 1B <sub>1u</sub> (V, $\pi$ - $\pi^*$ ) | 6.956            |       |       | 6.863            |       |       |
|                       | 2B <sub>1u</sub> (R, n-3p)             | 7.548            |       |       | 6.980            |       |       |
|                       | 2B <sub>2u</sub> (R, n-3p)             | 7.414            |       |       | 6.702            |       |       |
|                       | 1B <sub>3g</sub> (R, n.d.)             | 8.099            |       |       | 7.386            |       |       |
| Pyridazine            | 2B <sub>1</sub> (V, n- $\pi^*$ )       | 6.666            |       |       | 6.332            |       |       |
|                       | 1A <sub>2</sub> (V, n- $\pi^*$ )       | 4.652            |       |       | 4.258            |       |       |
| Pyrrole               | 1B <sub>1</sub> (R, mixed)             | 6.021            |       |       | 5.891            |       |       |
|                       | 1A <sub>2</sub> (R, $\pi$ -3s)         | 5.331            |       |       | 5.213            |       |       |
|                       | 2A <sub>2</sub> (R, $\pi$ -3p)         | 6.052            |       |       | 5.921            |       |       |
| Silylidene            | 1A <sub>2</sub> (V, $\pi$ - $\pi^*$ )  | 2.287            | 0.000 | 0.000 | 2.366            | 0.000 | 0.000 |
|                       | 1B <sub>2</sub> (V, n- $\pi^*$ )       | 3.877            | 0.036 | 0.027 | 3.851            | 0.037 | 0.028 |
| Tetrazine             | 1B <sub>2g</sub> (V, n- $\pi^*$ )      | 5.835            |       |       | 5.640            |       |       |
|                       | 1B <sub>1g</sub> (V, n- $\pi^*$ )      | 5.263            |       |       | 5.015            |       |       |
|                       | 1B <sub>3u</sub> (V, n- $\pi^*$ )      | 2.634            |       |       | 2.378            |       |       |
| Thiophene             | 1A <sub>2</sub> (R, $\pi$ -3s)         | 6.198            |       |       | 6.044            |       |       |
|                       | 1B <sub>1</sub> (R, $\pi$ -3p)         | 6.301            |       |       | 6.146            |       |       |
| Water                 | 1A <sub>2</sub> (R, n-3p)              | 9.348            | 0.000 | 0.000 | 8.868            | 0.000 | 0.000 |
|                       | 1B <sub>1</sub> (R, n-3s)              | 7.592            | 0.051 | 0.055 | 7.226            | 0.054 | 0.054 |

### S2.3 Full testing set, ISR-ADC(2) with AVDZ, dAVDZ, AVTZ, and dAVTZ basis sets

Table S13: Ground state absorption data for ISR-ADC(2) obtained with AVDZ, dAVDZ, AVTZ and dAVTZ basis sets.  $\Delta E_{0,n}$  [eV] and oscillator strengths in length gauge ( $f^l$ ). Rydberg = R, valence = V.

| Molecule        | State                                 | AVDZ             |       |  | dAVDZ            |       |  | AVTZ             |       |  | dAVTZ            |       |  |
|-----------------|---------------------------------------|------------------|-------|--|------------------|-------|--|------------------|-------|--|------------------|-------|--|
|                 |                                       | $\Delta E_{0,n}$ | $f^l$ |  | $\Delta E_{0,n}$ | $f^l$ |  | $\Delta E_{0,n}$ | $f^l$ |  | $\Delta E_{0,n}$ | $f^l$ |  |
| Acetone         | 2A <sub>1</sub> (R, n-3p)             | 6.633            | 0.003 |  | 6.507            | 0.002 |  | 6.850            | 0.002 |  | 6.790            | 0.002 |  |
|                 | 1B <sub>2</sub> (R, n-3s)             | 5.628            | 0.024 |  | 5.591            | 0.023 |  | 5.871            | 0.024 |  | 5.856            | 0.023 |  |
|                 | 2B <sub>2</sub> (R, n-3p)             | 6.843            | 0.010 |  | 6.514            | 0.001 |  | 6.990            | 0.005 |  | 6.800            | 0.001 |  |
|                 | 2A <sub>2</sub> (R, n-3p)             | 6.608            | 0.000 |  | 6.433            | 0.000 |  | 6.805            | 0.000 |  | 6.713            | 0.000 |  |
| Acrolein        | 1A'' (V, n- $\pi^*$ )                 | 3.678            | 0.000 |  | 3.671            | 0.000 |  | 3.681            | 0.000 |  | 3.678            | 0.000 |  |
|                 | 2A'' (V, n- $\pi^*$ )                 | 6.517            | 0.000 |  | 6.446            | 0.000 |  | 6.590            | 0.000 |  | 6.561            | 0.000 |  |
| Ammonia         | 1A <sub>2</sub> (R, n-3s)             | 6.207            | 0.084 |  | 6.193            | 0.079 |  | 6.404            | 0.081 |  | 6.401            | 0.079 |  |
|                 | 1E (R, n-3p)                          | 7.691            | 0.003 |  | 7.593            | 0.002 |  | 7.866            | 0.003 |  | 7.821            | 0.002 |  |
|                 | 2A <sub>1</sub> (R, n-3p)             | 9.331            | 0.001 |  | 7.955            | 0.000 |  | 9.052            | 0.002 |  | 8.187            | 0.000 |  |
|                 | 2A <sub>2</sub> (R, n-4s)             | 10.105           | 0.029 |  | 8.450            | 0.004 |  | 9.673            | 0.015 |  | 8.681            | 0.003 |  |
| Benzene         | 1E <sub>1g</sub> (R, $\pi$ -3s)       | 6.367            | 0.000 |  | 6.316            | 0.000 |  | 6.524            | 0.000 |  | 6.502            | 0.000 |  |
|                 | 1E <sub>2u</sub> (R, $\pi$ -3p)       | 6.961            | 0.000 |  | 6.878            | 0.000 |  | 7.119            | 0.000 |  | 7.079            | 0.000 |  |
|                 | 1A <sub>2u</sub> (R, $\pi$ -3p)       | 6.896            | 0.071 |  | 6.820            | 0.059 |  | 7.056            | 0.067 |  | 7.021            | 0.060 |  |
|                 | 1B <sub>g</sub> (R, $\pi$ -3s)        | 6.142            | 0.000 |  | 6.085            | 0.000 |  | 6.310            | 0.000 |  | 6.284            | 0.000 |  |
| Butadiene       | 2B <sub>g</sub> (R, $\pi$ -3d)        | 7.362            | 0.000 |  | 7.152            | 0.000 |  | 7.482            | 0.000 |  | 7.364            | 0.000 |  |
|                 | 1A <sub>u</sub> (R, $\pi$ -3p)        | 6.460            | 0.001 |  | 6.403            | 0.001 |  | 6.626            | 0.001 |  | 6.602            | 0.001 |  |
|                 | 2A <sub>u</sub> (R, $\pi$ -3p)        | 6.593            | 0.056 |  | 6.531            | 0.046 |  | 6.760            | 0.051 |  | 6.733            | 0.046 |  |
|                 | 2 $\Sigma^+$ (R, n.d.)                | 11.277           | 0.016 |  | 10.854           | 0.019 |  | 11.322           | 0.026 |  | 11.033           | 0.022 |  |
| Carbon monoxide | 3 $\Sigma^+$ (R, n.d.)                | 11.779           | 0.258 |  | 11.442           | 0.123 |  | 11.833           | 0.214 |  | 11.631           | 0.126 |  |
|                 | 1 $\Pi$ (V, n- $\pi^*$ )              | 8.774            | 0.070 |  | 8.764            | 0.070 |  | 8.689            | 0.067 |  | 8.684            | 0.067 |  |
|                 | 2 $\Pi$ (R, n.d.)                     | 12.038           | 0.071 |  | 11.560           | 0.034 |  | 12.032           | 0.062 |  | 11.743           | 0.039 |  |
|                 | 2A <sub>1</sub> (V, $\pi$ - $\pi^*$ ) | 6.927            | 0.000 |  | 6.811            | 0.000 |  | 6.904            | 0.001 |  | 6.880            | 0.000 |  |
| Cyclopentadiene |                                       |                  |       |  |                  |       |  |                  |       |  |                  |       |  |



| Molecule     | State                                 | AVDZ             |       |       | dAVDZ |                  |       | AVTZ  |       |                  | dAVTZ |       |       |
|--------------|---------------------------------------|------------------|-------|-------|-------|------------------|-------|-------|-------|------------------|-------|-------|-------|
|              |                                       | $\Delta E_{0,n}$ | $f^l$ | $f^v$ | $f^m$ | $\Delta E_{0,n}$ | $f^l$ | $f^v$ | $f^m$ | $\Delta E_{0,n}$ | $f^l$ | $f^v$ | $f^m$ |
| Cyclopropene | 1A <sub>2</sub> (R, $\pi$ -3s)        | 5.543            | 0.000 | 5.496 | 0.000 | 5.711            | 0.000 | 5.691 | 0.000 | 5.711            | 0.000 | 5.691 | 0.000 |
|              | 2A <sub>2</sub> (R, $\pi$ -3p)        | 6.194            | 0.000 | 6.097 | 0.000 | 6.355            | 0.000 | 6.307 | 0.000 | 6.355            | 0.000 | 6.307 | 0.000 |
|              | 1B <sub>1</sub> (R, $\pi$ -3p)        | 6.138            | 0.043 | 6.057 | 0.033 | 6.306            | 0.038 | 6.267 | 0.033 | 6.306            | 0.038 | 6.267 | 0.033 |
|              | 1B <sub>2</sub> (V, $\pi$ - $\pi^*$ ) | 5.511            | 0.106 | 5.503 | 0.103 | 5.487            | 0.104 | 5.485 | 0.103 | 5.487            | 0.104 | 5.485 | 0.103 |
|              | 2B <sub>2</sub> (R, $\pi$ -3p)        | 6.372            | 0.052 | 6.138 | 0.039 | 6.475            | 0.047 | 6.344 | 0.039 | 6.475            | 0.047 | 6.344 | 0.039 |
|              | 2B <sub>1</sub> (R, $\pi$ -3s)        | 6.768            | 0.006 | 6.759 | 0.005 | 6.863            | 0.008 | 6.845 | 0.008 | 6.863            | 0.008 | 6.845 | 0.008 |
|              | 3B <sub>1</sub> (R, $\pi$ -3p)        | 7.105            | 0.031 | 6.640 | 0.004 | 7.258            | 0.030 | 7.222 | 0.027 | 7.258            | 0.030 | 7.222 | 0.027 |
|              | 1B <sub>1</sub> (V, n- $\pi^*$ )      | 4.266            | 0.002 | 4.264 | 0.002 | 4.209            | 0.002 | 4.208 | 0.002 | 4.209            | 0.002 | 4.208 | 0.002 |
| Diazirine    | 1B <sub>2</sub> (R, n-3s)             | 7.136            | 0.002 | 7.096 | 0.001 | 7.330            | 0.001 | 7.315 | 0.001 | 7.330            | 0.001 | 7.315 | 0.001 |
|              | 2A <sub>1</sub> (V, $\pi$ - $\pi^*$ ) | 7.736            | 0.135 | 7.574 | 0.096 | 7.873            | 0.132 | 7.789 | 0.108 | 7.873            | 0.132 | 7.789 | 0.108 |
| Diazomethane | 1B <sub>1</sub> (R, $\pi$ -3s)        | 5.432            | 0.018 | 5.391 | 0.017 | 5.626            | 0.017 | 5.607 | 0.016 | 5.626            | 0.017 | 5.607 | 0.016 |
|              | 1A <sub>2</sub> (V, $\pi$ - $\pi^*$ ) | 3.396            | 0.000 | 3.398 | 0.000 | 3.337            | 0.000 | 3.338 | 0.000 | 3.337            | 0.000 | 3.338 | 0.000 |
| Formaldehyde | 2A <sub>1</sub> (R, n-3p)             | 7.263            | 0.055 | 7.169 | 0.044 | 7.470            | 0.051 | 7.426 | 0.046 | 7.470            | 0.051 | 7.426 | 0.046 |
|              | 1B <sub>2</sub> (R, n-3s)             | 6.273            | 0.019 | 6.251 | 0.017 | 6.505            | 0.019 | 6.495 | 0.018 | 6.505            | 0.019 | 6.495 | 0.018 |
|              | 2B <sub>2</sub> (R, n-3p)             | 7.369            | 0.034 | 7.141 | 0.024 | 7.530            | 0.030 | 7.387 | 0.024 | 7.530            | 0.030 | 7.387 | 0.024 |
|              | 1A <sub>2</sub> (V, n- $\pi^*$ )      | 3.918            | 0.000 | 3.908 | 0.000 | 3.922            | 0.000 | 3.918 | 0.000 | 3.922            | 0.000 | 3.918 | 0.000 |
| Furane       | 2A <sub>2</sub> (R, n-3p)             | 7.936            | 0.000 | 7.410 | 0.000 | 7.990            | 0.000 | 7.668 | 0.000 | 7.990            | 0.000 | 7.668 | 0.000 |
|              | 1B <sub>1</sub> (R, $\pi$ -3p)        | 6.471            | 0.046 | 6.399 | 0.037 | 6.644            | 0.041 | 6.613 | 0.036 | 6.644            | 0.041 | 6.613 | 0.036 |
|              | 2B <sub>2</sub> (R, $\pi$ -3p)        | 7.398            | 0.009 | 6.744 | 0.013 | 7.293            | 0.007 | 6.896 | 0.000 | 7.293            | 0.007 | 6.896 | 0.000 |
|              | 1A <sub>2</sub> (R, $\pi$ -3s)        | 5.951            | 0.000 | 5.898 | 0.000 | 6.121            | 0.000 | 6.100 | 0.000 | 6.121            | 0.000 | 6.100 | 0.000 |
| Glyoxal      | 2A <sub>2</sub> (R, $\pi$ -3p)        | 6.654            | 0.000 | 6.548 | 0.000 | 6.818            | 0.000 | 6.764 | 0.000 | 6.818            | 0.000 | 6.764 | 0.000 |
|              | 1A <sub>u</sub> (V, n- $\pi^*$ )      | 2.832            | 0.000 | 2.827 | 0.000 | 2.831            | 0.000 | 2.828 | 0.000 | 2.831            | 0.000 | 2.828 | 0.000 |
|              | 1B <sub>g</sub> (V, n- $\pi^*$ )      | 4.281            | 0.000 | 4.273 | 0.000 | 4.274            | 0.000 | 4.271 | 0.000 | 4.274            | 0.000 | 4.271 | 0.000 |
| Ketene       | 2B <sub>g</sub> (V, n- $\pi^*$ )      | 6.472            | 0.000 | 6.419 | 0.000 | 6.497            | 0.000 | 6.476 | 0.000 | 6.497            | 0.000 | 6.476 | 0.000 |
|              | 2A <sub>1</sub> (V, $\pi$ - $\pi^*$ ) | 7.230            | 0.213 | 6.890 | 0.118 | 7.264            | 0.203 | 7.092 | 0.145 | 7.264            | 0.203 | 7.092 | 0.145 |
|              | 1B <sub>1</sub> (R, $\pi$ -3s)        | 5.822            | 0.033 | 5.796 | 0.031 | 6.026            | 0.032 | 6.017 | 0.031 | 6.026            | 0.032 | 6.017 | 0.031 |

| Molecule              | State                                  | AVDZ             |       |       | dAVDZ |                  |       | AVTZ  |       |                  | dAVTZ |       |       |
|-----------------------|----------------------------------------|------------------|-------|-------|-------|------------------|-------|-------|-------|------------------|-------|-------|-------|
|                       |                                        | $\Delta E_{0,n}$ | $f^l$ | $f^v$ | $f^m$ | $\Delta E_{0,n}$ | $f^l$ | $f^v$ | $f^m$ | $\Delta E_{0,n}$ | $f^l$ | $f^v$ | $f^m$ |
| Methylenecyclopropene | 2A <sub>2</sub> (R, $\pi$ -3p)         | 6.980            | 0.000 | 6.875 | 0.000 | 7.181            | 0.000 | 7.127 | 0.000 | 7.181            | 0.000 | 7.127 | 0.000 |
|                       | 1B <sub>1</sub> (R, $\pi$ -3s)         | 5.202            | 0.005 | 5.147 | 0.005 | 5.375            | 0.006 | 5.351 | 0.006 | 5.375            | 0.006 | 5.351 | 0.006 |
|                       | 1B <sub>2</sub> (V, $\pi$ - $\pi^*$ )  | 4.457            | 0.015 | 4.451 | 0.014 | 4.459            | 0.014 | 4.457 | 0.014 | 4.459            | 0.014 | 4.457 | 0.014 |
|                       | 1A <sub>2</sub> (R, $\pi$ -3p)         | 5.702            | 0.000 | 5.626 | 0.000 | 5.870            | 0.000 | 5.836 | 0.000 | 5.870            | 0.000 | 5.836 | 0.000 |
| Pyrazine              | 2A <sub>g</sub> (R, n-3s)              | 6.101            | 0.000 | 6.042 | 0.000 | 6.301            | 0.000 | 6.274 | 0.000 | 6.301            | 0.000 | 6.274 | 0.000 |
|                       | 1B <sub>1u</sub> (V, $\pi$ - $\pi^*$ ) | 6.863            | 0.005 | 6.964 | 0.130 | 6.878            | 0.068 | 6.871 | 0.054 | 6.878            | 0.068 | 6.871 | 0.054 |
|                       | 2B <sub>1u</sub> (R, n-3p)             | 7.005            | 0.138 | 6.750 | 0.003 | 7.109            | 0.080 | 7.039 | 0.085 | 7.109            | 0.080 | 7.039 | 0.085 |
|                       | 2B <sub>2u</sub> (R, n-3p)             | 6.633            | 0.038 | 6.557 | 0.034 | 6.839            | 0.037 | 6.800 | 0.034 | 6.839            | 0.037 | 6.800 | 0.034 |
| Pyridazine            | 1B <sub>3g</sub> (R, n.d.)             | 7.392            | 0.000 | 7.235 | 0.000 | 7.572            | 0.000 | 7.484 | 0.000 | 7.572            | 0.000 | 7.484 | 0.000 |
|                       | 2B <sub>1</sub> (V, n- $\pi^*$ )       | 6.377            | 0.005 | 6.371 | 0.005 | 6.346            | 0.005 | 6.343 | 0.005 | 6.346            | 0.005 | 6.343 | 0.005 |
|                       | 1A <sub>2</sub> (V, n- $\pi^*$ )       | 4.276            | 0.000 | 4.270 | 0.000 | 4.272            | 0.000 | 4.270 | 0.000 | 4.272            | 0.000 | 4.270 | 0.000 |
|                       | 1B <sub>1</sub> (R, mixed)             | 5.744            | 0.005 | 5.705 | 0.007 | 5.942            | 0.006 | 5.925 | 0.008 | 5.942            | 0.006 | 5.925 | 0.008 |
| Pyrrole               | 1A <sub>2</sub> (R, $\pi$ -3s)         | 5.118            | 0.000 | 5.083 | 0.000 | 5.296            | 0.000 | 5.283 | 0.000 | 5.296            | 0.000 | 5.283 | 0.000 |
|                       | 2A <sub>2</sub> (R, $\pi$ -3p)         | 5.860            | 0.000 | 5.769 | 0.000 | 6.026            | 0.000 | 5.983 | 0.000 | 6.026            | 0.000 | 5.983 | 0.000 |
|                       | 1A <sub>2</sub> (V, $\pi$ - $\pi^*$ )  | 2.367            | 0.000 | 2.367 | 0.000 | 2.371            | 0.000 | 2.371 | 0.000 | 2.371            | 0.000 | 2.371 | 0.000 |
|                       | 1B <sub>2</sub> (V, n- $\pi^*$ )       | 3.875            | 0.038 | 3.875 | 0.038 | 3.886            | 0.039 | 3.885 | 0.039 | 3.886            | 0.039 | 3.885 | 0.039 |
| Tetrazine             | 1B <sub>2g</sub> (V, n- $\pi^*$ )      | 5.759            | 0.000 | 5.756 | 0.000 | 5.677            | 0.000 | 5.676 | 0.000 | 5.677            | 0.000 | 5.676 | 0.000 |
|                       | 1B <sub>1g</sub> (V, n- $\pi^*$ )      | 5.125            | 0.000 | 5.121 | 0.000 | 5.043            | 0.000 | 5.042 | 0.000 | 5.043            | 0.000 | 5.042 | 0.000 |
|                       | 1B <sub>3u</sub> (V, n- $\pi^*$ )      | 2.465            | 0.006 | 2.462 | 0.006 | 2.423            | 0.006 | 2.421 | 0.006 | 2.423            | 0.006 | 2.421 | 0.006 |
|                       | 1A <sub>2</sub> (R, $\pi$ -3s)         | 5.990            | 0.000 | 5.932 | 0.000 | 6.146            | 0.000 | 6.121 | 0.000 | 6.146            | 0.000 | 6.121 | 0.000 |
| Thiophene             | 1B <sub>1</sub> (R, $\pi$ -3p)         | 6.200            | 0.021 | 6.165 | 0.019 | 6.243            | 0.014 | 6.233 | 0.014 | 6.243            | 0.014 | 6.233 | 0.014 |
|                       | 1A <sub>2</sub> (R, n-3p)              | 8.622            | 0.000 | 8.570 | 0.000 | 8.838            | 0.000 | 8.816 | 0.000 | 8.838            | 0.000 | 8.816 | 0.000 |
|                       | 1B <sub>1</sub> (R, n-3s)              | 6.967            | 0.055 | 6.943 | 0.049 | 7.181            | 0.052 | 7.173 | 0.049 | 7.181            | 0.052 | 7.173 | 0.049 |
|                       |                                        |                  |       |       |       |                  |       |       |       |                  |       |       |       |
| Water                 |                                        |                  |       |       |       |                  |       |       |       |                  |       |       |       |
|                       |                                        |                  |       |       |       |                  |       |       |       |                  |       |       |       |
|                       |                                        |                  |       |       |       |                  |       |       |       |                  |       |       |       |
|                       |                                        |                  |       |       |       |                  |       |       |       |                  |       |       |       |

## S2.4 Full testing set ISR-ADC(3), EOM-CCSD, LR-TDDFT and LR-TDA (dAVTZ)

Table S14: Ground state absorption data for ISR-ADC(3), B3LYP (full TDDFT), and CAM-B3LYP (full TDDFT).  $\Delta E_{0,n}$  [eV] and oscillator strengths in length, velocity gauges,  $f^l$ ,  $f^v$  respectively. Rydberg = R, valence = V. All data are obtained with dAVTZ basis set.

| Molecule        | State                           | ISR-ADC(3)       |       |                  | B3LYP |       |                  | CAMB3LYP |       |  |
|-----------------|---------------------------------|------------------|-------|------------------|-------|-------|------------------|----------|-------|--|
|                 |                                 | $\Delta E_{0,n}$ | $f^l$ | $\Delta E_{0,n}$ | $f^l$ | $f^v$ | $\Delta E_{0,n}$ | $f^l$    | $f^v$ |  |
| Acetone         | 2A <sub>1</sub> (R, n-3p)       | 7.885            | 0.001 | 6.444            | 0.002 | 0.002 | 7.288            | 0.000    | 0.000 |  |
|                 | 1B <sub>2</sub> (R, n-3s)       | 6.900            | 0.033 | 5.706            | 0.026 | 0.026 | 6.368            | 0.030    | 0.028 |  |
|                 | 2B <sub>2</sub> (R, n-3p)       | 7.881            | 0.001 | 6.585            | 0.004 | 0.004 | 7.314            | 0.002    | 0.001 |  |
|                 | 2A <sub>2</sub> (R, n-3p)       | 7.822            | 0.000 | 6.526            | 0.000 | 0.000 | 7.266            | 0.000    | 0.000 |  |
| Acrolein        | 1A'' (V, n- $\pi^*$ )           | 3.760            | 0.000 | 3.561            | 0.000 | 0.000 | 3.774            | 0.000    | 0.000 |  |
|                 | 2A'' (V, n- $\pi^*$ )           | 6.817            | 0.000 | 6.393            | 0.000 | 0.000 | 6.968            | 0.002    | 0.000 |  |
| Ammonia         | 1A <sub>2</sub> (R, n-3s)       | 6.628            | 0.082 | 5.897            | 0.068 | 0.068 | 6.196            | 0.073    | 0.072 |  |
|                 | 1E (R, n-3p)                    | 8.188            | 0.003 | 6.993            | 0.001 | 0.001 | 7.553            | 0.002    | 0.002 |  |
|                 | 2A <sub>1</sub> (R, n-3p)       | 8.659            | 0.000 | 7.279            | 0.000 | 0.000 | 7.943            | 0.000    | 0.000 |  |
|                 | 2A <sub>2</sub> (R, n-4s)       | 9.207            | 0.000 | 7.316            | 0.005 | 0.005 | 8.270            | 0.003    | 0.002 |  |
| Benzene         | 1E <sub>1g</sub> (R, $\pi$ -3s) | 6.363            | 0.000 | 5.969            | 0.000 | 0.000 | 6.430            | 0.000    | 0.000 |  |
|                 | 1E <sub>2u</sub> (R, $\pi$ -3p) | 6.971            | 0.000 | 6.450            | 0.000 | 0.000 | 7.005            | 0.000    | 0.000 |  |
|                 | 1A <sub>2u</sub> (R, $\pi$ -3p) | 6.891            | 0.064 | 6.427            | 0.039 | 0.040 | 6.910            | 0.054    | 0.058 |  |
|                 | 1B <sub>g</sub> (R, $\pi$ -3s)  | 6.102            | 0.000 | 5.610            | 0.000 | 0.000 | 6.014            | 0.000    | 0.000 |  |
| Butadiene       | 2B <sub>g</sub> (R, $\pi$ -3d)  | 7.242            | 0.000 | 6.420            | 0.000 | 0.000 | 7.068            | 0.000    | 0.000 |  |
|                 | 1A <sub>u</sub> (R, $\pi$ -3p)  | 6.421            | 0.001 | 5.869            | 0.000 | 0.000 | 6.294            | 0.001    | 0.001 |  |
| Carbon monoxide | 2A <sub>u</sub> (R, $\pi$ -3p)  | 6.572            | 0.047 | 5.927            | 0.028 | 0.028 | 6.441            | 0.039    | 0.042 |  |
|                 | 2 $\Sigma^+$ (R. n.d.)          | 10.531           | 0.007 | 9.809            | 0.001 | 0.001 | 10.377           | 0.011    | 0.008 |  |
|                 | 3 $\Sigma^+$ (R. n.d.)          | 11.139           | 0.117 | 10.148           | 0.047 | 0.047 | 10.817           | 0.074    | 0.085 |  |
|                 | 1 $\Pi$ (V, n- $\pi^*$ )        | 8.240            | 0.087 | 8.337            | 0.082 | 0.083 | 8.414            | 0.080    | 0.085 |  |
|                 | 2 $\Pi$ (R, n.d.)               | 11.284           | 0.025 | 10.205           | 0.008 | 0.008 | 10.916           | 0.021    | 0.023 |  |

| Molecule        | State                                 | ISR-ADC(3)       |       |       | B3LYP            |       |       | CAMB3LYP         |       |       |
|-----------------|---------------------------------------|------------------|-------|-------|------------------|-------|-------|------------------|-------|-------|
|                 |                                       | $\Delta E_{0,n}$ | $f^l$ | $f^v$ | $\Delta E_{0,n}$ | $f^l$ | $f^v$ | $\Delta E_{0,n}$ | $f^l$ | $f^v$ |
| Cyclopentadiene | 2A <sub>1</sub> (V, $\pi$ - $\pi^*$ ) | 5.923            | 0.000 | 0.000 | 6.202            | 0.000 | 0.000 | 6.825            | 0.000 | 0.000 |
|                 | 1A <sub>2</sub> (R, $\pi$ -3s)        | 5.613            | 0.000 | 0.000 | 5.052            | 0.000 | 0.000 | 5.519            | 0.000 | 0.000 |
|                 | 2A <sub>2</sub> (R, $\pi$ -3p)        | 6.270            | 0.000 | 0.000 | 5.554            | 0.000 | 0.000 | 6.141            | 0.000 | 0.000 |
|                 | 1B <sub>1</sub> (R, $\pi$ -3p)        | 6.218            | 0.035 | 0.021 | 5.543            | 0.021 | 0.021 | 6.083            | 0.029 | 0.031 |
|                 | 1B <sub>2</sub> (V, $\pi$ - $\pi^*$ ) | 5.346            | 0.089 | 0.079 | 4.981            | 0.079 | 0.079 | 5.125            | 0.083 | 0.084 |
| Cyclopropene    | 2B <sub>2</sub> (R, $\pi$ -3p)        | 6.296            | 0.041 | 0.029 | 5.655            | 0.029 | 0.029 | 6.177            | 0.035 | 0.036 |
|                 | 2B <sub>1</sub> (R, $\pi$ -3s)        | 6.793            | 0.009 | 0.003 | 6.053            | 0.003 | 0.003 | 6.487            | 0.006 | 0.007 |
|                 | 3B <sub>1</sub> (R, $\pi$ -3p)        | 7.163            | 0.025 | 0.007 | 6.388            | 0.007 | 0.007 | 6.840            | 0.020 | 0.023 |
| Diazirine       | 1B <sub>1</sub> (V, n- $\pi^*$ )      | 3.820            | 0.002 | 0.002 | 3.890            | 0.002 | 0.002 | 3.886            | 0.001 | 0.002 |
|                 | 1B <sub>2</sub> (R, n-3s)             | 7.332            | 0.002 | 0.000 | 6.713            | 0.000 | 0.000 | 7.114            | 0.008 | 0.004 |
| Diazomethane    | 2A <sub>1</sub> (V, $\pi$ - $\pi^*$ ) | 7.901            | 0.116 | 0.058 | 7.269            | 0.058 | 0.058 | 7.695            | 0.098 | 0.094 |
|                 | 1B <sub>1</sub> (R, $\pi$ -3s)        | 5.214            | 0.014 | 0.015 | 5.084            | 0.015 | 0.015 | 5.321            | 0.015 | 0.014 |
| Formaldehyde    | 1A <sub>2</sub> (V, $\pi$ - $\pi^*$ ) | 2.743            | 0.000 | 0.000 | 2.997            | 0.000 | 0.000 | 2.972            | 0.000 | 0.000 |
|                 | 2A <sub>1</sub> (R, n-3p)             | 8.563            | 0.055 | 0.024 | 7.118            | 0.024 | 0.024 | 7.711            | 0.037 | 0.038 |
|                 | 1B <sub>2</sub> (R, n-3s)             | 7.613            | 0.019 | 0.022 | 6.410            | 0.022 | 0.022 | 6.870            | 0.023 | 0.017 |
|                 | 2B <sub>2</sub> (R, n-3p)             | 8.362            | 0.042 | 0.015 | 7.145            | 0.015 | 0.015 | 7.610            | 0.026 | 0.030 |
|                 | 1A <sub>2</sub> (V, n- $\pi^*$ )      | 3.902            | 0.000 | 0.000 | 3.914            | 0.000 | 0.000 | 3.913            | 0.000 | 0.000 |
| Furane          | 2A <sub>2</sub> (R, n-3p)             | 8.764            | 0.000 | 0.000 | 7.313            | 0.000 | 0.000 | 7.914            | 0.000 | 0.000 |
|                 | 1B <sub>1</sub> (R, $\pi$ -3p)        | 6.471            | 0.036 | 0.021 | 5.870            | 0.021 | 0.021 | 6.386            | 0.030 | 0.033 |
|                 | 2B <sub>2</sub> (R, $\pi$ -3p)        | 6.742            | 0.001 | 0.015 | 6.231            | 0.015 | 0.015 | 6.682            | 0.000 | 0.000 |
| Glyoxal         | 1A <sub>2</sub> (R, $\pi$ -3s)        | 5.934            | 0.000 | 0.000 | 5.453            | 0.000 | 0.000 | 5.894            | 0.000 | 0.000 |
|                 | 2A <sub>2</sub> (R, $\pi$ -3p)        | 6.630            | 0.000 | 0.000 | 5.982            | 0.000 | 0.000 | 6.556            | 0.000 | 0.000 |
|                 | 1A <sub>u</sub> (V, n- $\pi^*$ )      | 2.824            | 0.000 | 0.000 | 2.539            | 0.000 | 0.000 | 2.728            | 0.000 | 0.000 |
|                 | 1B <sub>g</sub> (V, n- $\pi^*$ )      | 4.224            | 0.000 | 0.000 | 4.052            | 0.000 | 0.000 | 4.236            | 0.000 | 0.000 |
|                 | 2B <sub>g</sub> (V, n- $\pi^*$ )      | 6.790            | 0.000 | 0.000 | 5.946            | 0.000 | 0.000 | 6.528            | 0.000 | 0.000 |
| Ketene          | 2A <sub>1</sub> (V, $\pi$ - $\pi^*$ ) | 7.009            | 0.121 | 0.036 | 6.503            | 0.036 | 0.036 | 6.939            | 0.078 | 0.078 |

| Molecule              | State                                  | ISR-ADC(3)       |       |       | B3LYP            |       |       | CAMB3LYP         |       |       |
|-----------------------|----------------------------------------|------------------|-------|-------|------------------|-------|-------|------------------|-------|-------|
|                       |                                        | $\Delta E_{0,n}$ | $f^l$ | $f^l$ | $\Delta E_{0,n}$ | $f^l$ | $f^v$ | $\Delta E_{0,n}$ | $f^l$ | $f^v$ |
| Methylenecyclopropene | 1B <sub>1</sub> (R, $\pi$ -3s)         | 5.867            | 0.035 | 0.031 | 5.570            | 0.031 | 0.031 | 5.845            | 0.036 | 0.033 |
|                       | 2A <sub>2</sub> (R, $\pi$ -3p)         | 7.020            | 0.000 | 0.000 | 6.414            | 0.000 | 0.000 | 6.871            | 0.000 | 0.000 |
|                       | 1B <sub>1</sub> (R, $\pi$ -3s)         | 5.238            | 0.005 | 0.001 | 4.805            | 0.001 | 0.001 | 5.246            | 0.004 | 0.007 |
|                       | 1B <sub>2</sub> (V, $\pi$ - $\pi^*$ )  | 4.179            | 0.012 | 0.010 | 3.964            | 0.010 | 0.010 | 4.416            | 0.016 | 0.013 |
|                       | 1A <sub>2</sub> (R, $\pi$ -3p)         | 5.751            | 0.000 | 0.000 | 5.188            | 0.000 | 0.000 | 5.724            | 0.000 | 0.000 |
| Pyrazine              | 2A <sub>g</sub> (R, n-3s)              | 6.938            | 0.000 | 0.000 | 6.074            | 0.000 | 0.000 | 6.703            | 0.000 | 0.000 |
|                       | 1B <sub>1u</sub> (V, $\pi$ - $\pi^*$ ) | 6.655            | 0.065 | 0.049 | 6.455            | 0.049 | 0.049 | 6.556            | 0.055 | 0.062 |
|                       | 2B <sub>1u</sub> (R, n-3p)             | 7.566            | 0.296 | 0.031 | 6.714            | 0.031 | 0.031 | 7.365            | 0.326 | 0.130 |
|                       | 2B <sub>2u</sub> (R, n-3p)             | 7.548            | 0.025 | 0.036 | 6.468            | 0.036 | 0.036 | 7.255            | 0.029 | 0.039 |
| Pyridazine            | 1B <sub>3g</sub> (R, n.d.)             | 8.225            | 0.000 | 0.000 | 7.023            | 0.000 | 0.000 | 7.903            | 0.000 | 0.000 |
|                       | 2B <sub>1</sub> (V, n- $\pi^*$ )       | 6.617            | 0.004 | 0.004 | 6.119            | 0.004 | 0.004 | 6.481            | 0.004 | 0.005 |
| Pyrrole               | 1A <sub>2</sub> (V, n- $\pi^*$ )       | 4.604            | 0.000 | 0.000 | 4.129            | 0.000 | 0.000 | 4.498            | 0.000 | 0.000 |
|                       | 1B <sub>1</sub> (R, mixed)             | 5.870            | 0.025 | 0.019 | 5.340            | 0.019 | 0.019 | 5.842            | 0.026 | 0.027 |
| Silylidene            | 1A <sub>2</sub> (R, $\pi$ -3s)         | 5.133            | 0.000 | 0.000 | 4.677            | 0.000 | 0.000 | 5.137            | 0.000 | 0.000 |
|                       | 2A <sub>2</sub> (R, $\pi$ -3p)         | 5.878            | 0.000 | 0.000 | 5.337            | 0.000 | 0.000 | 5.863            | 0.000 | 0.000 |
|                       | 1A <sub>2</sub> (V, $\pi$ - $\pi^*$ )  | 1.877            | 0.000 | 0.000 | 2.174            | 0.000 | 0.000 | 2.223            | 0.000 | 0.000 |
|                       | 1B <sub>2</sub> (V, n- $\pi^*$ )       | 3.885            | 0.039 | 0.035 | 3.788            | 0.035 | 0.033 | 3.803            | 0.042 | 0.035 |
| Tetrazine             | 1B <sub>2g</sub> (V, n- $\pi^*$ )      | 5.133            | 0.000 | 0.000 | 5.464            | 0.000 | 0.000 | 5.753            | 0.000 | 0.000 |
|                       | 1B <sub>1g</sub> (V, n- $\pi^*$ )      | 4.970            | 0.000 | 0.000 | 4.720            | 0.000 | 0.000 | 5.004            | 0.000 | 0.000 |
| Thiophene             | 1B <sub>3u</sub> (V, n- $\pi^*$ )      | 2.415            | 0.007 | 0.004 | 2.236            | 0.004 | 0.005 | 2.452            | 0.006 | 0.006 |
|                       | 1A <sub>2</sub> (R, $\pi$ -3s)         | 6.008            | 0.000 | 0.000 | 5.595            | 0.000 | 0.000 | 6.049            | 0.000 | 0.000 |
| Water                 | 1B <sub>1</sub> (R, $\pi$ -3p)         | 6.019            | 0.010 | 0.012 | 5.746            | 0.012 | 0.012 | 6.183            | 0.015 | 0.012 |
|                       | 1A <sub>2</sub> (R, n-3p)              | 9.621            | 0.000 | 0.000 | 8.223            | 0.000 | 0.000 | 8.682            | 0.000 | 0.000 |
|                       | 1B <sub>1</sub> (R, n-3s)              | 7.839            | 0.052 | 0.044 | 6.886            | 0.044 | 0.044 | 7.124            | 0.044 | 0.046 |

Table S15: Ground state absorption data for LC-BLYP33 (full TDDFT), and LC-BLYP47 (full TDDFT).

| Molecule        | State                                 | LC-BLYP33        |       |       |                  | LC-BLYP47 |       |       |       |
|-----------------|---------------------------------------|------------------|-------|-------|------------------|-----------|-------|-------|-------|
|                 |                                       | $\Delta E_{0,n}$ | $f^l$ | $f^v$ | $\Delta E_{0,n}$ | $f^l$     | $f^v$ | $f^l$ | $f^v$ |
| Acetone         | 2A <sub>1</sub> (R, n-3p)             | 7.365            | 0.002 | 0.002 | 8.189            | 0.000     | 0.008 | 0.000 | 0.008 |
|                 | 1B <sub>2</sub> (R, n-3s)             | 6.289            | 0.027 | 0.027 | 7.081            | 0.030     | 0.028 | 0.030 | 0.028 |
|                 | 2B <sub>2</sub> (R, n-3p)             | 7.328            | 0.001 | 0.001 | 8.146            | 0.002     | 0.001 | 0.002 | 0.001 |
|                 | 2A <sub>2</sub> (R, n-3p)             | 7.229            | 0.000 | 0.000 | 8.043            | 0.000     | 0.000 | 0.000 | 0.000 |
| Acrolein        | 1A'' (V, n- $\pi^*$ )                 | 3.717            | 0.000 | 0.000 | 3.920            | 0.000     | 0.000 | 0.000 | 0.000 |
|                 | 2A'' (V, n- $\pi^*$ )                 | 6.900            | 0.000 | 0.000 | 7.518            | 0.002     | 0.000 | 0.002 | 0.000 |
| Ammonia         | 1A <sub>2</sub> (R, n-3s)             | 6.049            | 0.071 | 0.071 | 6.676            | 0.073     | 0.074 | 0.073 | 0.074 |
|                 | 1E (R, n-3p)                          | 7.491            | 0.001 | 0.001 | 8.216            | 0.002     | 0.001 | 0.002 | 0.001 |
| Benzene         | 2A <sub>1</sub> (R, n-3p)             | 7.964            | 0.000 | 0.000 | 8.729            | 0.000     | 0.001 | 0.000 | 0.001 |
|                 | 2A <sub>2</sub> (R, n-4s)             | 8.479            | 0.000 | 0.000 | 9.297            | 0.003     | 0.000 | 0.003 | 0.000 |
|                 | 1E <sub>1g</sub> (R, $\pi$ -3s)       | 6.633            | 0.000 | 0.000 | 6.977            | 0.000     | 0.000 | 0.000 | 0.000 |
|                 | 1E <sub>2u</sub> (R, $\pi$ -3p)       | 7.280            | 0.000 | 0.000 | 7.644            | 0.000     | 0.000 | 0.000 | 0.000 |
| Butadiene       | 1A <sub>2u</sub> (R, $\pi$ -3p)       | 7.129            | 0.068 | 0.068 | 7.458            | 0.054     | 0.073 | 0.054 | 0.073 |
|                 | 1B <sub>g</sub> (R, $\pi$ -3s)        | 6.177            | 0.000 | 0.000 | 6.550            | 0.000     | 0.000 | 0.000 | 0.000 |
|                 | 2B <sub>g</sub> (R, $\pi$ -3d)        | 7.348            | 0.000 | 0.000 | 7.749            | 0.000     | 0.000 | 0.000 | 0.000 |
|                 | 1A <sub>u</sub> (R, $\pi$ -3p)        | 6.472            | 0.002 | 0.002 | 6.861            | 0.001     | 0.004 | 0.001 | 0.004 |
| Carbon monoxide | 2A <sub>u</sub> (R, $\pi$ -3p)        | 6.678            | 0.050 | 0.050 | 7.069            | 0.039     | 0.053 | 0.039 | 0.053 |
|                 | 2 $\Sigma^+$ (R, n.d.)                | 10.271           | 0.011 | 0.011 | 11.085           | 0.011     | 0.026 | 0.011 | 0.026 |
|                 | 3 $\Sigma^+$ (R, n.d.)                | 10.732           | 0.108 | 0.108 | 11.594           | 0.074     | 0.120 | 0.074 | 0.120 |
|                 | 1 $\Pi$ (V, n- $\pi^*$ )              | 8.373            | 0.088 | 0.089 | 8.501            | 0.080     | 0.085 | 0.080 | 0.085 |
| Cyclopentadiene | 2 $\Pi$ (R, n.d.)                     | 10.853           | 0.032 | 0.032 | 11.712           | 0.021     | 0.043 | 0.021 | 0.043 |
|                 | 2A <sub>1</sub> (V, $\pi$ - $\pi^*$ ) | 6.961            | 0.002 | 0.002 | 7.432            | 0.000     | 0.000 | 0.000 | 0.000 |
|                 | 1A <sub>2</sub> (R, $\pi$ -3s)        | 5.723            | 0.000 | 0.000 | 6.093            | 0.000     | 0.000 | 0.000 | 0.000 |

| Molecule     | State                                 | LC-BLYP33        |       |       |                  | LC-BLYP47 |       |       |       |
|--------------|---------------------------------------|------------------|-------|-------|------------------|-----------|-------|-------|-------|
|              |                                       | $\Delta E_{0,n}$ | $f^l$ | $f^v$ | $\Delta E_{0,n}$ | $f^l$     | $f^v$ | $f^l$ | $f^v$ |
| Cyclopropene | 2A <sub>2</sub> (R, $\pi$ -3p)        | 6.435            | 0.000 | 0.000 | 6.840            | 0.000     | 0.000 | 0.000 | 0.000 |
|              | 1B <sub>1</sub> (R, $\pi$ -3p)        | 6.335            | 0.036 | 0.037 | 6.706            | 0.029     | 0.039 | 0.029 | 0.039 |
|              | 1B <sub>2</sub> (V, $\pi$ - $\pi^*$ ) | 5.211            | 0.087 | 0.086 | 5.308            | 0.083     | 0.087 | 0.083 | 0.087 |
|              | 2B <sub>2</sub> (R, $\pi$ -3p)        | 6.400            | 0.038 | 0.038 | 6.780            | 0.035     | 0.039 | 0.035 | 0.039 |
|              | 2B <sub>1</sub> (R, $\pi$ -3s)        | 6.581            | 0.006 | 0.006 | 7.036            | 0.006     | 0.007 | 0.006 | 0.007 |
| Diazirine    | 3B <sub>1</sub> (R, $\pi$ -3p)        | 6.961            | 0.026 | 0.026 | 7.414            | 0.020     | 0.026 | 0.020 | 0.026 |
|              | 1B <sub>1</sub> (V, $n$ - $\pi^*$ )   | 3.840            | 0.002 | 0.002 | 3.873            | 0.001     | 0.002 | 0.001 | 0.002 |
|              | 1B <sub>2</sub> (R, $n$ -3s)          | 7.094            | 0.009 | 0.009 | 7.492            | 0.008     | 0.025 | 0.008 | 0.025 |
| Diazomethane | 2A <sub>1</sub> (V, $\pi$ - $\pi^*$ ) | 7.669            | 0.101 | 0.102 | 8.189            | 0.098     | 0.135 | 0.098 | 0.135 |
|              | 1B <sub>1</sub> (R, $\pi$ -3s)        | 5.285            | 0.013 | 0.013 | 5.669            | 0.015     | 0.014 | 0.015 | 0.014 |
|              | 1A <sub>2</sub> (V, $\pi$ - $\pi^*$ ) | 2.955            | 0.000 | 0.000 | 2.927            | 0.000     | 0.000 | 0.000 | 0.000 |
| Formaldehyde | 2A <sub>1</sub> (R, $n$ -3p)          | 7.559            | 0.043 | 0.043 | 8.336            | 0.037     | 0.054 | 0.037 | 0.054 |
|              | 1B <sub>2</sub> (R, $n$ -3s)          | 6.668            | 0.011 | 0.011 | 7.398            | 0.023     | 0.012 | 0.023 | 0.012 |
|              | 2B <sub>2</sub> (R, $n$ -3p)          | 7.432            | 0.040 | 0.040 | 8.172            | 0.026     | 0.046 | 0.026 | 0.046 |
|              | 1A <sub>2</sub> (V, $n$ - $\pi^*$ )   | 3.778            | 0.000 | 0.000 | 3.894            | 0.000     | 0.000 | 0.000 | 0.000 |
| Furane       | 2A <sub>2</sub> (R, $n$ -3p)          | 7.730            | 0.000 | 0.000 | 8.535            | 0.000     | 0.000 | 0.000 | 0.000 |
|              | 1B <sub>1</sub> (R, $\pi$ -3p)        | 6.609            | 0.039 | 0.040 | 6.995            | 0.030     | 0.043 | 0.030 | 0.043 |
|              | 2B <sub>2</sub> (R, $\pi$ -3p)        | 6.887            | 0.002 | 0.002 | 7.252            | 0.000     | 0.009 | 0.000 | 0.009 |
|              | 1A <sub>2</sub> (R, $\pi$ -3s)        | 6.073            | 0.000 | 0.000 | 6.449            | 0.000     | 0.000 | 0.000 | 0.000 |
| Glyoxal      | 2A <sub>2</sub> (R, $\pi$ -3p)        | 6.823            | 0.000 | 0.000 | 7.241            | 0.000     | 0.000 | 0.000 | 0.000 |
|              | 1A <sub>u</sub> (V, $n$ - $\pi^*$ )   | 2.673            | 0.000 | 0.000 | 2.891            | 0.000     | 0.000 | 0.000 | 0.000 |
|              | 1B <sub>g</sub> (V, $n$ - $\pi^*$ )   | 4.172            | 0.000 | 0.000 | 4.356            | 0.000     | 0.000 | 0.000 | 0.000 |
|              | 2B <sub>g</sub> (V, $n$ - $\pi^*$ )   | 6.416            | 0.000 | 0.000 | 7.253            | 0.000     | 0.000 | 0.000 | 0.000 |
| Ketene       | 2A <sub>1</sub> (V, $\pi$ - $\pi^*$ ) | 6.954            | 0.097 | 0.096 | 7.334            | 0.078     | 0.153 | 0.078 | 0.153 |
|              | 1B <sub>1</sub> (R, $\pi$ -3s)        | 5.799            | 0.030 | 0.030 | 6.259            | 0.036     | 0.033 | 0.036 | 0.033 |
|              | 2A <sub>2</sub> (R, $\pi$ -3p)        | 6.900            | 0.000 | 0.000 | 7.429            | 0.000     | 0.000 | 0.000 | 0.000 |



| Molecule              | State                                  | LC-BLYP33        |       |       |                  | LC-BLYP47 |       |       |       |
|-----------------------|----------------------------------------|------------------|-------|-------|------------------|-----------|-------|-------|-------|
|                       |                                        | $\Delta E_{0,n}$ | $f^l$ | $f^v$ | $\Delta E_{0,n}$ | $f^l$     | $f^v$ | $f^l$ | $f^v$ |
| Methylenecyclopropene | 1B <sub>1</sub> (R, $\pi$ -3s)         | 5.389            | 0.011 | 0.011 | 5.750            | 0.004     | 0.012 | 0.004 | 0.012 |
|                       | 1B <sub>2</sub> (V, $\pi$ - $\pi^*$ )  | 4.558            | 0.014 | 0.014 | 4.971            | 0.016     | 0.020 | 0.016 | 0.020 |
|                       | 1A <sub>2</sub> (R, $\pi$ -3p)         | 5.935            | 0.000 | 0.000 | 6.333            | 0.000     | 0.000 | 0.000 | 0.000 |
| Pyrazine              | 2A <sub>g</sub> (R, n-3s)              | 6.651            | 0.000 | 0.000 | 7.420            | 0.000     | 0.000 | 0.000 | 0.000 |
|                       | 1B <sub>1u</sub> (V, $\pi$ - $\pi^*$ ) | 6.628            | 0.068 | 0.068 | 6.624            | 0.055     | 0.068 | 0.055 | 0.068 |
|                       | 2B <sub>1u</sub> (R, n-3p)             | 7.311            | 0.159 | 0.158 | 7.842            | 0.326     | 0.463 | 0.326 | 0.463 |
|                       | 2B <sub>2u</sub> (R, n-3p)             | 7.338            | 0.043 | 0.042 | 8.074            | 0.029     | 0.313 | 0.029 | 0.313 |
| Pyridazine            | 1B <sub>3g</sub> (R, n.d.)             | 7.964            | 0.000 | 0.000 | 8.772            | 0.000     | 0.000 | 0.000 | 0.000 |
|                       | 2B <sub>1</sub> (V, n- $\pi^*$ )       | 6.343            | 0.005 | 0.005 | 6.854            | 0.004     | 0.005 | 0.004 | 0.005 |
|                       | 1A <sub>2</sub> (V, n- $\pi^*$ )       | 4.365            | 0.000 | 0.000 | 4.858            | 0.000     | 0.000 | 0.000 | 0.000 |
| Pyrrole               | 1B <sub>1</sub> (R, mixed)             | 6.055            | 0.028 | 0.028 | 6.430            | 0.026     | 0.034 | 0.026 | 0.034 |
|                       | 1A <sub>2</sub> (R, $\pi$ -3s)         | 5.333            | 0.000 | 0.000 | 5.726            | 0.000     | 0.000 | 0.000 | 0.000 |
|                       | 2A <sub>2</sub> (R, $\pi$ -3p)         | 6.096            | 0.000 | 0.000 | 6.483            | 0.000     | 0.000 | 0.000 | 0.000 |
| Silylidene            | 1A <sub>2</sub> (V, $\pi$ - $\pi^*$ )  | 2.234            | 0.000 | 0.000 | 2.320            | 0.000     | 0.000 | 0.000 | 0.000 |
|                       | 1B <sub>2</sub> (V, n- $\pi^*$ )       | 3.692            | 0.033 | 0.032 | 3.800            | 0.042     | 0.035 | 0.042 | 0.035 |
|                       | 1B <sub>2g</sub> (V, n- $\pi^*$ )      | 5.736            | 0.000 | 0.000 | 6.041            | 0.000     | 0.000 | 0.000 | 0.000 |
| Tetrazine             | 1B <sub>1g</sub> (V, n- $\pi^*$ )      | 4.900            | 0.000 | 0.000 | 5.176            | 0.000     | 0.000 | 0.000 | 0.000 |
|                       | 1B <sub>3u</sub> (V, n- $\pi^*$ )      | 2.391            | 0.005 | 0.006 | 2.630            | 0.006     | 0.008 | 0.006 | 0.008 |
|                       | 1A <sub>2</sub> (R, $\pi$ -3s)         | 6.229            | 0.000 | 0.000 | 6.466            | 0.000     | 0.000 | 0.000 | 0.000 |
| Thiophene             | 1B <sub>1</sub> (R, $\pi$ -3p)         | 6.372            | 0.012 | 0.012 | 6.766            | 0.015     | 0.013 | 0.015 | 0.013 |
|                       | 1A <sub>2</sub> (R, n-3p)              | 8.485            | 0.000 | 0.000 | 9.275            | 0.000     | 0.000 | 0.000 | 0.000 |
|                       | 1B <sub>1</sub> (R, n-3s)              | 6.861            | 0.047 | 0.047 | 7.541            | 0.044     | 0.048 | 0.044 | 0.048 |

Table S16: Ground state absorption data for BHandHLYP (full TDDFT), BHandHLYP (TDA) and EOM-CCSD.

| Molecule        | State                                 | BHandHLYP        |       |       | BHandHLYP (TDA)  |       |       | EOM-CCSD         |  |
|-----------------|---------------------------------------|------------------|-------|-------|------------------|-------|-------|------------------|--|
|                 |                                       | $\Delta E_{0,n}$ | $f^l$ | $f^v$ | $\Delta E_{0,n}$ | $f^l$ | $f^v$ | $\Delta E_{0,n}$ |  |
| Acetone         | 2A <sub>1</sub> (R, n-3p)             | 7.714            | 0.000 | 0.000 | 7.723            | 0.000 | 0.000 | 7.585            |  |
|                 | 1B <sub>2</sub> (R, n-3s)             | 6.861            | 0.030 | 0.030 | 6.865            | 0.031 | 0.033 | 6.575            |  |
|                 | 2B <sub>2</sub> (R, n-3p)             | 7.774            | 0.002 | 0.002 | 7.777            | 0.002 | 0.001 | 7.564            |  |
|                 | 2A <sub>2</sub> (R, n-3p)             | 7.730            | 0.000 | 0.000 | 7.732            | 0.000 | 0.000 | 7.485            |  |
| Acrolein        | 1A'' (V, n- $\pi^*$ )                 | 3.989            | 0.000 | 0.000 | 4.048            | 0.000 | 0.002 | 3.911            |  |
|                 | 2A'' (V, n- $\pi^*$ )                 | 7.489            | 0.002 | 0.002 | 7.507            | 0.004 | 0.007 | 7.254            |  |
| Ammonia         | 1A <sub>2</sub> (R, n-3s)             | 6.594            | 0.073 | 0.073 | 6.610            | 0.077 | 0.070 | 6.601            |  |
|                 | 1E (R, n-3p)                          | 7.937            | 0.002 | 0.002 | 7.943            | 0.003 | 0.000 | 8.120            |  |
| Benzene         | 2A <sub>1</sub> (R, n-3p)             | 8.319            | 0.000 | 0.000 | 8.340            | 0.000 | 0.002 | 8.566            |  |
|                 | 2A <sub>2</sub> (R, n-4s)             | 8.545            | 0.003 | 0.003 | 8.547            | 0.003 | 0.003 | 9.109            |  |
|                 | 1E <sub>1g</sub> (R, $\pi$ -3s)       | 6.370            | 0.000 | 0.000 | 6.372            | 0.000 | 0.000 | 6.559            |  |
|                 | 1E <sub>2u</sub> (R, $\pi$ -3p)       | 6.914            | 0.000 | 0.000 | 6.916            | 0.000 | 0.000 | 7.165            |  |
| Butadiene       | 1A <sub>2u</sub> (R, $\pi$ -3p)       | 6.829            | 0.054 | 0.054 | 6.833            | 0.057 | 0.039 | 7.090            |  |
|                 | 1B <sub>g</sub> (R, $\pi$ -3s)        | 5.973            | 0.000 | 0.000 | 5.976            | 0.000 | 0.000 | 6.387            |  |
|                 | 2B <sub>g</sub> (R, $\pi$ -3d)        | 6.963            | 0.000 | 0.000 | 6.964            | 0.000 | 0.000 | 7.517            |  |
|                 | 1A <sub>u</sub> (R, $\pi$ -3p)        | 6.257            | 0.001 | 0.001 | 6.259            | 0.001 | 0.002 | 6.704            |  |
| Carbon monoxide | 2A <sub>u</sub> (R, $\pi$ -3p)        | 6.367            | 0.039 | 0.039 | 6.370            | 0.041 | 0.034 | 6.863            |  |
|                 | 2 $\Sigma^+$ (R, n.d.)                | 10.862           | 0.011 | 0.011 | 10.888           | 0.010 | 0.012 | 10.962           |  |
|                 | 3 $\Sigma^+$ (R, n.d.)                | 11.310           | 0.074 | 0.074 | 11.313           | 0.077 | 0.075 | 11.568           |  |
|                 | 1 $\Pi$ (V, n- $\pi^*$ )              | 8.512            | 0.080 | 0.081 | 8.738            | 0.106 | 0.017 | 8.583            |  |
| Cyclopentadiene | 2 $\Pi$ (R, n.d.)                     | 11.396           | 0.021 | 0.020 | 11.401           | 0.019 | 0.022 | 11.702           |  |
|                 | 2A <sub>1</sub> (V, $\pi$ - $\pi^*$ ) | 6.740            | 0.000 | 0.000 | 6.746            | 0.000 | 0.000 | 6.954            |  |
|                 | 1A <sub>2</sub> (R, $\pi$ -3s)        | 5.459            | 0.000 | 0.000 | 5.461            | 0.000 | 0.000 | 5.829            |  |

| Molecule     | State                                 | BHandHLYP        |       |       | BHandHLYP (TDA)  |       |       | EOM-CCSD         |  |
|--------------|---------------------------------------|------------------|-------|-------|------------------|-------|-------|------------------|--|
|              |                                       | $\Delta E_{0,n}$ | $f^1$ | $f^v$ | $\Delta E_{0,n}$ | $f^1$ | $f^v$ | $\Delta E_{0,n}$ |  |
| Cyclopropene | 2A <sub>2</sub> (R, $\pi$ -3p)        | 6.043            | 0.000 | 0.000 | 6.044            | 0.000 | 0.000 | 6.476            |  |
|              | 1B <sub>1</sub> (R, $\pi$ -3p)        | 5.990            | 0.029 | 0.029 | 5.993            | 0.030 | 0.022 | 6.429            |  |
|              | 1B <sub>2</sub> (V, $\pi$ - $\pi^*$ ) | 5.113            | 0.083 | 0.083 | 5.439            | 0.126 | 0.003 | 5.667            |  |
|              | 2B <sub>2</sub> (R, $\pi$ -3p)        | 6.104            | 0.035 | 0.035 | 6.109            | 0.040 | 0.022 | 6.502            |  |
|              | 2B <sub>1</sub> (R, $\pi$ -3s)        | 6.538            | 0.006 | 0.006 | 6.541            | 0.006 | 0.004 | 6.976            |  |
|              | 3B <sub>1</sub> (R, $\pi$ -3p)        | 6.889            | 0.020 | 0.021 | 6.895            | 0.020 | 0.033 | 7.354            |  |
| Diazirine    | 1B <sub>1</sub> (V, $\pi$ - $\pi^*$ ) | 3.942            | 0.001 | 0.002 | 4.022            | 0.002 | 0.008 | 4.183            |  |
|              | 1B <sub>2</sub> (R, $\pi$ -3s)        | 7.308            | 0.008 | 0.007 | 7.374            | 0.001 | 0.009 | 7.544            |  |
| Diazomethane | 2A <sub>1</sub> (V, $\pi$ - $\pi^*$ ) | 7.930            | 0.098 | 0.098 | 7.965            | 0.101 | 0.035 | 8.047            |  |
|              | 1B <sub>1</sub> (R, $\pi$ -3s)        | 5.434            | 0.015 | 0.015 | 5.439            | 0.016 | 0.014 | 5.556            |  |
|              | 1A <sub>2</sub> (V, $\pi$ - $\pi^*$ ) | 2.965            | 0.000 | 0.000 | 3.042            | 0.000 | 0.000 | 3.192            |  |
|              | 2A <sub>1</sub> (R, $\pi$ -3p)        | 8.255            | 0.037 | 0.037 | 8.261            | 0.040 | 0.031 | 8.170            |  |
| Formaldehyde | 1B <sub>2</sub> (R, $\pi$ -3s)        | 7.415            | 0.023 | 0.023 | 7.421            | 0.024 | 0.017 | 7.224            |  |
|              | 2B <sub>2</sub> (R, $\pi$ -3p)        | 8.151            | 0.026 | 0.026 | 8.157            | 0.028 | 0.029 | 8.027            |  |
|              | 1A <sub>2</sub> (V, $\pi$ - $\pi^*$ ) | 4.081            | 0.000 | 0.000 | 4.143            | 0.000 | 0.000 | 4.011            |  |
|              | 2A <sub>2</sub> (R, $\pi$ -3p)        | 8.469            | 0.000 | 0.000 | 8.470            | 0.000 | 0.000 | 8.393            |  |
| Furane       | 1B <sub>1</sub> (R, $\pi$ -3p)        | 6.310            | 0.030 | 0.030 | 6.313            | 0.031 | 0.025 | 6.684            |  |
|              | 2B <sub>2</sub> (R, $\pi$ -3p)        | 6.610            | 0.000 | 0.000 | 6.692            | 0.019 | 0.008 | 6.970            |  |
|              | 1A <sub>2</sub> (R, $\pi$ -3s)        | 5.844            | 0.000 | 0.000 | 5.846            | 0.000 | 0.000 | 6.151            |  |
|              | 2A <sub>2</sub> (R, $\pi$ -3p)        | 6.469            | 0.000 | 0.000 | 6.471            | 0.000 | 0.000 | 6.844            |  |
| Glyoxal      | 1A <sub>u</sub> (V, $\pi$ - $\pi^*$ ) | 2.930            | 0.000 | 0.000 | 2.997            | 0.000 | 0.005 | 3.008            |  |
|              | 1B <sub>g</sub> (V, $\pi$ - $\pi^*$ ) | 4.426            | 0.000 | 0.000 | 4.494            | 0.000 | 0.000 | 4.416            |  |
|              | 2B <sub>g</sub> (V, $\pi$ - $\pi^*$ ) | 7.226            | 0.000 | 0.000 | 7.238            | 0.000 | 0.000 | 7.105            |  |
| Ketene       | 2A <sub>1</sub> (V, $\pi$ - $\pi^*$ ) | 7.112            | 0.078 | 0.077 | 7.151            | 0.069 | 0.026 | 7.213            |  |
|              | 1B <sub>1</sub> (R, $\pi$ -3s)        | 6.021            | 0.036 | 0.036 | 6.030            | 0.038 | 0.026 | 6.087            |  |
|              | 2A <sub>2</sub> (R, $\pi$ -3p)        | 7.031            | 0.000 | 0.000 | 7.034            | 0.000 | 0.000 | 7.246            |  |

| Molecule              | State                                  | BHandHLYP        |       |       | BHandHLYP (TDA)  |       |       | EOM-CCSD         |  |
|-----------------------|----------------------------------------|------------------|-------|-------|------------------|-------|-------|------------------|--|
|                       |                                        | $\Delta E_{0,n}$ | $f^1$ | $f^v$ | $\Delta E_{0,n}$ | $f^1$ | $f^v$ | $\Delta E_{0,n}$ |  |
| Methylenecyclopropene | 1B <sub>1</sub> (R, $\pi$ -3s)         | 5.207            | 0.004 | 0.004 | 5.210            | 0.005 | 0.003 | 5.461            |  |
|                       | 1B <sub>2</sub> (V, $\pi$ - $\pi^*$ )  | 4.555            | 0.016 | 0.016 | 4.676            | 0.021 | 0.009 | 4.582            |  |
|                       | 1A <sub>2</sub> (R, $\pi$ -3p)         | 5.660            | 0.000 | 0.000 | 5.662            | 0.000 | 0.000 | 5.971            |  |
| Pyrazine              | 2A <sub>g</sub> (R, n-3s)              | 7.147            | 0.000 | 0.000 | 7.150            | 0.000 | 0.000 | 6.811            |  |
|                       | 1B <sub>1u</sub> (V, $\pi$ - $\pi^*$ ) | 6.503            | 0.055 | 0.055 | 6.760            | 0.059 | 0.008 | 6.956            |  |
|                       | 2B <sub>1u</sub> (R, n-3p)             | 7.705            | 0.326 | 0.324 | 7.807            | 0.131 | 0.031 | 7.548            |  |
|                       | 2B <sub>2u</sub> (R, n-3p)             | 7.652            | 0.029 | 0.028 | 7.655            | 0.033 | 0.026 | 7.414            |  |
|                       | 1B <sub>3g</sub> (R, n.d.)             | 8.284            | 0.000 | 0.000 | 8.284            | 0.000 | 0.000 | 8.100            |  |
| Pyridazine            | 2B <sub>1</sub> (V, n- $\pi^*$ )       | 6.999            | 0.004 | 0.004 | 7.027            | 0.006 | 0.000 | 6.666            |  |
|                       | 1A <sub>2</sub> (V, n- $\pi^*$ )       | 4.977            | 0.000 | 0.000 | 5.033            | 0.000 | 0.000 | 4.652            |  |
| Pyrrole               | 1B <sub>1</sub> (R, mixed)             | 5.770            | 0.026 | 0.027 | 5.773            | 0.028 | 0.020 | 6.022            |  |
|                       | 1A <sub>2</sub> (R, $\pi$ -3s)         | 5.101            | 0.000 | 0.000 | 5.103            | 0.000 | 0.000 | 5.331            |  |
| Silylidene            | 2A <sub>2</sub> (R, $\pi$ -3p)         | 5.794            | 0.000 | 0.000 | 5.796            | 0.000 | 0.000 | 6.053            |  |
|                       | 1A <sub>2</sub> (V, $\pi$ - $\pi^*$ )  | 2.248            | 0.000 | 0.000 | 2.269            | 0.000 | 0.000 | 2.288            |  |
|                       | 1B <sub>2</sub> (V, n- $\pi^*$ )       | 3.949            | 0.042 | 0.040 | 4.091            | 0.058 | 0.001 | 3.877            |  |
| Tetrazine             | 1B <sub>2g</sub> (V, n- $\pi^*$ )      | 5.978            | 0.000 | 0.000 | 6.071            | 0.000 | 0.000 | 5.835            |  |
|                       | 1B <sub>1g</sub> (V, n- $\pi^*$ )      | 5.330            | 0.000 | 0.000 | 5.456            | 0.000 | 0.000 | 5.264            |  |
|                       | 1B <sub>3u</sub> (V, n- $\pi^*$ )      | 2.704            | 0.006 | 0.007 | 2.813            | 0.010 | 0.063 | 2.634            |  |
| Thiophene             | 1A <sub>2</sub> (R, $\pi$ -3s)         | 6.010            | 0.000 | 0.000 | 6.013            | 0.000 | 0.000 | 6.199            |  |
|                       | 1B <sub>1</sub> (R, $\pi$ -3p)         | 6.189            | 0.015 | 0.015 | 6.204            | 0.016 | 0.022 | 6.301            |  |
| Water                 | 1A <sub>2</sub> (R, n-3p)              | 9.242            | 0.000 | 0.000 | 9.252            | 0.000 | 0.000 | 9.349            |  |
|                       | 1B <sub>1</sub> (R, n-3s)              | 7.667            | 0.044 | 0.045 | 7.689            | 0.046 | 0.059 | 7.593            |  |

Table S17: Ground state absorption data for B3LYP (TDA), and CAM-B3LYP (full TDA).

| Molecule        | State                                 | B3LYP (TDA)      |       |       |                  | CAM-B3LYP (TDA) |       |       |       |
|-----------------|---------------------------------------|------------------|-------|-------|------------------|-----------------|-------|-------|-------|
|                 |                                       | $\Delta E_{0,n}$ | $f^l$ | $f^v$ | $\Delta E_{0,n}$ | $f^l$           | $f^v$ | $f^l$ | $f^v$ |
| Acetone         | 2A <sub>1</sub> (R, n-3p)             | 6.451            | 0.002 | 0.001 | 7.296            | 0.000           | 0.000 | 0.000 | 0.000 |
|                 | 1B <sub>2</sub> (R, n-3s)             | 5.709            | 0.027 | 0.026 | 6.372            | 0.029           | 0.031 | 0.029 | 0.031 |
|                 | 2B <sub>2</sub> (R, n-3p)             | 6.586            | 0.004 | 0.003 | 7.316            | 0.002           | 0.001 | 0.002 | 0.001 |
|                 | 2A <sub>2</sub> (R, n-3p)             | 6.527            | 0.000 | 0.000 | 7.266            | 0.000           | 0.000 | 0.000 | 0.000 |
| Acrolein        | 1A'' (V, n- $\pi^*$ )                 | 3.585            | 0.000 | 0.002 | 3.808            | 0.000           | 0.002 | 0.000 | 0.002 |
|                 | 2A'' (V, n- $\pi^*$ )                 | 6.402            | 0.001 | 0.000 | 6.981            | 0.000           | 0.001 | 0.000 | 0.001 |
| Ammonia         | 1A <sub>2</sub> (R, n-3s)             | 5.911            | 0.072 | 0.060 | 6.212            | 0.075           | 0.070 | 0.075 | 0.070 |
|                 | 1E (R, n-3p)                          | 6.995            | 0.002 | 0.000 | 7.556            | 0.002           | 0.000 | 0.002 | 0.000 |
|                 | 2A <sub>1</sub> (R, n-3p)             | 7.291            | 0.001 | 0.000 | 7.969            | 0.000           | 0.002 | 0.000 | 0.002 |
| Benzene         | 2A <sub>2</sub> (R, n-4s)             | 7.321            | 0.004 | 0.007 | 8.273            | 0.002           | 0.003 | 0.002 | 0.003 |
|                 | 1E <sub>1g</sub> (R, $\pi$ -3s)       | 5.969            | 0.000 | 0.000 | 6.430            | 0.000           | 0.000 | 0.000 | 0.000 |
|                 | 1E <sub>2u</sub> (R, $\pi$ -3p)       | 6.450            | 0.000 | 0.000 | 7.005            | 0.000           | 0.000 | 0.000 | 0.000 |
|                 | 1A <sub>2u</sub> (R, $\pi$ -3p)       | 6.427            | 0.039 | 0.040 | 6.910            | 0.057           | 0.058 | 0.057 | 0.058 |
| Butadiene       | 1B <sub>g</sub> (R, $\pi$ -3s)        | 5.611            | 0.000 | 0.000 | 6.016            | 0.000           | 0.000 | 0.000 | 0.000 |
|                 | 2B <sub>g</sub> (R, $\pi$ -3d)        | 6.420            | 0.000 | 0.000 | 7.069            | 0.000           | 0.000 | 0.000 | 0.000 |
|                 | 1A <sub>u</sub> (R, $\pi$ -3p)        | 5.870            | 0.001 | 0.001 | 6.295            | 0.001           | 0.002 | 0.001 | 0.002 |
|                 | 2A <sub>u</sub> (R, $\pi$ -3p)        | 5.928            | 0.029 | 0.027 | 6.444            | 0.043           | 0.039 | 0.043 | 0.039 |
| Carbon monoxide | 2 $\Sigma^+$ (R, n.d.)                | 9.829            | 0.001 | 0.002 | 10.407           | 0.007           | 0.009 | 0.007 | 0.009 |
|                 | 3 $\Sigma^+$ (R, n.d.)                | 10.150           | 0.048 | 0.047 | 10.821           | 0.088           | 0.085 | 0.088 | 0.085 |
|                 | 1 $\Pi$ (V, n- $\pi^*$ )              | 8.542            | 0.107 | 0.018 | 8.629            | 0.110           | 0.018 | 0.110 | 0.018 |
| Cyclopentadiene | 2 $\Pi$ (R, n.d.)                     | 10.211           | 0.006 | 0.010 | 10.923           | 0.021           | 0.026 | 0.021 | 0.026 |
|                 | 2A <sub>1</sub> (V, $\pi$ - $\pi^*$ ) | 6.205            | 0.000 | 0.000 | 6.839            | 0.000           | 0.000 | 0.000 | 0.000 |
|                 | 1A <sub>2</sub> (R, $\pi$ -3s)        | 5.053            | 0.000 | 0.000 | 5.520            | 0.000           | 0.000 | 0.000 | 0.000 |

| Molecule     | State                                 | B3LYP (TDA)      |       |       | CAM-B3LYP (TDA)  |       |       |
|--------------|---------------------------------------|------------------|-------|-------|------------------|-------|-------|
|              |                                       | $\Delta E_{0,n}$ | $f^l$ | $f^v$ | $\Delta E_{0,n}$ | $f^l$ | $f^v$ |
| Cyclopropene | 2A <sub>2</sub> (R, $\pi$ -3p)        | 5.554            | 0.000 | 0.000 | 6.142            | 0.000 | 0.000 |
|              | 1B <sub>1</sub> (R, $\pi$ -3p)        | 5.544            | 0.021 | 0.016 | 6.085            | 0.032 | 0.025 |
|              | 1B <sub>2</sub> (V, $\pi$ - $\pi^*$ ) | 5.335            | 0.118 | 0.008 | 5.477            | 0.132 | 0.003 |
|              | 2B <sub>2</sub> (R, $\pi$ -3p)        | 5.660            | 0.040 | 0.014 | 6.181            | 0.040 | 0.025 |
| Diazirine    | 2B <sub>1</sub> (R, $\pi$ -3s)        | 6.055            | 0.003 | 0.002 | 6.496            | 0.000 | 0.003 |
|              | 3B <sub>1</sub> (R, $\pi$ -3p)        | 6.404            | 0.003 | 0.019 | 6.846            | 0.023 | 0.036 |
|              | 1B <sub>1</sub> (V, n- $\pi^*$ )      | 3.953            | 0.002 | 0.008 | 3.955            | 0.003 | 0.008 |
|              | 1B <sub>2</sub> (R, n-3s)             | 6.726            | 0.000 | 0.007 | 7.165            | 0.001 | 0.008 |
| Diazomethane | 2A <sub>1</sub> (V, $\pi$ - $\pi^*$ ) | 7.290            | 0.060 | 0.020 | 7.728            | 0.097 | 0.033 |
|              | 1B <sub>1</sub> (R, $\pi$ -3s)        | 5.088            | 0.015 | 0.014 | 5.326            | 0.015 | 0.014 |
|              | 1A <sub>2</sub> (V, $\pi$ - $\pi^*$ ) | 3.015            | 0.000 | 0.000 | 3.012            | 0.000 | 0.000 |
|              | 2A <sub>1</sub> (R, n-3p)             | 7.122            | 0.025 | 0.019 | 7.717            | 0.042 | 0.032 |
| Formaldehyde | 1B <sub>2</sub> (R, n-3s)             | 6.415            | 0.024 | 0.015 | 6.875            | 0.019 | 0.012 |
|              | 2B <sub>2</sub> (R, n-3p)             | 7.148            | 0.016 | 0.016 | 7.616            | 0.032 | 0.032 |
|              | 1A <sub>2</sub> (V, n- $\pi^*$ )      | 3.940            | 0.000 | 0.000 | 3.947            | 0.000 | 0.000 |
|              | 2A <sub>2</sub> (R, n-3p)             | 7.313            | 0.000 | 0.000 | 7.914            | 0.000 | 0.000 |
| Furane       | 1B <sub>1</sub> (R, $\pi$ -3p)        | 5.871            | 0.021 | 0.019 | 6.388            | 0.034 | 0.029 |
|              | 2B <sub>2</sub> (R, $\pi$ -3p)        | 6.395            | 0.075 | 0.001 | 6.769            | 0.016 | 0.010 |
|              | 1A <sub>2</sub> (R, $\pi$ -3s)        | 5.453            | 0.000 | 0.000 | 5.895            | 0.000 | 0.000 |
|              | 2A <sub>2</sub> (R, $\pi$ -3p)        | 5.983            | 0.000 | 0.000 | 6.557            | 0.000 | 0.000 |
| Glyoxal      | 1A <sub>u</sub> (V, n- $\pi^*$ )      | 2.571            | 0.000 | 0.007 | 2.770            | 0.000 | 0.005 |
|              | 1B <sub>g</sub> (V, n- $\pi^*$ )      | 4.080            | 0.000 | 0.000 | 4.272            | 0.000 | 0.000 |
|              | 2B <sub>g</sub> (V, n- $\pi^*$ )      | 5.951            | 0.000 | 0.000 | 6.534            | 0.000 | 0.000 |
|              | 2A <sub>1</sub> (V, $\pi$ - $\pi^*$ ) | 6.521            | 0.034 | 0.013 | 6.980            | 0.071 | 0.026 |
| Ketene       | 1B <sub>1</sub> (R, $\pi$ -3s)        | 5.577            | 0.032 | 0.023 | 5.853            | 0.035 | 0.025 |
|              | 2A <sub>2</sub> (R, $\pi$ -3p)        | 6.415            | 0.000 | 0.000 | 6.872            | 0.000 | 0.000 |

| Molecule              | State                                  | B3LYP (TDA)      |       |       | CAM-B3LYP (TDA)  |       |       |
|-----------------------|----------------------------------------|------------------|-------|-------|------------------|-------|-------|
|                       |                                        | $\Delta E_{0,n}$ | $f^l$ | $f^v$ | $\Delta E_{0,n}$ | $f^l$ | $f^v$ |
| Methylenecyclopropene | 1B <sub>1</sub> (R, $\pi$ -3s)         | 4.807            | 0.001 | 0.000 | 5.248            | 0.007 | 0.005 |
|                       | 1B <sub>2</sub> (V, $\pi$ - $\pi^*$ )  | 4.077            | 0.014 | 0.016 | 4.542            | 0.018 | 0.012 |
|                       | 1A <sub>2</sub> (R, $\pi$ -3p)         | 5.189            | 0.000 | 0.000 | 5.726            | 0.000 | 0.000 |
| Pyrazine              | 2A <sub>g</sub> (R, n-3s)              | 6.076            | 0.000 | 0.000 | 6.707            | 0.000 | 0.000 |
|                       | 1B <sub>1u</sub> (V, $\pi$ - $\pi^*$ ) | 6.656            | 0.004 | 0.000 | 6.820            | 0.055 | 0.005 |
|                       | 2B <sub>1u</sub> (R, n-3p)             | 6.790            | 0.077 | 0.014 | 7.401            | 0.110 | 0.037 |
|                       | 2B <sub>2u</sub> (R, n-3p)             | 6.471            | 0.039 | 0.024 | 7.258            | 0.043 | 0.031 |
|                       | 1B <sub>3g</sub> (R, n.d.)             | 7.023            | 0.000 | 0.000 | 7.904            | 0.000 | 0.000 |
| Pyridazine            | 2B <sub>1</sub> (V, n- $\pi^*$ )       | 6.134            | 0.006 | 0.000 | 6.504            | 0.006 | 0.000 |
|                       | 1A <sub>2</sub> (V, n- $\pi^*$ )       | 4.154            | 0.000 | 0.000 | 4.533            | 0.000 | 0.000 |
| Pyrrole               | 1B <sub>1</sub> (R, mixed)             | 5.341            | 0.020 | 0.016 | 5.844            | 0.028 | 0.021 |
|                       | 1A <sub>2</sub> (R, $\pi$ -3s)         | 4.678            | 0.000 | 0.000 | 5.138            | 0.000 | 0.000 |
| Silylidene            | 2A <sub>2</sub> (R, $\pi$ -3p)         | 5.338            | 0.000 | 0.000 | 5.864            | 0.000 | 0.000 |
|                       | 1A <sub>2</sub> (V, $\pi$ - $\pi^*$ )  | 2.183            | 0.000 | 0.000 | 2.240            | 0.000 | 0.000 |
|                       | 1B <sub>2</sub> (V, n- $\pi^*$ )       | 3.927            | 0.049 | 0.001 | 3.946            | 0.051 | 0.001 |
| Tetrazine             | 1B <sub>2g</sub> (V, n- $\pi^*$ )      | 5.500            | 0.000 | 0.000 | 5.807            | 0.000 | 0.000 |
|                       | 1B <sub>1g</sub> (V, n- $\pi^*$ )      | 4.809            | 0.000 | 0.000 | 5.111            | 0.000 | 0.000 |
|                       | 1B <sub>3u</sub> (V, n- $\pi^*$ )      | 2.313            | 0.008 | 0.076 | 2.543            | 0.009 | 0.071 |
| Thiophene             | 1A <sub>2</sub> (R, $\pi$ -3s)         | 5.596            | 0.000 | 0.000 | 6.050            | 0.000 | 0.000 |
|                       | 1B <sub>1</sub> (R, $\pi$ -3p)         | 5.754            | 0.013 | 0.020 | 6.198            | 0.013 | 0.023 |
| Water                 | 1A <sub>2</sub> (R, n-3p)              | 8.224            | 0.000 | 0.000 | 8.684            | 0.000 | 0.000 |
|                       | 1B <sub>1</sub> (R, n-3s)              | 6.900            | 0.045 | 0.052 | 7.142            | 0.047 | 0.058 |

Table S18: Ground state absorption data for LC-BLYP33 (TDA), and LC-BLYP47 (full TDA).

| Molecule        | State                                 | LC-BLYP33 (TDA)  |       |       | LC-BLYP47 (TDA)  |       |       |
|-----------------|---------------------------------------|------------------|-------|-------|------------------|-------|-------|
|                 |                                       | $\Delta E_{0,n}$ | $f^l$ | $f^v$ | $\Delta E_{0,n}$ | $f^l$ | $f^v$ |
| Acetone         | 2A <sub>1</sub> (R, n-3p)             | 7.375            | 0.003 | 0.001 | 8.200            | 0.007 | 0.003 |
|                 | 1B <sub>2</sub> (R, n-3s)             | 6.296            | 0.028 | 0.031 | 7.089            | 0.029 | 0.035 |
|                 | 2B <sub>2</sub> (R, n-3p)             | 7.331            | 0.001 | 0.000 | 8.150            | 0.001 | 0.000 |
|                 | 2A <sub>2</sub> (R, n-3p)             | 7.230            | 0.000 | 0.000 | 8.044            | 0.000 | 0.000 |
| Acrolein        | 1A'' (V, n- $\pi^*$ )                 | 3.751            | 0.000 | 0.002 | 3.969            | 0.000 | 0.002 |
|                 | 2A'' (V, n- $\pi^*$ )                 | 6.915            | 0.000 | 0.001 | 7.546            | 0.000 | 0.002 |
| Ammonia         | 1A <sub>2</sub> (R, n-3s)             | 6.067            | 0.075 | 0.072 | 6.697            | 0.077 | 0.080 |
|                 | 1E (R, n-3p)                          | 7.494            | 0.001 | 0.000 | 8.221            | 0.001 | 0.000 |
|                 | 2A <sub>1</sub> (R, n-3p)             | 8.000            | 0.000 | 0.003 | 8.766            | 0.001 | 0.003 |
| Benzene         | 2A <sub>2</sub> (R, n-4s)             | 8.483            | 0.000 | 0.001 | 9.303            | 0.000 | 0.000 |
|                 | 1E <sub>1g</sub> (R, $\pi$ -3s)       | 6.635            | 0.000 | 0.000 | 6.979            | 0.000 | 0.000 |
|                 | 1E <sub>2u</sub> (R, $\pi$ -3p)       | 7.281            | 0.000 | 0.000 | 7.645            | 0.000 | 0.000 |
|                 | 1A <sub>2u</sub> (R, $\pi$ -3p)       | 7.132            | 0.072 | 0.055 | 7.461            | 0.077 | 0.058 |
| Butadiene       | 1B <sub>g</sub> (R, $\pi$ -3s)        | 6.179            | 0.000 | 0.000 | 6.554            | 0.000 | 0.000 |
|                 | 2B <sub>g</sub> (R, $\pi$ -3d)        | 7.349            | 0.000 | 0.000 | 7.751            | 0.000 | 0.000 |
|                 | 1A <sub>u</sub> (R, $\pi$ -3p)        | 6.474            | 0.002 | 0.003 | 6.864            | 0.004 | 0.004 |
|                 | 2A <sub>u</sub> (R, $\pi$ -3p)        | 6.682            | 0.052 | 0.048 | 7.074            | 0.056 | 0.049 |
| Carbon monoxide | 2 $\Sigma^+$ (R, n.d.)                | 10.312           | 0.010 | 0.013 | 11.128           | 0.025 | 0.025 |
|                 | 3 $\Sigma^+$ (R, n.d.)                | 10.738           | 0.114 | 0.107 | 11.601           | 0.127 | 0.120 |
|                 | 1 $\Pi$ (V, n- $\pi^*$ )              | 8.595            | 0.116 | 0.020 | 8.734            | 0.112 | 0.017 |
| Cyclopentadiene | 2 $\Pi$ (R, n.d.)                     | 10.863           | 0.029 | 0.035 | 11.720           | 0.042 | 0.044 |
|                 | 2A <sub>1</sub> (V, $\pi$ - $\pi^*$ ) | 6.986            | 0.002 | 0.000 | 7.465            | 0.000 | 0.000 |
|                 | 1A <sub>2</sub> (R, $\pi$ -3s)        | 5.725            | 0.000 | 0.000 | 6.096            | 0.000 | 0.000 |



| Molecule     | State                                 | LC-BLYP33 (TDA)  |       |       | LC-BLYP47 (TDA)  |       |       |
|--------------|---------------------------------------|------------------|-------|-------|------------------|-------|-------|
|              |                                       | $\Delta E_{0,n}$ | $f^l$ | $f^v$ | $\Delta E_{0,n}$ | $f^l$ | $f^v$ |
| Cyclopropene | 2A <sub>2</sub> (R, $\pi$ -3p)        | 6.436            | 0.000 | 0.000 | 6.842            | 0.000 | 0.000 |
|              | 1B <sub>1</sub> (R, $\pi$ -3p)        | 6.337            | 0.038 | 0.032 | 6.709            | 0.041 | 0.033 |
|              | 1B <sub>2</sub> (V, $\pi$ - $\pi^*$ ) | 5.579            | 0.139 | 0.002 | 5.660            | 0.135 | 0.001 |
|              | 2B <sub>2</sub> (R, $\pi$ -3p)        | 6.407            | 0.039 | 0.029 | 6.787            | 0.041 | 0.030 |
|              | 2B <sub>1</sub> (R, $\pi$ -3s)        | 6.584            | 0.006 | 0.003 | 7.041            | 0.008 | 0.004 |
| Diazirine    | 3B <sub>1</sub> (R, $\pi$ -3p)        | 6.969            | 0.025 | 0.041 | 7.423            | 0.026 | 0.042 |
|              | 1B <sub>1</sub> (V, n- $\pi^*$ )      | 3.914            | 0.003 | 0.009 | 3.956            | 0.003 | 0.009 |
|              | 1B <sub>2</sub> (R, n-3s)             | 7.171            | 0.003 | 0.007 | 7.683            | 0.014 | 0.009 |
| Diazomethane | 2A <sub>1</sub> (V, $\pi$ - $\pi^*$ ) | 7.705            | 0.107 | 0.037 | 8.238            | 0.141 | 0.050 |
|              | 1B <sub>1</sub> (R, $\pi$ -3s)        | 5.292            | 0.014 | 0.013 | 5.677            | 0.014 | 0.013 |
|              | 1A <sub>2</sub> (V, $\pi$ - $\pi^*$ ) | 2.997            | 0.000 | 0.000 | 3.013            | 0.000 | 0.000 |
| Formaldehyde | 2A <sub>1</sub> (R, n-3p)             | 7.565            | 0.047 | 0.036 | 8.344            | 0.059 | 0.044 |
|              | 1B <sub>2</sub> (R, n-3s)             | 6.673            | 0.012 | 0.007 | 7.404            | 0.013 | 0.008 |
|              | 2B <sub>2</sub> (R, n-3p)             | 7.441            | 0.042 | 0.042 | 8.184            | 0.048 | 0.050 |
|              | 1A <sub>2</sub> (V, n- $\pi^*$ )      | 3.811            | 0.000 | 0.000 | 3.941            | 0.000 | 0.000 |
| Furane       | 2A <sub>2</sub> (R, n-3p)             | 7.730            | 0.000 |       | 8.536            | 0.000 | 0.000 |
|              | 1B <sub>1</sub> (R, $\pi$ -3p)        | 6.611            | 0.041 | 0.037 | 6.998            | 0.045 | 0.038 |
|              | 2B <sub>2</sub> (R, $\pi$ -3p)        | 6.966            | 0.005 | 0.015 | 7.296            | 0.001 | 0.020 |
|              | 1A <sub>2</sub> (R, $\pi$ -3s)        | 6.075            | 0.000 | 0.000 | 6.452            | 0.000 | 0.000 |
| Glyoxal      | 2A <sub>2</sub> (R, $\pi$ -3p)        | 6.824            | 0.000 | 0.000 | 7.243            | 0.000 | 0.000 |
|              | 1A <sub>u</sub> (V, n- $\pi^*$ )      | 2.715            | 0.000 | 0.005 | 2.948            | 0.000 | 0.004 |
|              | 1B <sub>g</sub> (V, n- $\pi^*$ )      | 4.206            | 0.000 | 0.000 | 4.403            | 0.000 | 0.000 |
|              | 2B <sub>g</sub> (V, n- $\pi^*$ )      | 6.422            | 0.000 | 0.000 | 7.263            | 0.000 | 0.000 |
| Ketene       | 2A <sub>1</sub> (V, $\pi$ - $\pi^*$ ) | 7.007            | 0.089 | 0.032 | 7.432            | 0.143 | 0.051 |
|              | 1B <sub>1</sub> (R, $\pi$ -3s)        | 5.811            | 0.033 | 0.024 | 6.272            | 0.036 | 0.026 |
|              | 2A <sub>2</sub> (R, $\pi$ -3p)        | 6.901            | 0.000 | 0.000 | 7.431            | 0.000 | 0.000 |

| Molecule              | State                                  | LC-BLYP33 (TDA)  |       |       | LC-BLYP47 (TDA)  |       |       |
|-----------------------|----------------------------------------|------------------|-------|-------|------------------|-------|-------|
|                       |                                        | $\Delta E_{0,n}$ | $f^l$ | $f^v$ | $\Delta E_{0,n}$ | $f^l$ | $f^v$ |
| Methylenecyclopropene | 1B <sub>1</sub> (R, $\pi$ -3s)         | 5.393            | 0.012 | 0.009 | 5.755            | 0.013 | 0.011 |
|                       | 1B <sub>2</sub> (V, $\pi$ - $\pi^*$ )  | 4.697            | 0.019 | 0.013 | 5.120            | 0.026 | 0.008 |
|                       | 1A <sub>2</sub> (R, $\pi$ -3p)         | 5.937            | 0.000 | 0.000 | 6.335            | 0.000 | 0.000 |
|                       | 2A <sub>g</sub> (R, n-3s)              | 6.657            | 0.000 | 0.000 | 7.427            | 0.000 | 0.000 |
| Pyrazine              | 1B <sub>1u</sub> (V, $\pi$ - $\pi^*$ ) | 6.899            | 0.048 | 0.002 | 6.910            | 0.069 | 0.008 |
|                       | 2B <sub>1u</sub> (R, n-3p)             | 7.360            | 0.168 | 0.061 | 8.049            | 0.308 | 0.076 |
|                       | 2B <sub>2u</sub> (R, n-3p)             | 7.341            | 0.048 | 0.034 | 8.151            | 0.047 | 0.035 |
|                       | 1B <sub>3g</sub> (R, n.d.)             | 7.966            | 0.000 | 0.000 | 8.774            | 0.000 | 0.000 |
| Pyridazine            | 2B <sub>1</sub> (V, n- $\pi^*$ )       | 6.370            | 0.007 | 0.000 | 6.891            | 0.007 | 0.000 |
|                       | 1A <sub>2</sub> (V, n- $\pi^*$ )       | 4.399            | 0.000 | 0.000 | 4.910            | 0.000 | 0.000 |
| Pyrrole               | 1B <sub>1</sub> (R, mixed)             | 6.058            | 0.030 | 0.023 | 6.433            | 0.035 | 0.027 |
|                       | 1A <sub>2</sub> (R, $\pi$ -3s)         | 5.334            | 0.000 | 0.000 | 5.728            | 0.000 | 0.000 |
| Silylidene            | 2A <sub>2</sub> (R, $\pi$ -3p)         | 6.097            | 0.000 | 0.000 | 6.485            | 0.000 | 0.000 |
|                       | 1A <sub>2</sub> (V, $\pi$ - $\pi^*$ )  | 2.257            | 0.000 | 0.000 | 2.353            | 0.000 | 0.000 |
| Tetrazine             | 1B <sub>2</sub> (V, n- $\pi^*$ )       | 3.841            | 0.048 | 0.000 | 3.947            | 0.053 | 0.001 |
|                       | 1B <sub>2g</sub> (V, n- $\pi^*$ )      | 5.780            | 0.000 | 0.000 | 6.121            | 0.000 | 0.000 |
|                       | 1B <sub>1g</sub> (V, n- $\pi^*$ )      | 5.010            | 0.000 | 0.000 | 5.305            | 0.000 | 0.000 |
|                       | 1B <sub>3u</sub> (V, n- $\pi^*$ )      | 2.487            | 0.009 | 0.073 | 2.746            | 0.011 | 0.067 |
| Thiophene             | 1A <sub>2</sub> (R, $\pi$ -3s)         | 6.231            | 0.000 | 0.000 | 6.499            | 0.000 | 0.000 |
|                       | 1B <sub>1</sub> (R, $\pi$ -3p)         | 6.392            | 0.013 | 0.025 | 6.793            | 0.015 | 0.025 |
| Water                 | 1A <sub>2</sub> (R, n-3p)              | 8.487            | 0.000 | 0.000 | 9.279            | 0.000 | 0.000 |
|                       | 1B <sub>1</sub> (R, n-3s)              | 6.884            | 0.049 | 0.059 | 7.570            | 0.049 | 0.065 |

## S3 Excited state absorption data

### S3.1 Transition dipole moments, small set of transitions

Table S19: Excited State absorption data. Transition dipole moments obtained with QR-CC3 and eight different basis sets: AVDZ, dAVDZ, tAVDZ, AVTZ, dAVTZ, tAVTZ, AVQZ, dAVQZ.

| Molecule        | State1          | State2          | AVDZ  | dAVDZ | tAVDZ | AVTZ  | dAVTZ | tAVTZ | AVQZ  | dAVQZ |
|-----------------|-----------------|-----------------|-------|-------|-------|-------|-------|-------|-------|-------|
| Ammonia         | 1A <sub>2</sub> | 1E              | 2.837 | 2.930 | 2.929 | 2.865 | 2.907 | 2.907 | 2.874 | 2.901 |
|                 | 1A <sub>2</sub> | 2A <sub>1</sub> | 2.003 | 2.479 | 2.472 | 2.218 | 2.457 | 2.451 | 2.340 | 2.451 |
|                 | 1E              | 2A <sub>2</sub> | 2.113 | 2.483 | 2.282 | 2.312 | 2.376 | 2.209 | 2.378 | 2.333 |
| Carbon monoxide | 2A <sub>1</sub> | 2A <sub>2</sub> | 0.323 | 4.137 | 4.745 | 1.140 | 4.297 | 4.790 | 1.817 | 4.394 |
|                 | 2Σ <sup>+</sup> | 3Σ <sup>+</sup> | 1.469 | 3.157 | 3.175 | 2.046 | 3.133 | 3.137 | 2.405 | 3.130 |
|                 | 2Σ <sup>+</sup> | 2Π              | 2.573 | 3.807 | 3.808 | 2.804 | 3.765 | 3.781 | 2.985 | 3.760 |
|                 | 2Π              | 1Π              | 0.434 | 0.401 | 0.380 | 0.407 | 0.374 | 0.368 | 0.398 | 0.369 |
|                 | 1B <sub>1</sub> | 2A <sub>1</sub> | 0.401 | 0.398 | 0.398 | 0.388 | 0.383 | 0.383 | 0.383 | 0.378 |
| Diazirine       | 1B <sub>2</sub> | 2A <sub>1</sub> | 2.275 | 2.737 | 2.734 | 2.297 | 2.551 | 2.548 | 2.313 | 2.471 |
| Silylidene      | 1A <sub>2</sub> | 1B <sub>2</sub> | 0.282 | 0.284 | 0.274 | 0.274 | 0.274 | 0.274 | 0.274 | 0.274 |
| Water           | 1B <sub>1</sub> | 1A <sub>2</sub> | 2.591 | 2.582 | 2.582 | 2.570 | 2.554 | 2.555 | 2.558 | 2.547 |

### S3.2 Small set of transitions, large basis sets

Table S20: Excited State absorption data for QR-CC3/dAVQZ and QR-CCSD/dAVQZ calculations.  $\Delta E_{m,n}$ [eV] and oscillator strengths in length, velocity, and mixed gauges,  $f^l$ ,  $f^v$ , and  $f^m$ , respectively.

| molecule        | State1          | State2          | QR-CC3/dAVQZ     |       |       |        | QR-CCSD/dAVQZ    |       |       |        |
|-----------------|-----------------|-----------------|------------------|-------|-------|--------|------------------|-------|-------|--------|
|                 |                 |                 | $\Delta E_{m,n}$ | $f^l$ | $f^v$ | $f^m$  | $\Delta E_{m,n}$ | $f^l$ | $f^v$ | $f^m$  |
| Ammonia         | 1A <sub>2</sub> | 1E              | 1.547            | 0.319 | 0.321 | 0.320  | 1.522            | 0.322 | 0.324 | 0.324  |
|                 | 1A <sub>2</sub> | 2A <sub>1</sub> | 1.995            | 0.294 | 0.295 | 0.294  | 1.969            | 0.295 | 0.292 | 0.294  |
|                 | 1E              | 2A <sub>2</sub> | 1.006            | 0.134 | 0.137 | 0.136  | 0.993            | 0.136 | 0.138 | 0.137  |
|                 | 2A <sub>1</sub> | 2A <sub>2</sub> | 0.558            | 0.264 | 0.284 | 0.274  | 0.546            | 0.261 | 0.282 | 0.272  |
| Carbon monoxide | 2 $\Sigma^+$    | 3 $\Sigma^+$    | 0.609            | 0.146 | 0.146 | 0.146  | 0.607            | 0.146 | 0.145 | 0.147  |
|                 | 2 $\Sigma^+$    | 2 $\Pi$         | 0.737            | 0.255 | 0.261 | 0.258  | 0.739            | 0.253 | 0.259 | 0.258  |
|                 | 2 $\Pi$         | 1 $\Pi$         | 2.986            | 0.010 | 0.009 | 0.010  | 3.177            | 0.011 | 0.009 | 0.010  |
|                 | 1B <sub>1</sub> | 2A <sub>1</sub> | 3.909            | 0.014 | 0.014 | -0.014 | 3.923            | 0.014 | 0.014 | -0.014 |
| Diazirine       | 1B <sub>2</sub> | 2A <sub>1</sub> | 0.537            | 0.080 | 0.080 | -0.080 | 0.505            | 0.087 | 0.074 | -0.084 |
|                 | 1A <sub>2</sub> | 1B <sub>2</sub> | 1.626            | 0.003 | 0.002 | -0.003 | 1.589            | 0.003 | 0.002 | -0.002 |
| Silylidene      | 1B <sub>1</sub> | 1A <sub>2</sub> | 1.768            | 0.281 | 0.283 | 0.282  | 1.756            | 0.285 | 0.287 | 0.288  |
| Water           |                 |                 |                  |       |       |        |                  |       |       |        |

Table S21: Excited State absorption data for QR-CC2/dAVQZ and QR-CC3/AVQZ calculations.

| molecule        | State1          | State2          | QR-CC2/dAVQZ     |       |       |        | QR-CC3/AVQZ      |       |       |        |
|-----------------|-----------------|-----------------|------------------|-------|-------|--------|------------------|-------|-------|--------|
|                 |                 |                 | $\Delta E_{m,n}$ | $f^l$ | $f^v$ | $f^m$  | $\Delta E_{m,n}$ | $f^l$ | $f^v$ | $f^m$  |
| Ammonia         | 1A <sub>2</sub> | 1E              | 1.422            | 0.332 | 0.326 | 0.330  | 1.565            | 0.317 | 0.317 | 0.317  |
|                 | 1A <sub>2</sub> | 2A <sub>1</sub> | 1.795            | 0.305 | 0.300 | 0.303  | 2.495            | 0.335 | 0.249 | 0.289  |
|                 | 1E              | 2A <sub>2</sub> | 0.863            | 0.156 | 0.155 | 0.155  | 1.598            | 0.221 | 0.208 | 0.215  |
|                 | 2A <sub>1</sub> | 2A <sub>2</sub> | 0.490            | 0.222 | 0.265 | 0.243  | 0.668            | 0.054 | 0.725 | 0.198  |
| Carbon monoxide | 2 $\Sigma^+$    | 3 $\Sigma^+$    | 0.583            | 0.153 | 0.157 | 0.157  | 0.554            | 0.078 | 0.152 | 0.109  |
|                 | 2 $\Sigma^+$    | 2 $\Pi$         | 0.702            | 0.257 | 0.263 | 0.260  | 0.730            | 0.159 | 0.357 | 0.238  |
|                 | 2 $\Pi$         | 1 $\Pi$         | 2.952            | 0.011 | 0.009 | 0.010  | 3.162            | 0.012 | 0.012 | 0.012  |
|                 | 1B <sub>1</sub> | 2A <sub>1</sub> | 3.586            | 0.014 | 0.014 | -0.014 | 3.945            | 0.014 | 0.015 | -0.014 |
| Diazirine       | 1B <sub>2</sub> | 2A <sub>1</sub> | 0.477            | 0.100 | 0.105 | -0.103 | 0.569            | 0.075 | 0.060 | -0.067 |
|                 | 1A <sub>2</sub> | 1B <sub>2</sub> | 1.484            | 0.003 | 0.000 | -0.002 | 1.627            | 0.003 | 0.002 | -0.003 |
| Silylidene      | 1B <sub>1</sub> | 1A <sub>2</sub> | 1.646            | 0.311 | 0.302 | 0.307  | 1.774            | 0.284 | 0.281 | 0.283  |

Table S22: Excited State absorption data for QR-CCSD/AVQZ and QR-CC2/AVQZ calculations.

| molecule        | State1          | State2          | QR-CCSD/AVQZ     |       |       |        | QR-CC2/AVQZ      |       |       |        |
|-----------------|-----------------|-----------------|------------------|-------|-------|--------|------------------|-------|-------|--------|
|                 |                 |                 | $\Delta E_{m,n}$ | $f^l$ | $f^v$ | $f^m$  | $\Delta E_{m,n}$ | $f^l$ | $f^v$ | $f^m$  |
| Ammonia         | 1A <sub>2</sub> | 1E              | 1.541            | 0.319 | 0.320 | 0.321  | 1.452            | 0.330 | 0.322 | 0.327  |
|                 | 1A <sub>2</sub> | 2A <sub>1</sub> | 2.480            | 0.338 | 0.243 | 0.287  | 2.389            | 0.353 | 0.236 | 0.289  |
|                 | 1E              | 2A <sub>2</sub> | 1.599            | 0.224 | 0.207 | 0.215  | 1.576            | 0.239 | 0.201 | 0.220  |
|                 | 2A <sub>1</sub> | 2A <sub>2</sub> | 0.659            | 0.052 | 0.736 | 0.195  | 0.640            | 0.040 | 0.828 | 0.181  |
| Carbon monoxide | 2 $\Sigma^+$    | 3 $\Sigma^+$    | 0.543            | 0.083 | 0.153 | 0.114  | 0.529            | 0.078 | 0.160 | 0.114  |
|                 | 2 $\Sigma^+$    | 2 $\Pi$         | 0.725            | 0.160 | 0.367 | 0.244  | 0.702            | 0.157 | 0.361 | 0.238  |
|                 | 2 $\Pi$         | 1 $\Pi$         | 3.342            | 0.013 | 0.011 | 0.012  | 3.152            | 0.014 | 0.011 | 0.012  |
|                 | 1B <sub>1</sub> | 2A <sub>1</sub> | 3.961            | 0.014 | 0.015 | -0.015 | 3.637            | 0.015 | 0.014 | -0.014 |
| Diazirine       | 1B <sub>2</sub> | 2A <sub>1</sub> | 0.539            | 0.080 | 0.052 | -0.069 | 0.519            | 0.091 | 0.073 | -0.082 |
|                 | 1A <sub>2</sub> | 1B <sub>2</sub> | 1.590            | 0.003 | 0.002 | -0.002 | 1.485            | 0.003 | 0.000 | -0.002 |
| Silylidene      | 1B <sub>1</sub> | 1A <sub>2</sub> | 1.762            | 0.289 | 0.285 | 0.289  | 1.655            | 0.314 | 0.301 | 0.308  |



Table S23: Excited State absorption data for QR-CC3/tAVTZ and QR-CCSD/tAVTZ calculations.

| molecule        | State1          | State2          | QR-CC3/tAVTZ     |       |       |        | QR-CCSD/tAVTZ    |       |       |        |
|-----------------|-----------------|-----------------|------------------|-------|-------|--------|------------------|-------|-------|--------|
|                 |                 |                 | $\Delta E_{m,n}$ | $f^l$ | $f^v$ | $f^m$  | $\Delta E_{m,n}$ | $f^l$ | $f^v$ | $f^m$  |
| Ammonia         | 1A <sub>2</sub> | 1E              | 1.545            | 0.320 | 0.321 | 0.320  | 1.519            | 0.323 | 0.324 | 0.325  |
|                 | 1A <sub>2</sub> | 2A <sub>1</sub> | 1.987            | 0.292 | 0.294 | 0.293  | 1.960            | 0.294 | 0.290 | 0.292  |
|                 | 1E              | 2A <sub>2</sub> | 1.000            | 0.119 | 0.120 | 0.120  | 0.986            | 0.121 | 0.120 | 0.120  |
| Carbon monoxide | 2A <sub>1</sub> | 2A <sub>2</sub> | 0.557            | 0.313 | 0.314 | 0.314  | 0.545            | 0.313 | 0.313 | 0.313  |
|                 | 2 $\Sigma^+$    | 3 $\Sigma^+$    | 0.607            | 0.146 | 0.147 | 0.147  | 0.604            | 0.146 | 0.145 | 0.147  |
|                 | 2 $\Sigma^+$    | 2 $\Pi$         | 0.736            | 0.258 | 0.260 | 0.259  | 0.738            | 0.256 | 0.259 | 0.259  |
|                 | 2 $\Pi$         | 1 $\Pi$         | 2.931            | 0.010 | 0.009 | 0.009  | 3.116            | 0.010 | 0.008 | 0.010  |
| Diazirine       | 1B <sub>1</sub> | 2A <sub>1</sub> | 3.860            | 0.014 | 0.015 | -0.014 | 3.863            | 0.014 | 0.015 | -0.014 |
|                 | 1B <sub>2</sub> | 2A <sub>1</sub> | 0.530            | 0.084 | 0.084 | -0.084 | 0.503            | 0.090 | 0.078 | -0.088 |
| Silylidene      | 1A <sub>2</sub> | 1B <sub>2</sub> | 1.624            | 0.003 | 0.002 | -0.003 | 1.589            | 0.003 | 0.002 | -0.002 |
| Water           | 1B <sub>1</sub> | 1A <sub>2</sub> | 1.768            | 0.283 | 0.283 | 0.283  | 1.756            | 0.287 | 0.288 | 0.289  |

Table S24: Excited State absorption data for QR-CC2/tAVTZ and QR-CC3/tAVDZ calculations.

| molecule        | State1          | State2          | QR-CC2/tAVTZ     |       |       |        | QR-CC3/tAVDZ     |       |       |        |
|-----------------|-----------------|-----------------|------------------|-------|-------|--------|------------------|-------|-------|--------|
|                 |                 |                 | $\Delta E_{m,n}$ | $f^l$ | $f^v$ | $f^m$  | $\Delta E_{m,n}$ | $f^l$ | $f^v$ | $f^m$  |
| Ammonia         | 1A <sub>2</sub> | 1E              | 1.417            | 0.333 | 0.326 | 0.330  | 1.536            | 0.323 | 0.323 | 0.323  |
|                 | 1A <sub>2</sub> | 2A <sub>1</sub> | 1.781            | 0.302 | 0.297 | 0.300  | 1.971            | 0.295 | 0.295 | 0.295  |
|                 | 1E              | 2A <sub>2</sub> | 0.857            | 0.142 | 0.138 | 0.140  | 0.988            | 0.126 | 0.127 | 0.126  |
|                 | 2A <sub>1</sub> | 2A <sub>2</sub> | 0.493            | 0.278 | 0.275 | 0.276  | 0.554            | 0.305 | 0.303 | 0.304  |
| Carbon monoxide | 2 $\Sigma^+$    | 3 $\Sigma^+$    | 0.579            | 0.154 | 0.158 | 0.158  | 0.597            | 0.147 | 0.149 | 0.148  |
|                 | 2 $\Sigma^+$    | 2 $\Pi$         | 0.701            | 0.261 | 0.261 | 0.262  | 0.737            | 0.262 | 0.264 | 0.263  |
|                 | 2 $\Pi$         | 1 $\Pi$         | 2.880            | 0.011 | 0.008 | 0.009  | 2.708            | 0.010 | 0.008 | 0.009  |
|                 | 1B <sub>1</sub> | 2A <sub>1</sub> | 3.517            | 0.014 | 0.014 | -0.014 | 3.684            | 0.014 | 0.015 | -0.015 |
| Diazirine       | 1B <sub>2</sub> | 2A <sub>1</sub> | 0.478            | 0.103 | 0.108 | -0.106 | 0.511            | 0.094 | 0.095 | -0.094 |
|                 | 1A <sub>2</sub> | 1B <sub>2</sub> | 1.485            | 0.003 | 0.000 | -0.002 | 1.624            | 0.003 | 0.002 | -0.003 |
| Silylidene      | 1B <sub>1</sub> | 1A <sub>2</sub> | 1.641            | 0.312 | 0.302 | 0.308  | 1.765            | 0.288 | 0.285 | 0.287  |

Table S25: Excited State absorption data for QR-CCSD/tAVDZ and QR-CC2/tAVDZ calculations.

| molecule        | State1          | State2          | QR-CCSD/tAVDZ    |       |       |        | QR-CC2/tAVDZ     |       |       |        |
|-----------------|-----------------|-----------------|------------------|-------|-------|--------|------------------|-------|-------|--------|
|                 |                 |                 | $\Delta E_{m,n}$ | $f^l$ | $f^v$ | $f^m$  | $\Delta E_{m,n}$ | $f^l$ | $f^v$ | $f^m$  |
| Ammonia         | 1A <sub>2</sub> | 1E              | 1.508            | 0.326 | 0.326 | 0.327  | 1.399            | 0.335 | 0.327 | 0.332  |
|                 | 1A <sub>2</sub> | 2A <sub>1</sub> | 1.940            | 0.297 | 0.292 | 0.295  | 1.758            | 0.305 | 0.298 | 0.302  |
|                 | 1E              | 2A <sub>2</sub> | 0.973            | 0.127 | 0.127 | 0.127  | 0.848            | 0.147 | 0.143 | 0.145  |
|                 | 2A <sub>1</sub> | 2A <sub>2</sub> | 0.542            | 0.305 | 0.303 | 0.304  | 0.489            | 0.272 | 0.266 | 0.269  |
| Carbon monoxide | 2 $\Sigma^+$    | 3 $\Sigma^+$    | 0.593            | 0.147 | 0.148 | 0.149  | 0.567            | 0.156 | 0.161 | 0.161  |
|                 | 2 $\Sigma^+$    | 2 $\Pi$         | 0.736            | 0.259 | 0.262 | 0.262  | 0.696            | 0.264 | 0.265 | 0.265  |
|                 | 2 $\Pi$         | 1 $\Pi$         | 2.870            | 0.010 | 0.008 | 0.009  | 2.654            | 0.011 | 0.008 | 0.009  |
|                 | 1B <sub>1</sub> | 2A <sub>1</sub> | 3.649            | 0.015 | 0.016 | -0.015 | 3.305            | 0.015 | 0.015 | -0.015 |
| Diazirine       | 1B <sub>2</sub> | 2A <sub>1</sub> | 0.494            | 0.098 | 0.088 | -0.097 | 0.480            | 0.112 | 0.118 | -0.115 |
|                 | 1A <sub>2</sub> | 1B <sub>2</sub> | 1.589            | 0.003 | 0.002 | -0.002 | 1.485            | 0.003 | 0.000 | -0.002 |
| Silylidene      | 1B <sub>1</sub> | 1A <sub>2</sub> | 1.750            | 0.294 | 0.291 | 0.294  | 1.626            | 0.316 | 0.303 | 0.310  |
| Water           |                 |                 |                  |       |       |        |                  |       |       |        |

### S3.3 Full testing set, QR-CC3, QR-CCSD, QR-CC2, with AVDZ, dAVDZ, AVTZ, and dAVTZ basis sets

Table S26: Excited State absorption data for QR-CC3/AVDZ and QR-CCSD/AVDZ calculations.  $\Delta E_{m,n}$ [eV] and oscillator strengths in length, velocity, and mixed gauges,  $f^l$ ,  $f^v$ , and  $f^m$ , respectively.

| Molecule        | State1           | State2           | QR-CC3/AVDZ      |       |       |        | QR-CCSD/AVDZ     |       |       |        |
|-----------------|------------------|------------------|------------------|-------|-------|--------|------------------|-------|-------|--------|
|                 |                  |                  | $\Delta E_{m,n}$ | $f^l$ | $f^v$ | $f^m$  | $\Delta E_{m,n}$ | $f^l$ | $f^v$ | $f^m$  |
| Acetone         | 1B <sub>2</sub>  | 2A <sub>1</sub>  | 1.082            | 0.262 | 0.259 | -0.261 | 1.065            | 0.272 | 0.252 | -0.270 |
|                 | 1B <sub>2</sub>  | 2B <sub>2</sub>  | 1.254            | 0.276 | 0.213 | 0.243  | 1.199            | 0.285 | 0.202 | 0.252  |
|                 | 1B <sub>2</sub>  | 2A <sub>2</sub>  | 1.064            | 0.336 | 0.358 | 0.347  | 1.030            | 0.343 | 0.330 | 0.355  |
| Acrolein        | 1A''             | 2A''             | 2.987            | 0.038 | 0.041 | 0.040  | 3.294            | 0.053 | 0.041 | 0.051  |
| Ammonia         | 1A <sub>2</sub>  | 1E               | 1.596            | 0.315 | 0.312 | 0.313  | 1.569            | 0.317 | 0.317 | 0.318  |
|                 | 1A <sub>2</sub>  | 2A <sub>1</sub>  | 3.199            | 0.315 | 0.144 | 0.213  | 3.194            | 0.317 | 0.139 | 0.211  |
|                 | 1E               | 2A <sub>2</sub>  | 2.336            | 0.255 | 0.204 | 0.228  | 2.352            | 0.257 | 0.201 | 0.227  |
| Benzene         | 2A <sub>1</sub>  | 2A <sub>2</sub>  | 0.733            | 0.002 | 1.251 | 0.048  | 0.727            | 0.001 | 1.272 | 0.042  |
|                 | 1E <sub>1g</sub> | 1A <sub>2u</sub> | 0.564            | 0.130 | 0.123 | -0.126 | 0.544            | 0.131 | 0.090 | -0.120 |
|                 | 1E <sub>1g</sub> | 1E <sub>2u</sub> | 0.631            | 0.135 | 0.130 | 0.132  | 0.623            | 0.139 | 0.128 | 0.146  |
| Butadiene       | 1B <sub>g</sub>  | 1A <sub>u</sub>  | 0.317            | 0.111 | 0.105 | -0.108 | 0.317            | 0.116 | 0.050 | -0.115 |
|                 | 1B <sub>g</sub>  | 2A <sub>u</sub>  | 0.474            | 0.151 | 0.167 | -0.159 | 0.478            | 0.154 | 0.162 | -0.164 |
|                 | 1A <sub>u</sub>  | 2B <sub>g</sub>  | 0.938            | 0.062 | 0.075 | 0.068  | 0.933            | 0.062 | 0.076 | 0.069  |
| Carbon monoxide | 2A <sub>u</sub>  | 2B <sub>g</sub>  | 0.780            | 0.327 | 0.289 | 0.308  | 0.773            | 0.333 | 0.290 | 0.316  |
|                 | 2Σ <sup>+</sup>  | 3Σ <sup>+</sup>  | 0.565            | 0.030 | 0.154 | 0.068  | 0.539            | 0.035 | 0.161 | 0.075  |
|                 | 2Σ <sup>+</sup>  | 2Π               | 0.820            | 0.133 | 0.270 | 0.190  | 0.802            | 0.134 | 0.291 | 0.199  |
| Cyclopentadiene | 2Π               | 1Π               | 3.165            | 0.015 | 0.015 | 0.015  | 3.302            | 0.015 | 0.012 | 0.014  |
|                 | 2Σ <sup>+</sup>  | 1Π               | 2.345            | 0.026 | 0.015 | -0.020 | 2.500            | 0.026 | 0.015 | -0.019 |
|                 | 3Σ <sup>+</sup>  | 1Π               | 2.910            | 0.023 | 0.023 | -0.023 | 3.040            | 0.020 | 0.022 | -0.021 |
|                 | 1B <sub>2</sub>  | 2A <sub>1</sub>  | 1.007            | 0.023 | 0.030 | -0.026 | 1.241            | 0.045 | 0.006 | -0.063 |
|                 | 1A <sub>2</sub>  | 1B <sub>1</sub>  | 0.637            | 0.224 | 0.227 | -0.225 | 0.621            | 0.227 | 0.218 | -0.231 |
|                 | 1A <sub>2</sub>  | 2B <sub>2</sub>  | 0.845            | 0.248 | 0.200 | -0.223 | 0.839            | 0.251 | 0.181 | -0.224 |

| Molecule              | State1           | State2           | QR-CC3/AVDZ      |       |       |        | QR-CCSD/AVDZ     |       |        |        |
|-----------------------|------------------|------------------|------------------|-------|-------|--------|------------------|-------|--------|--------|
|                       |                  |                  | $\Delta E_{m,n}$ | $f^l$ | $f^v$ | $f^m$  | $\Delta E_{m,n}$ | $f^l$ | $f^v$  | $f^m$  |
| Cyclopropene          | 1A <sub>2</sub>  | 2A <sub>2</sub>  | 0.685            | 0.244 | 0.227 | 0.236  | 0.678            | 0.253 | 0.205  | 0.248  |
|                       | 2B <sub>1</sub>  | 3B <sub>1</sub>  | 0.397            | 0.097 | 0.078 | 0.087  | 0.403            | 0.099 | 0.066  | 0.090  |
|                       | 1B <sub>1</sub>  | 2A <sub>1</sub>  | 3.808            | 0.015 | 0.014 | -0.015 | 3.779            | 0.015 | 0.014  | -0.015 |
|                       | 1B <sub>2</sub>  | 2A <sub>1</sub>  | 0.611            | 0.077 | 0.039 | -0.055 | 0.596            | 0.080 | 0.031  | -0.055 |
| Diazomethane          | 1A <sub>2</sub>  | 1B <sub>1</sub>  | 2.221            | 0.013 | 0.013 | -0.013 | 2.197            | 0.013 | 0.012  | -0.013 |
|                       | 1B <sub>2</sub>  | 2A <sub>1</sub>  | 1.030            | 0.300 | 0.276 | -0.288 | 1.009            | 0.304 | 0.268  | -0.289 |
| Formaldehyde          | 1B <sub>2</sub>  | 2A <sub>2</sub>  | 1.604            | 0.287 | 0.181 | 0.228  | 1.571            | 0.294 | 0.184  | 0.235  |
|                       | 1A <sub>2</sub>  | 1B <sub>2</sub>  | 3.048            | 0.021 | 0.018 | -0.020 | 3.023            | 0.021 | 0.016  | -0.019 |
|                       | 2B <sub>2</sub>  | 2A <sub>2</sub>  | 0.638            | 0.008 | 0.013 | 0.011  | 0.621            | 0.007 | 0.010  | 0.008  |
|                       | 1A <sub>2</sub>  | 2A <sub>2</sub>  | 4.651            | 0.020 | 0.019 | 0.019  | 4.594            | 0.021 | 0.019  | 0.020  |
| Furane                | 1A <sub>2</sub>  | 2B <sub>2</sub>  | 1.393            | 0.272 | 0.087 | -0.153 | 1.403            | 0.272 | 0.076  | -0.151 |
|                       | 1A <sub>2</sub>  | 1B <sub>1</sub>  | 0.555            | 0.220 | 0.189 | -0.204 | 0.541            | 0.218 | 0.173  | -0.205 |
| Glyoxal               | 1A <sub>2</sub>  | 2A <sub>2</sub>  | 0.733            | 0.252 | 0.246 | 0.249  | 0.731            | 0.256 | 0.232  | 0.256  |
|                       | 1A <sub>u</sub>  | 1B <sub>g</sub>  | 1.400            | 0.021 | 0.020 | 0.021  | 1.411            | 0.019 | -0.016 | 0.022  |
|                       | 1A <sub>u</sub>  | 2B <sub>g</sub>  | 3.689            | 0.116 | 0.117 | 0.117  | 4.058            | 0.159 | 0.144  | 0.160  |
|                       | 1B <sub>1</sub>  | 2A <sub>2</sub>  | 1.217            | 0.338 | 0.317 | 0.327  | 1.210            | 0.341 | 0.316  | 0.332  |
| Ketene                | 1B <sub>1</sub>  | 2A <sub>1</sub>  | 1.410            | 0.124 | 0.064 | -0.089 | 1.397            | 0.128 | 0.070  | -0.095 |
|                       | 1B <sub>1</sub>  | 1A <sub>2</sub>  | 0.523            | 0.180 | 0.163 | 0.171  | 0.527            | 0.189 | 0.143  | 0.184  |
| Methylenecyclopropene | 1B <sub>2</sub>  | 1A <sub>2</sub>  | 1.555            | 0.024 | 0.026 | 0.025  | 1.342            | 0.024 | 0.027  | 0.025  |
|                       | 2A <sub>g</sub>  | 2B <sub>1u</sub> | 0.837            | 0.183 | 0.185 | 0.184  | 0.807            | 0.172 | 0.176  | 0.174  |
| Pyrazine              | 2A <sub>g</sub>  | 2B <sub>2u</sub> | 0.598            | 0.248 | 0.207 | 0.227  | 0.608            | 0.261 | 0.127  | 0.242  |
|                       | 1B <sub>1u</sub> | 1B <sub>3g</sub> | 0.981            | 0.007 | 0.006 | 0.006  | 0.988            | 0.013 | 0.010  | 0.012  |
|                       | 2B <sub>2u</sub> | 1B <sub>3g</sub> | 0.767            | 0.178 | 0.182 | 0.180  | 0.735            | 0.173 | 0.177  | 0.175  |
|                       | 1A <sub>2</sub>  | 2B <sub>1</sub>  | 2.018            | 0.013 | 0.010 | -0.011 | 2.037            | 0.013 | -0.020 | -0.012 |
| Pyrrole               | 1A <sub>2</sub>  | 1B <sub>1</sub>  | 0.739            | 0.049 | 0.049 | -0.049 | 0.689            | 0.050 | 0.059  | -0.055 |
|                       | 1A <sub>2</sub>  | 2A <sub>2</sub>  | 0.792            | 0.163 | 0.157 | 0.160  | 0.766            | 0.175 | 0.149  | 0.175  |

| Molecule   | State1           | State2           | QR-CC3/AVDZ      |       |       |        | QR-CCSD/AVDZ     |       |        |        |
|------------|------------------|------------------|------------------|-------|-------|--------|------------------|-------|--------|--------|
|            |                  |                  | $\Delta E_{m,n}$ | $f^l$ | $f^v$ | $f^m$  | $\Delta E_{m,n}$ | $f^l$ | $f^v$  | $f^m$  |
| Silylidene | 1A <sub>2</sub>  | 1B <sub>2</sub>  | 1.622            | 0.003 | 0.003 | -0.003 | 1.587            | 0.003 | 0.003  | -0.003 |
| Tetrazine  | 1B <sub>3u</sub> | 1B <sub>1g</sub> | 2.478            | 0.064 | 0.070 | 0.067  | 2.653            | 0.077 | 0.005  | 0.087  |
|            | 1B <sub>3u</sub> | 1B <sub>2g</sub> | 3.045            | 0.016 | 0.013 | 0.015  | 3.230            | 0.026 | 0.013  | 0.030  |
| Thiophene  | 1A <sub>2</sub>  | 1B <sub>1</sub>  | 0.119            | 0.017 | 0.008 | -0.012 | 0.182            | 0.034 | -0.029 | -0.028 |
| Water      | 1B <sub>1</sub>  | 1A <sub>2</sub>  | 1.782            | 0.293 | 0.285 | 0.289  | 1.766            | 0.298 | 0.292  | 0.296  |

Table S27: Excited State absorption data for QR-CC2/AVDZ and QR-CC3/dAVDZ calculations.  $\Delta E_{m,n}[\text{eV}]$  and oscillator strengths in length, velocity, and mixed gauges,  $f^l$ ,  $f^v$ , and  $f^m$ , respectively.

| Molecule        | State1           | State2           | QR-CC2/AVDZ      |       |       | QR-CC3/dAVDZ |                  |       |       |        |
|-----------------|------------------|------------------|------------------|-------|-------|--------------|------------------|-------|-------|--------|
|                 |                  |                  | $\Delta E_{m,n}$ | $f^l$ | $f^v$ | $f^m$        | $\Delta E_{m,n}$ | $f^l$ | $f^v$ | $f^m$  |
| Acetone         | 1B <sub>2</sub>  | 2A <sub>1</sub>  | 1.007            | 0.284 | 0.277 | -0.286       | 1.025            | 0.260 | 0.263 | -0.261 |
|                 | 1B <sub>2</sub>  | 2B <sub>2</sub>  | 1.213            | 0.290 | 0.214 | 0.252        | 1.024            | 0.270 | 0.269 | 0.269  |
|                 | 1B <sub>2</sub>  | 2A <sub>2</sub>  | 0.979            | 0.349 | 0.358 | 0.358        | 0.954            | 0.363 | 0.361 | 0.362  |
| Acrolein        | 1A''             | 2A''             | 2.781            | 0.081 | 0.079 | 0.083        | 2.970            | 0.036 | 0.038 | 0.037  |
| Ammonia         | 1A <sub>2</sub>  | 1E               | 1.484            | 0.326 | 0.318 | 0.323        | 1.537            | 0.323 | 0.323 | 0.323  |
|                 | 1A <sub>2</sub>  | 2A <sub>1</sub>  | 3.151            | 0.322 | 0.122 | 0.199        | 1.979            | 0.298 | 0.298 | 0.298  |
|                 | 1E               | 2A <sub>2</sub>  | 2.415            | 0.259 | 0.182 | 0.217        | 0.994            | 0.150 | 0.155 | 0.153  |
| Benzene         | 2A <sub>1</sub>  | 2A <sub>2</sub>  | 0.747            | 0.000 | 1.335 | 0.010        | 0.552            | 0.231 | 0.270 | 0.250  |
|                 | 1E <sub>1g</sub> | 1A <sub>2u</sub> | 0.533            | 0.137 | 0.128 | -0.139       | 0.545            | 0.133 | 0.133 | -0.133 |
|                 | 1E <sub>1g</sub> | 1E <sub>2u</sub> | 0.597            | 0.142 | 0.124 | 0.140        | 0.606            | 0.138 | 0.138 | 0.138  |
| Butadiene       | 1B <sub>g</sub>  | 1A <sub>u</sub>  | 0.319            | 0.122 | 0.099 | -0.124       | 0.319            | 0.125 | 0.129 | -0.127 |
|                 | 1B <sub>g</sub>  | 2A <sub>u</sub>  | 0.450            | 0.164 | 0.171 | -0.179       | 0.471            | 0.168 | 0.171 | -0.169 |
|                 | 1A <sub>u</sub>  | 2B <sub>g</sub>  | 0.901            | 0.065 | 0.082 | 0.074        | 0.814            | 0.060 | 0.061 | 0.060  |
| Carbon monoxide | 2A <sub>u</sub>  | 2B <sub>g</sub>  | 0.770            | 0.358 | 0.310 | 0.339        | 0.661            | 0.375 | 0.378 | 0.376  |
|                 | 2Σ <sup>+</sup>  | 3Σ <sup>+</sup>  | 0.539            | 0.029 | 0.164 | 0.071        | 0.602            | 0.147 | 0.151 | 0.149  |
|                 | 2Σ <sup>+</sup>  | 2Π               | 0.789            | 0.131 | 0.271 | 0.189        | 0.740            | 0.263 | 0.260 | 0.261  |
|                 | 2Π               | 1Π               | 3.154            | 0.017 | 0.014 | 0.015        | 2.710            | 0.011 | 0.007 | 0.009  |
|                 | 2Σ <sup>+</sup>  | 1Π               | 2.365            | 0.021 | 0.007 | -0.012       | 1.970            | 0.027 | 0.026 | -0.027 |
|                 | 3Σ <sup>+</sup>  | 1Π               | 2.904            | 0.022 | 0.021 | -0.022       | 2.571            | 0.011 | 0.010 | -0.011 |
| Cyclopentadiene | 1B <sub>2</sub>  | 2A <sub>1</sub>  | 1.343            | 0.065 | 0.069 | -0.080       | 1.005            | 0.023 | 0.030 | -0.026 |
|                 | 1A <sub>2</sub>  | 1B <sub>1</sub>  | 0.600            | 0.237 | 0.234 | -0.244       | 0.610            | 0.236 | 0.236 | -0.236 |
|                 | 1A <sub>2</sub>  | 2B <sub>2</sub>  | 0.826            | 0.255 | 0.207 | -0.231       | 0.683            | 0.284 | 0.283 | -0.283 |



| Molecule              | State1           | State2           | QR-CC2/AVDZ      |       |        |        | QR-CC3/dAVDZ     |       |       |        |
|-----------------------|------------------|------------------|------------------|-------|--------|--------|------------------|-------|-------|--------|
|                       |                  |                  | $\Delta E_{m,n}$ | $f^l$ | $f^v$  | $f^m$  | $\Delta E_{m,n}$ | $f^l$ | $f^v$ | $f^m$  |
| Cyclopropene          | 1A <sub>2</sub>  | 2A <sub>2</sub>  | 0.654            | 0.258 | 0.234  | 0.256  | 0.648            | 0.254 | 0.253 | 0.253  |
|                       | 2B <sub>1</sub>  | 3B <sub>1</sub>  | 0.354            | 0.013 | 0.013  | 0.013  | 0.377            | 0.104 | 0.104 | 0.104  |
|                       | 1B <sub>1</sub>  | 2A <sub>1</sub>  | 3.469            | 0.016 | 0.014  | -0.015 | 3.684            | 0.014 | 0.015 | -0.015 |
|                       | 1B <sub>2</sub>  | 2A <sub>1</sub>  | 0.605            | 0.090 | 0.045  | -0.064 | 0.512            | 0.094 | 0.094 | -0.094 |
| Diazomethane          | 1A <sub>2</sub>  | 1B <sub>1</sub>  | 1.970            | 0.014 | 0.012  | -0.013 | 2.186            | 0.013 | 0.013 | -0.013 |
|                       | 1B <sub>2</sub>  | 2A <sub>1</sub>  | 0.987            | 0.308 | 0.286  | -0.298 | 0.962            | 0.297 | 0.298 | -0.297 |
| Formaldehyde          | 1B <sub>2</sub>  | 2A <sub>2</sub>  | 1.665            | 0.302 | 0.184  | 0.236  | 1.198            | 0.281 | 0.279 | 0.280  |
|                       | 1A <sub>2</sub>  | 1B <sub>2</sub>  | 2.304            | 0.022 | 0.022  | -0.022 | 3.041            | 0.019 | 0.020 | -0.019 |
|                       | 2B <sub>2</sub>  | 2A <sub>2</sub>  | 0.585            | 0.012 | 0.017  | 0.015  | 0.373            | 0.010 | 0.011 | 0.011  |
|                       | 1A <sub>2</sub>  | 2A <sub>2</sub>  | 3.969            | 0.024 | 0.020  | 0.022  | 4.239            | 0.015 | 0.014 | 0.014  |
| Furane                | 1A <sub>2</sub>  | 2B <sub>2</sub>  | 1.461            | 0.280 | 0.077  | -0.148 | 0.843            | 0.253 | 0.251 | -0.252 |
|                       | 1A <sub>2</sub>  | 1B <sub>1</sub>  | 0.528            | 0.230 | 0.187  | -0.218 | 0.541            | 0.221 | 0.221 | -0.221 |
|                       | 1A <sub>2</sub>  | 2A <sub>2</sub>  | 0.705            | 0.260 | 0.255  | 0.263  | 0.686            | 0.269 | 0.268 | 0.268  |
|                       | 1A <sub>u</sub>  | 1B <sub>g</sub>  | 1.533            | 0.035 | -0.008 | 0.038  | 1.399            | 0.020 | 0.020 | 0.021  |
| Glyoxal               | 1A <sub>u</sub>  | 2B <sub>g</sub>  | 3.588            | 0.181 | 0.185  | 0.188  | 3.661            | 0.112 | 0.112 | 0.112  |
|                       | 1B <sub>1</sub>  | 2A <sub>2</sub>  | 1.153            | 0.348 | 0.321  | 0.336  | 1.144            | 0.338 | 0.337 | 0.337  |
| Ketene                | 1B <sub>1</sub>  | 2A <sub>1</sub>  | 1.481            | 0.174 | 0.098  | -0.131 | 1.154            | 0.203 | 0.195 | -0.199 |
|                       | 1B <sub>1</sub>  | 1A <sub>2</sub>  | 0.504            | 0.192 | 0.181  | 0.189  | 0.506            | 0.191 | 0.192 | 0.192  |
| Methylenecyclopropene | 1B <sub>2</sub>  | 1A <sub>2</sub>  | 1.217            | 0.023 | 0.029  | 0.026  | 1.499            | 0.024 | 0.025 | 0.025  |
|                       | 2A <sub>g</sub>  | 2B <sub>1u</sub> | 0.944            | 0.067 | 0.069  | 0.069  | 0.781            | 0.205 | 0.205 | 0.205  |
| Pyrazine              | 2A <sub>g</sub>  | 2B <sub>2u</sub> | 0.535            | 0.270 | 0.185  | 0.250  | 0.590            | 0.243 | 0.244 | 0.243  |
|                       | 1B <sub>1u</sub> | 1B <sub>3g</sub> | 0.509            | 0.193 | 0.126  | 0.169  | 0.887            | 0.009 | 0.009 | 0.009  |
|                       | 2B <sub>2u</sub> | 1B <sub>3g</sub> | 0.758            | 0.206 | 0.211  | 0.212  | 0.718            | 0.203 | 0.203 | 0.203  |
|                       | 1A <sub>2</sub>  | 2B <sub>1</sub>  | 2.098            | 0.019 | 0.016  | -0.020 | 2.018            | 0.013 | 0.009 | -0.011 |
| Pyrrole               | 1A <sub>2</sub>  | 1B <sub>1</sub>  | 0.678            | 0.026 | 0.022  | -0.025 | 0.728            | 0.086 | 0.085 | -0.086 |
|                       | 1A <sub>2</sub>  | 2A <sub>2</sub>  | 0.756            | 0.177 | 0.168  | 0.177  | 0.744            | 0.171 | 0.170 | 0.171  |

| Molecule   | State1           | State2           | QR-CC2/AVDZ      |       |        | QR-CC3/dAVDZ     |       |       |
|------------|------------------|------------------|------------------|-------|--------|------------------|-------|-------|
|            |                  |                  | $\Delta E_{m,n}$ | $f^l$ | $f^v$  | $\Delta E_{m,n}$ | $f^l$ | $f^v$ |
| Silylidene | 1A <sub>2</sub>  | 1B <sub>2</sub>  | 1.478            | 0.003 | 0.001  | -0.003           | 0.003 | 0.003 |
|            | 1B <sub>3u</sub> | 1B <sub>1g</sub> | 2.674            | 0.104 | 0.087  | 0.117            | 0.064 | 0.069 |
|            | 1B <sub>3u</sub> | 1B <sub>2g</sub> | 3.302            | 0.035 | 0.028  | 0.037            | 0.017 | 0.015 |
| Thiophene  | 1A <sub>2</sub>  | 1B <sub>1</sub>  | 0.189            | 0.043 | -0.000 | -0.040           | 0.023 | 0.022 |
|            | 1B <sub>1</sub>  | 1A <sub>2</sub>  | 1.654            | 0.318 | 0.307  | 0.313            | 0.288 | 0.285 |
| Water      |                  |                  |                  |       |        |                  |       | 0.287 |

Table S28: Excited State absorption data for QR-CCSD/dAVDZ and QR-CC2/dAVDZ calculations.  $\Delta E_{m,n}$ [eV] and oscillator strengths in length, velocity, and mixed gauges,  $f^l$ ,  $f^v$ , and  $f^m$ , respectively.

| Molecule        | State1           | State2           | QR-CCSD/dAVDZ    |       |       |        | QR-CC2/dAVDZ     |       |       |        |
|-----------------|------------------|------------------|------------------|-------|-------|--------|------------------|-------|-------|--------|
|                 |                  |                  | $\Delta E_{m,n}$ | $f^l$ | $f^v$ | $f^m$  | $\Delta E_{m,n}$ | $f^l$ | $f^v$ | $f^m$  |
| Acetone         | 1B <sub>2</sub>  | 2A <sub>1</sub>  | 1.003            | 0.269 | 0.256 | -0.269 | 0.915            | 0.283 | 0.276 | -0.284 |
|                 | 1B <sub>2</sub>  | 2B <sub>2</sub>  | 0.977            | 0.277 | 0.258 | 0.278  | 0.919            | 0.290 | 0.282 | 0.289  |
|                 | 1B <sub>2</sub>  | 2A <sub>2</sub>  | 0.901            | 0.371 | 0.331 | 0.369  | 0.841            | 0.378 | 0.358 | 0.372  |
| Acrolein        | 1A''             | 2A''             | 3.263            | 0.049 | 0.037 | 0.047  | 2.714            | 0.068 | 0.063 | 0.068  |
| Ammonia         | 1A <sub>2</sub>  | 1E               | 1.508            | 0.326 | 0.326 | 0.327  | 1.399            | 0.335 | 0.327 | 0.332  |
|                 | 1A <sub>2</sub>  | 2A <sub>1</sub>  | 1.948            | 0.300 | 0.294 | 0.297  | 1.772            | 0.311 | 0.303 | 0.307  |
|                 | 1E               | 2A <sub>2</sub>  | 0.980            | 0.152 | 0.156 | 0.154  | 0.856            | 0.168 | 0.169 | 0.169  |
| Benzene         | 2A <sub>1</sub>  | 2A <sub>2</sub>  | 0.540            | 0.228 | 0.270 | 0.248  | 0.483            | 0.193 | 0.271 | 0.229  |
|                 | 1E <sub>1g</sub> | 1A <sub>2u</sub> | 0.525            | 0.135 | 0.102 | -0.127 | 0.507            | 0.143 | 0.137 | -0.146 |
|                 | 1E <sub>1g</sub> | 1E <sub>2u</sub> | 0.596            | 0.142 | 0.139 | 0.151  | 0.564            | 0.147 | 0.132 | 0.145  |
|                 | 1B <sub>g</sub>  | 1A <sub>u</sub>  | 0.319            | 0.131 | 0.083 | -0.135 | 0.319            | 0.142 | 0.131 | -0.147 |
| Butadiene       | 1B <sub>g</sub>  | 2A <sub>u</sub>  | 0.474            | 0.172 | 0.166 | -0.175 | 0.444            | 0.188 | 0.174 | -0.191 |
|                 | 1A <sub>u</sub>  | 2B <sub>g</sub>  | 0.804            | 0.057 | 0.056 | 0.057  | 0.748            | 0.061 | 0.062 | 0.062  |
|                 | 2A <sub>u</sub>  | 2B <sub>g</sub>  | 0.649            | 0.387 | 0.387 | 0.390  | 0.623            | 0.415 | 0.415 | 0.419  |
|                 | 2Σ <sup>+</sup>  | 3Σ <sup>+</sup>  | 0.599            | 0.146 | 0.150 | 0.149  | 0.571            | 0.155 | 0.164 | 0.162  |
| Carbon monoxide | 2Σ <sup>+</sup>  | 2Π               | 0.740            | 0.260 | 0.257 | 0.260  | 0.699            | 0.264 | 0.262 | 0.264  |
|                 | 2Π               | 1Π               | 2.872            | 0.011 | 0.007 | 0.009  | 2.655            | 0.012 | 0.007 | 0.009  |
|                 | 2Σ <sup>+</sup>  | 1Π               | 2.132            | 0.026 | 0.024 | -0.025 | 1.956            | 0.023 | 0.016 | -0.019 |
|                 | 3Σ <sup>+</sup>  | 1Π               | 2.731            | 0.010 | 0.010 | -0.010 | 2.527            | 0.011 | 0.010 | -0.011 |
| Cyclopentadiene | 1B <sub>2</sub>  | 2A <sub>1</sub>  | 1.218            | 0.044 | 0.010 | -0.060 | 1.254            | 0.037 | 0.037 | -0.043 |
|                 | 1A <sub>2</sub>  | 1B <sub>1</sub>  | 0.593            | 0.241 | 0.227 | -0.242 | 0.566            | 0.255 | 0.242 | -0.256 |
|                 | 1A <sub>2</sub>  | 2B <sub>2</sub>  | 0.666            | 0.289 | 0.268 | -0.289 | 0.643            | 0.296 | 0.296 | -0.297 |

| Molecule              | State1           | State2           | QR-CCSD/dAVDZ    |       |        |        | QR-CC2/dAVDZ     |       |        |        |
|-----------------------|------------------|------------------|------------------|-------|--------|--------|------------------|-------|--------|--------|
|                       |                  |                  | $\Delta E_{m,n}$ | $f^l$ | $f^v$  | $f^m$  | $\Delta E_{m,n}$ | $f^l$ | $f^v$  | $f^m$  |
| Cyclopropene          | 1A <sub>2</sub>  | 2A <sub>2</sub>  | 0.638            | 0.263 | 0.234  | 0.265  | 0.605            | 0.273 | 0.261  | 0.275  |
|                       | 2B <sub>1</sub>  | 3B <sub>1</sub>  | 0.380            | 0.104 | 0.093  | 0.106  | 0.294            | 0.006 | 0.007  | 0.006  |
|                       | 1B <sub>1</sub>  | 2A <sub>1</sub>  | 3.649            | 0.015 | 0.015  | -0.015 | 3.305            | 0.015 | 0.015  | -0.015 |
|                       | 1B <sub>2</sub>  | 2A <sub>1</sub>  | 0.494            | 0.098 | 0.088  | -0.097 | 0.481            | 0.112 | 0.117  | -0.115 |
| Diazomethane          | 1A <sub>2</sub>  | 1B <sub>1</sub>  | 2.161            | 0.013 | 0.012  | -0.013 | 1.928            | 0.013 | 0.013  | -0.013 |
|                       | 1B <sub>2</sub>  | 2A <sub>1</sub>  | 0.935            | 0.300 | 0.294  | -0.301 | 0.912            | 0.301 | 0.303  | -0.303 |
| Formaldehyde          | 1B <sub>2</sub>  | 2A <sub>2</sub>  | 1.154            | 0.290 | 0.285  | 0.289  | 1.150            | 0.292 | 0.289  | 0.291  |
|                       | 1A <sub>2</sub>  | 1B <sub>2</sub>  | 3.014            | 0.019 | 0.018  | -0.019 | 2.291            | 0.020 | 0.025  | -0.022 |
|                       | 2B <sub>2</sub>  | 2A <sub>2</sub>  | 0.347            | 0.008 | 0.008  | 0.009  | 0.276            | 0.013 | 0.016  | 0.014  |
|                       | 1A <sub>2</sub>  | 2A <sub>2</sub>  | 4.168            | 0.015 | 0.014  | 0.014  | 3.441            | 0.016 | 0.013  | 0.015  |
| Furane                | 1A <sub>2</sub>  | 2B <sub>2</sub>  | 0.851            | 0.231 | 0.222  | -0.230 | 0.860            | 0.204 | 0.199  | -0.202 |
|                       | 1A <sub>2</sub>  | 1B <sub>1</sub>  | 0.526            | 0.222 | 0.207  | -0.223 | 0.510            | 0.237 | 0.222  | -0.238 |
| Glyoxal               | 1A <sub>2</sub>  | 2A <sub>2</sub>  | 0.684            | 0.274 | 0.256  | 0.276  | 0.650            | 0.282 | 0.276  | 0.284  |
|                       | 1A <sub>u</sub>  | 1B <sub>g</sub>  | 1.410            | 0.019 | -0.016 | 0.022  | 1.531            | 0.035 | -0.007 | 0.038  |
| Ketene                | 1A <sub>u</sub>  | 2B <sub>g</sub>  | 4.016            | 0.151 | 0.133  | 0.150  | 3.541            | 0.171 | 0.171  | 0.176  |
|                       | 1B <sub>1</sub>  | 2A <sub>2</sub>  | 1.138            | 0.341 | 0.335  | 0.342  | 1.072            | 0.346 | 0.342  | 0.346  |
| Methylenecyclopropene | 1B <sub>1</sub>  | 2A <sub>1</sub>  | 1.143            | 0.204 | 0.198  | -0.202 | 1.121            | 0.244 | 0.244  | -0.244 |
|                       | 1B <sub>1</sub>  | 1A <sub>2</sub>  | 0.506            | 0.201 | 0.174  | 0.204  | 0.482            | 0.209 | 0.208  | 0.211  |
| Pyrazine              | 1B <sub>2</sub>  | 1A <sub>2</sub>  | 1.282            | 0.025 | 0.025  | 0.025  | 1.148            | 0.025 | 0.025  | 0.025  |
|                       | 2A <sub>g</sub>  | 2B <sub>1u</sub> | 0.749            | 0.196 | 0.195  | 0.196  | 0.974            | 0.024 | 0.023  | 0.024  |
|                       | 2A <sub>g</sub>  | 2B <sub>2u</sub> | 0.597            | 0.255 | 0.180  | 0.258  | 0.518            | 0.269 | 0.237  | 0.272  |
|                       | 1B <sub>1u</sub> | 1B <sub>3g</sub> | 0.885            | 0.017 | 0.016  | 0.017  | 0.478            | 0.247 | 0.235  | 0.249  |
| Pyridazine            | 2B <sub>2u</sub> | 1B <sub>3g</sub> | 0.683            | 0.202 | 0.201  | 0.202  | 0.677            | 0.240 | 0.235  | 0.240  |
|                       | 1A <sub>2</sub>  | 2B <sub>1</sub>  | 2.036            | 0.013 | -0.020 | -0.012 | 2.098            | 0.018 | 0.016  | -0.019 |
| Pyrrole               | 1A <sub>2</sub>  | 1B <sub>1</sub>  | 0.679            | 0.084 | 0.094  | -0.089 | 0.669            | 0.066 | 0.060  | -0.064 |
|                       | 1A <sub>2</sub>  | 2A <sub>2</sub>  | 0.717            | 0.184 | 0.163  | 0.186  | 0.700            | 0.188 | 0.181  | 0.189  |

| Molecule   | State1           | State2           | QR-CCSD/dAVDZ    |       |       |        | QR-CC2/dAVDZ     |       |       |        |
|------------|------------------|------------------|------------------|-------|-------|--------|------------------|-------|-------|--------|
|            |                  |                  | $\Delta E_{m,n}$ | $f^l$ | $f^v$ | $f^m$  | $\Delta E_{m,n}$ | $f^l$ | $f^v$ | $f^m$  |
| Silylidene | 1A <sub>2</sub>  | 1B <sub>2</sub>  | 1.586            | 0.003 | 0.003 | -0.003 | 1.478            | 0.003 | 0.001 | -0.003 |
| Tetrazine  | 1B <sub>3u</sub> | 1B <sub>1g</sub> | 2.652            | 0.077 | 0.004 | 0.087  | 2.673            | 0.104 | 0.087 | 0.117  |
|            | 1B <sub>3u</sub> | 1B <sub>2g</sub> | 3.230            | 0.027 | 0.015 | 0.032  | 3.301            | 0.035 | 0.028 | 0.037  |
| Thiophene  | 1A <sub>2</sub>  | 1B <sub>1</sub>  | 0.206            | 0.042 | 0.002 | -0.042 | 0.216            | 0.056 | 0.030 | -0.057 |
|            | 1B <sub>1</sub>  | 1A <sub>2</sub>  | 1.750            | 0.294 | 0.291 | 0.294  | 1.626            | 0.316 | 0.303 | 0.311  |
| Water      |                  |                  |                  |       |       |        |                  |       |       |        |

Table S29: Excited State absorption data for QR-CC3/AVTZ and QR-CCSD/AVTZ calculations.  $\Delta E_{m,n}$ [eV] and oscillator strengths in length, velocity, and mixed gauges,  $f^l$ ,  $f^v$ , and  $f^m$ , respectively.

| Molecule        | State1           | State2           | QR-CC3/AVTZ      |       |       |        | QR-CCSD/AVTZ     |       |       |        |
|-----------------|------------------|------------------|------------------|-------|-------|--------|------------------|-------|-------|--------|
|                 |                  |                  | $\Delta E_{m,n}$ | $f^l$ | $f^v$ | $f^m$  | $\Delta E_{m,n}$ | $f^l$ | $f^v$ | $f^m$  |
| Acetone         | 1B <sub>2</sub>  | 2A <sub>1</sub>  | 1.057            | 0.257 | 0.260 | -0.258 | 1.040            | 0.266 | 0.251 | -0.267 |
|                 | 1B <sub>2</sub>  | 2B <sub>2</sub>  | 1.167            | 0.278 | 0.237 | 0.257  | 1.115            | 0.286 | 0.223 | 0.265  |
|                 | 1B <sub>2</sub>  | 2A <sub>2</sub>  | 1.021            | 0.346 | 0.367 | 0.356  | 0.981            | 0.354 | 0.333 | 0.364  |
| Acrolein        | 1A''             | 2A''             | 3.009            | 0.036 | 0.040 | 0.038  | 3.356            | 0.049 | 0.038 | 0.048  |
| Ammonia         | 1A <sub>2</sub>  | 1E               | 1.573            | 0.316 | 0.315 | 0.316  | 1.548            | 0.319 | 0.319 | 0.320  |
|                 | 1A <sub>2</sub>  | 2A <sub>1</sub>  | 2.746            | 0.331 | 0.207 | 0.262  | 2.734            | 0.333 | 0.201 | 0.260  |
|                 | 1E               | 2A <sub>2</sub>  | 1.799            | 0.236 | 0.211 | 0.223  | 1.804            | 0.238 | 0.209 | 0.223  |
| Benzene         | 2A <sub>1</sub>  | 2A <sub>2</sub>  | 0.627            | 0.020 | 0.992 | 0.141  | 0.619            | 0.018 | 1.010 | 0.136  |
|                 | 1E <sub>1g</sub> | 1A <sub>2u</sub> | 0.559            | 0.130 | 0.129 | -0.130 | 0.540            | 0.131 | 0.094 | -0.123 |
|                 | 1E <sub>1g</sub> | 1E <sub>2u</sub> | 0.627            | 0.136 | 0.136 | 0.136  | 0.620            | 0.140 | 0.134 | 0.150  |
| Butadiene       | 1B <sub>g</sub>  | 1A <sub>u</sub>  | 0.313            | 0.113 | 0.117 | -0.115 | 0.315            | 0.118 | 0.057 | -0.122 |
|                 | 1B <sub>g</sub>  | 2A <sub>u</sub>  | 0.469            | 0.155 | 0.168 | -0.162 | 0.475            | 0.158 | 0.162 | -0.167 |
|                 | 1A <sub>u</sub>  | 2B <sub>g</sub>  | 0.894            | 0.068 | 0.078 | 0.073  | 0.890            | 0.067 | 0.077 | 0.073  |
| Carbon monoxide | 2A <sub>u</sub>  | 2B <sub>g</sub>  | 0.738            | 0.335 | 0.307 | 0.321  | 0.729            | 0.343 | 0.309 | 0.331  |
|                 | 2Σ <sup>+</sup>  | 3Σ <sup>+</sup>  | 0.545            | 0.056 | 0.158 | 0.094  | 0.529            | 0.061 | 0.161 | 0.101  |
|                 | 2Σ <sup>+</sup>  | 2Π               | 0.747            | 0.144 | 0.341 | 0.222  | 0.738            | 0.145 | 0.358 | 0.229  |
|                 | 2Π               | 1Π               | 3.204            | 0.013 | 0.013 | 0.013  | 3.373            | 0.013 | 0.011 | 0.013  |
|                 | 2Σ <sup>+</sup>  | 1Π               | 2.457            | 0.025 | 0.020 | -0.022 | 2.635            | 0.024 | 0.019 | -0.022 |
|                 | 3Σ <sup>+</sup>  | 1Π               | 3.002            | 0.017 | 0.019 | -0.018 | 3.164            | 0.014 | 0.017 | -0.016 |
| Cyclopentadiene | 1B <sub>2</sub>  | 2A <sub>1</sub>  | 1.030            | 0.023 | 0.032 | -0.027 | 1.295            | 0.047 | 0.002 | -0.066 |
|                 | 1A <sub>2</sub>  | 1B <sub>1</sub>  | 0.630            | 0.227 | 0.232 | -0.230 | 0.616            | 0.230 | 0.222 | -0.235 |
|                 | 1A <sub>2</sub>  | 2B <sub>2</sub>  | 0.783            | 0.260 | 0.230 | -0.245 | 0.774            | 0.265 | 0.208 | -0.247 |

| Molecule              | State1           | State2           | QR-CC3/AVTZ      |       |       |        | QR-CCSD/AVTZ     |       |        |        |
|-----------------------|------------------|------------------|------------------|-------|-------|--------|------------------|-------|--------|--------|
|                       |                  |                  | $\Delta E_{m,n}$ | $f^l$ | $f^v$ | $f^m$  | $\Delta E_{m,n}$ | $f^l$ | $f^v$  | $f^m$  |
| Cyclopropene          | 1A <sub>2</sub>  | 2A <sub>2</sub>  | 0.674            | 0.245 | 0.240 | 0.243  | 0.669            | 0.255 | 0.215  | 0.256  |
|                       | 2B <sub>1</sub>  | 3B <sub>1</sub>  | 0.386            | 0.099 | 0.085 | 0.092  | 0.391            | 0.103 | 0.070  | 0.097  |
|                       | 1B <sub>1</sub>  | 2A <sub>1</sub>  | 3.924            | 0.014 | 0.015 | -0.015 | 3.930            | 0.015 | 0.015  | -0.015 |
|                       | 1B <sub>2</sub>  | 2A <sub>1</sub>  | 0.587            | 0.076 | 0.049 | -0.061 | 0.561            | 0.081 | 0.041  | -0.062 |
| Diazomethane          | 1A <sub>2</sub>  | 1B <sub>1</sub>  | 2.380            | 0.012 | 0.012 | -0.012 | 2.380            | 0.012 | 0.011  | -0.011 |
|                       | 1B <sub>2</sub>  | 2A <sub>1</sub>  | 1.003            | 0.295 | 0.298 | -0.296 | 0.980            | 0.299 | 0.290  | -0.299 |
| Formaldehyde          | 1B <sub>2</sub>  | 2A <sub>2</sub>  | 1.457            | 0.290 | 0.213 | 0.248  | 1.420            | 0.299 | 0.215  | 0.256  |
|                       | 1A <sub>2</sub>  | 1B <sub>2</sub>  | 3.209            | 0.020 | 0.020 | -0.020 | 3.218            | 0.020 | 0.018  | -0.019 |
|                       | 2B <sub>2</sub>  | 2A <sub>2</sub>  | 0.549            | 0.008 | 0.016 | 0.011  | 0.530            | 0.006 | 0.012  | 0.009  |
|                       | 1A <sub>2</sub>  | 2A <sub>2</sub>  | 4.666            | 0.018 | 0.017 | 0.018  | 4.638            | 0.019 | 0.017  | 0.018  |
| Furane                | 1A <sub>2</sub>  | 2B <sub>2</sub>  | 1.155            | 0.276 | 0.136 | -0.194 | 1.157            | 0.278 | 0.124  | -0.193 |
|                       | 1A <sub>2</sub>  | 1B <sub>1</sub>  | 0.552            | 0.220 | 0.201 | -0.210 | 0.540            | 0.219 | 0.185  | -0.212 |
|                       | 1A <sub>2</sub>  | 2A <sub>2</sub>  | 0.721            | 0.258 | 0.254 | 0.256  | 0.722            | 0.264 | 0.238  | 0.264  |
|                       | 1A <sub>u</sub>  | 1B <sub>g</sub>  | 1.393            | 0.020 | 0.021 | 0.021  | 1.408            | 0.019 | -0.021 | 0.023  |
| Glyoxal               | 1A <sub>u</sub>  | 2B <sub>g</sub>  | 3.702            | 0.114 | 0.119 | 0.117  | 4.114            | 0.157 | 0.145  | 0.160  |
|                       | 1B <sub>1</sub>  | 2A <sub>2</sub>  | 1.201            | 0.336 | 0.327 | 0.332  | 1.198            | 0.340 | 0.324  | 0.337  |
| Ketene                | 1B <sub>1</sub>  | 2A <sub>1</sub>  | 1.276            | 0.127 | 0.087 | -0.106 | 1.263            | 0.128 | 0.092  | -0.109 |
|                       | 1B <sub>1</sub>  | 1A <sub>2</sub>  | 0.515            | 0.182 | 0.175 | 0.178  | 0.520            | 0.192 | 0.153  | 0.192  |
| Methylenecyclopropene | 1B <sub>2</sub>  | 1A <sub>2</sub>  | 1.642            | 0.023 | 0.026 | 0.025  | 1.416            | 0.024 | 0.027  | 0.025  |
|                       | 2A <sub>g</sub>  | 2B <sub>1u</sub> | 0.798            | 0.182 | 0.186 | 0.184  | 0.766            | 0.175 | 0.181  | 0.179  |
| Pyrazine              | 2A <sub>g</sub>  | 2B <sub>2u</sub> | 0.597            | 0.245 | 0.220 | 0.232  | 0.611            | 0.259 | 0.140  | 0.248  |
|                       | 1B <sub>1u</sub> | 1B <sub>3g</sub> | 1.139            | 0.004 | 0.004 | 0.004  | 1.198            | 0.007 | 0.006  | 0.007  |
|                       | 2B <sub>2u</sub> | 1B <sub>3g</sub> | 0.748            | 0.184 | 0.191 | 0.188  | 0.715            | 0.180 | 0.186  | 0.183  |
|                       | 1A <sub>2</sub>  | 2B <sub>1</sub>  | 1.995            | 0.012 | 0.010 | -0.011 | 2.014            | 0.011 | -0.021 | -0.012 |
| Pyrrole               | 1A <sub>2</sub>  | 1B <sub>1</sub>  | 0.741            | 0.069 | 0.069 | -0.069 | 0.698            | 0.077 | 0.087  | -0.082 |
|                       | 1A <sub>2</sub>  | 2A <sub>2</sub>  | 0.772            | 0.167 | 0.165 | 0.166  | 0.748            | 0.180 | 0.155  | 0.182  |

| Molecule   | State1           | State2           | QR-CC3/AVTZ      |       |       |        | QR-CCSD/AVTZ     |       |        |        |
|------------|------------------|------------------|------------------|-------|-------|--------|------------------|-------|--------|--------|
|            |                  |                  | $\Delta E_{m,n}$ | $f^l$ | $f^v$ | $f^m$  | $\Delta E_{m,n}$ | $f^l$ | $f^v$  | $f^m$  |
| Silylidene | 1A <sub>2</sub>  | 1B <sub>2</sub>  | 1.626            | 0.003 | 0.002 | -0.003 | 1.591            | 0.003 | 0.002  | -0.002 |
| Tetrazine  | 1B <sub>3u</sub> | 1B <sub>1g</sub> | 2.455            | 0.061 | 0.069 | 0.065  | 2.628            | 0.074 | -0.007 | 0.084  |
|            | 1B <sub>3u</sub> | 1B <sub>2g</sub> | 3.009            | 0.017 | 0.017 | 0.017  | 3.200            | 0.027 | 0.016  | 0.033  |
| Thiophene  | 1A <sub>2</sub>  | 1B <sub>1</sub>  | 0.005            | 0.000 | 0.005 | 0.003  | 0.089            | 0.011 | -0.073 | -0.006 |
| Water      | 1B <sub>1</sub>  | 1A <sub>2</sub>  | 1.778            | 0.288 | 0.281 | 0.284  | 1.765            | 0.292 | 0.286  | 0.291  |



Table S30: Excited State absorption data for QR-CC2/AVTZ and QR-CC3/dAVTZ calculations.  $\Delta E_{m,n}[\text{eV}]$  and oscillator strengths in length, velocity, and mixed gauges,  $f^l$ ,  $f^v$ , and  $f^m$ , respectively.

| Molecule        | State1           | State2           | QR-CC2/AVTZ      |       |       | QR-CC3/dAVTZ |                  |       |       |        |
|-----------------|------------------|------------------|------------------|-------|-------|--------------|------------------|-------|-------|--------|
|                 |                  |                  | $\Delta E_{m,n}$ | $f^l$ | $f^v$ | $f^m$        | $\Delta E_{m,n}$ | $f^l$ | $f^v$ | $f^m$  |
| Acetone         | 1B <sub>2</sub>  | 2A <sub>1</sub>  | 0.975            | 0.279 | 0.279 | -0.284       | 1.032            | 0.256 | 0.259 | -0.257 |
|                 | 1B <sub>2</sub>  | 2B <sub>2</sub>  | 1.111            | 0.297 | 0.242 | 0.271        | 1.037            | 0.267 | 0.268 | 0.268  |
|                 | 1B <sub>2</sub>  | 2A <sub>2</sub>  | 0.930            | 0.359 | 0.367 | 0.367        | 0.964            | 0.361 | 0.364 | 0.363  |
| Acrolein        | 1A''             | 2A''             | 2.828            | 0.079 | 0.077 | 0.081        | 3.002            | 0.036 | 0.039 | 0.037  |
| Ammonia         | 1A <sub>2</sub>  | 1E               | 1.460            | 0.330 | 0.321 | 0.326        | 1.545            | 0.320 | 0.321 | 0.321  |
|                 | 1A <sub>2</sub>  | 2A <sub>1</sub>  | 2.664            | 0.345 | 0.188 | 0.255        | 1.992            | 0.295 | 0.296 | 0.296  |
|                 | 1E               | 2A <sub>2</sub>  | 1.807            | 0.249 | 0.198 | 0.222        | 1.003            | 0.139 | 0.143 | 0.141  |
| Benzene         | 2A <sub>1</sub>  | 2A <sub>2</sub>  | 0.603            | 0.011 | 1.130 | 0.112        | 0.556            | 0.252 | 0.278 | 0.264  |
|                 | 1E <sub>1g</sub> | 1A <sub>2u</sub> | 0.532            | 0.138 | 0.136 | -0.143       | 0.549            | 0.132 | 0.133 | -0.133 |
|                 | 1E <sub>1g</sub> | 1E <sub>2u</sub> | 0.594            | 0.143 | 0.129 | 0.143        | 0.613            | 0.138 | 0.140 | 0.139  |
| Butadiene       | 1B <sub>g</sub>  | 1A <sub>u</sub>  | 0.316            | 0.125 | 0.116 | -0.133       | 0.316            | 0.122 | 0.124 | -0.124 |
|                 | 1B <sub>g</sub>  | 2A <sub>u</sub>  | 0.446            | 0.169 | 0.171 | -0.182       | 0.470            | 0.165 | 0.167 | -0.166 |
|                 | 1A <sub>u</sub>  | 2B <sub>g</sub>  | 0.853            | 0.071 | 0.084 | 0.078        | 0.821            | 0.062 | 0.062 | 0.062  |
| Carbon monoxide | 2A <sub>u</sub>  | 2B <sub>g</sub>  | 0.723            | 0.368 | 0.330 | 0.354        | 0.667            | 0.367 | 0.369 | 0.368  |
|                 | 2Σ <sup>+</sup>  | 3Σ <sup>+</sup>  | 0.520            | 0.055 | 0.167 | 0.098        | 0.609            | 0.146 | 0.146 | 0.147  |
|                 | 2Σ <sup>+</sup>  | 2Π               | 0.720            | 0.141 | 0.343 | 0.221        | 0.738            | 0.256 | 0.261 | 0.258  |
| Cyclopentadiene | 2Π               | 1Π               | 3.187            | 0.015 | 0.012 | 0.013        | 2.933            | 0.010 | 0.009 | 0.009  |
|                 | 2Σ <sup>+</sup>  | 1Π               | 2.467            | 0.020 | 0.010 | -0.015       | 2.195            | 0.025 | 0.025 | -0.025 |
|                 | 3Σ <sup>+</sup>  | 1Π               | 2.987            | 0.017 | 0.018 | -0.017       | 2.804            | 0.010 | 0.010 | -0.010 |
| Cyclopentadiene | 1B <sub>2</sub>  | 2A <sub>1</sub>  | 1.338            | 0.062 | 0.067 | -0.079       | 1.029            | 0.023 | 0.032 | -0.027 |
|                 | 1A <sub>2</sub>  | 1B <sub>1</sub>  | 0.597            | 0.241 | 0.239 | -0.248       | 0.616            | 0.235 | 0.236 | -0.236 |
|                 | 1A <sub>2</sub>  | 2B <sub>2</sub>  | 0.762            | 0.269 | 0.237 | -0.253       | 0.689            | 0.282 | 0.284 | -0.283 |

| Molecule              | State1           | State2           | QR-CC2/AVTZ      |       |        |        | QR-CC3/dAVTZ     |       |       |        |
|-----------------------|------------------|------------------|------------------|-------|--------|--------|------------------|-------|-------|--------|
|                       |                  |                  | $\Delta E_{m,n}$ | $f^l$ | $f^v$  | $f^m$  | $\Delta E_{m,n}$ | $f^l$ | $f^v$ | $f^m$  |
| Cyclopropene          | 1A <sub>2</sub>  | 2A <sub>2</sub>  | 0.644            | 0.260 | 0.248  | 0.263  | 0.653            | 0.252 | 0.254 | 0.253  |
|                       | 2B <sub>1</sub>  | 3B <sub>1</sub>  | 0.396            | 0.107 | 0.089  | 0.103  | 0.373            | 0.103 | 0.102 | 0.103  |
|                       | 1B <sub>1</sub>  | 2A <sub>1</sub>  | 3.604            | 0.015 | 0.014  | -0.015 | 3.859            | 0.014 | 0.015 | -0.014 |
|                       | 1B <sub>2</sub>  | 2A <sub>1</sub>  | 0.552            | 0.091 | 0.057  | -0.072 | 0.530            | 0.085 | 0.084 | -0.084 |
| Diazomethane          | 1A <sub>2</sub>  | 1B <sub>1</sub>  | 2.161            | 0.013 | 0.011  | -0.012 | 2.364            | 0.012 | 0.012 | -0.012 |
|                       | 1B <sub>2</sub>  | 2A <sub>1</sub>  | 0.960            | 0.302 | 0.304  | -0.304 | 0.972            | 0.297 | 0.301 | -0.299 |
| Formaldehyde          | 1B <sub>2</sub>  | 2A <sub>2</sub>  | 1.485            | 0.306 | 0.213  | 0.256  | 1.214            | 0.278 | 0.279 | 0.279  |
|                       | 1A <sub>2</sub>  | 1B <sub>2</sub>  | 2.486            | 0.021 | 0.023  | -0.022 | 3.205            | 0.019 | 0.020 | -0.020 |
|                       | 2B <sub>2</sub>  | 2A <sub>2</sub>  | 0.475            | 0.011 | 0.022  | 0.016  | 0.392            | 0.011 | 0.011 | 0.011  |
|                       | 1A <sub>2</sub>  | 2A <sub>2</sub>  | 3.971            | 0.021 | 0.018  | 0.020  | 4.419            | 0.015 | 0.014 | 0.014  |
| Furane                | 1A <sub>2</sub>  | 2B <sub>2</sub>  | 1.190            | 0.284 | 0.126  | -0.189 | 0.822            | 0.271 | 0.272 | -0.271 |
|                       | 1A <sub>2</sub>  | 1B <sub>1</sub>  | 0.529            | 0.232 | 0.200  | -0.225 | 0.544            | 0.220 | 0.220 | -0.220 |
|                       | 1A <sub>2</sub>  | 2A <sub>2</sub>  | 0.695            | 0.268 | 0.262  | 0.270  | 0.693            | 0.268 | 0.269 | 0.269  |
|                       | 1A <sub>u</sub>  | 1B <sub>g</sub>  | 1.525            | 0.035 | -0.009 | 0.038  | 1.393            | 0.020 | 0.021 | 0.021  |
| Glyoxal               | 1A <sub>u</sub>  | 2B <sub>g</sub>  | 3.598            | 0.178 | 0.186  | 0.188  | 3.692            | 0.113 | 0.117 | 0.115  |
|                       | 1B <sub>1</sub>  | 2A <sub>2</sub>  | 1.144            | 0.346 | 0.330  | 0.340  | 1.161            | 0.336 | 0.338 | 0.337  |
| Ketene                | 1B <sub>1</sub>  | 2A <sub>1</sub>  | 1.318            | 0.175 | 0.126  | -0.149 | 1.136            | 0.176 | 0.174 | -0.175 |
|                       | 1B <sub>1</sub>  | 1A <sub>2</sub>  | 0.497            | 0.194 | 0.192  | 0.196  | 0.506            | 0.188 | 0.189 | 0.189  |
| Methylenecyclopropene | 1B <sub>2</sub>  | 1A <sub>2</sub>  | 1.344            | 0.023 | 0.028  | 0.026  | 1.616            | 0.023 | 0.025 | 0.024  |
|                       | 2A <sub>g</sub>  | 2B <sub>1u</sub> | 0.827            | 0.185 | 0.191  | 0.191  | 0.771            | 0.198 | 0.197 | 0.198  |
| Pyrazine              | 2A <sub>g</sub>  | 2B <sub>2u</sub> | 0.537            | 0.270 | 0.202  | 0.257  | 0.591            | 0.240 | 0.244 | 0.242  |
|                       | 1B <sub>1u</sub> | 1B <sub>3g</sub> | 0.585            | 0.075 | 0.057  | 0.068  | 1.090            | 0.004 | 0.004 | 0.004  |
|                       | 2B <sub>2u</sub> | 1B <sub>3g</sub> | 0.732            | 0.213 | 0.223  | 0.221  | 0.722            | 0.201 | 0.201 | 0.201  |
|                       | 1A <sub>2</sub>  | 2B <sub>1</sub>  | 2.074            | 0.018 | 0.019  | -0.021 | 1.995            | 0.012 | 0.010 | -0.011 |
| Pyridazine            | 1A <sub>2</sub>  | 1B <sub>1</sub>  | 0.684            | 0.036 | 0.031  | -0.035 | 0.734            | 0.091 | 0.091 | -0.091 |
|                       | 1A <sub>2</sub>  | 2A <sub>2</sub>  | 0.739            | 0.181 | 0.175  | 0.183  | 0.747            | 0.171 | 0.171 | 0.171  |

| Molecule   | State1           | State2           | QR-CC2/AVTZ      |       |        |        | QR-CC3/dAVTZ     |       |        |        |
|------------|------------------|------------------|------------------|-------|--------|--------|------------------|-------|--------|--------|
|            |                  |                  | $\Delta E_{m,n}$ | $f^l$ | $f^v$  | $f^m$  | $\Delta E_{m,n}$ | $f^l$ | $f^v$  | $f^m$  |
| Silylidene | 1A <sub>2</sub>  | 1B <sub>2</sub>  | 1.487            | 0.003 | 0.000  | -0.002 | 1.624            | 0.003 | 0.002  | -0.003 |
| Tetrazine  | 1B <sub>3u</sub> | 1B <sub>1g</sub> | 2.637            | 0.100 | 0.083  | 0.114  | 2.456            | 0.061 | 0.068  | 0.065  |
|            | 1B <sub>3u</sub> | 1B <sub>2g</sub> | 3.262            | 0.034 | 0.030  | 0.038  | 3.009            | 0.017 | 0.017  | 0.017  |
| Thiophene  | 1A <sub>2</sub>  | 1B <sub>1</sub>  | 0.085            | 0.013 | -0.041 | -0.012 | 0.009            | 0.001 | -0.004 | -0.000 |
| Water      | 1B <sub>1</sub>  | 1A <sub>2</sub>  | 1.655            | 0.316 | 0.302  | 0.310  | 1.768            | 0.283 | 0.284  | 0.283  |

Table S31: Excited State absorption data for QR-CCSD/dAVTZ and QR-CC2/dAVTZ calculations.  $\Delta E_{m,n}$ [eV] and oscillator strengths in length, velocity, and mixed gauges,  $f^l$ ,  $f^v$ , and  $f^m$ , respectively.

| Molecule        | State1           | State2           | QR-CCSD/dAVTZ    |       |       |        | QR-CC2/dAVTZ     |       |       |        |
|-----------------|------------------|------------------|------------------|-------|-------|--------|------------------|-------|-------|--------|
|                 |                  |                  | $\Delta E_{m,n}$ | $f^l$ | $f^v$ | $f^m$  | $\Delta E_{m,n}$ | $f^l$ | $f^v$ | $f^m$  |
| Acetone         | 1B <sub>2</sub>  | 2A <sub>1</sub>  | 1.011            | 0.264 | 0.252 | -0.265 | 0.928            | 0.279 | 0.273 | -0.280 |
|                 | 1B <sub>2</sub>  | 2B <sub>2</sub>  | 0.989            | 0.275 | 0.256 | 0.276  | 0.935            | 0.287 | 0.281 | 0.286  |
|                 | 1B <sub>2</sub>  | 2A <sub>2</sub>  | 0.910            | 0.370 | 0.329 | 0.370  | 0.852            | 0.377 | 0.360 | 0.372  |
| Acrolein        | 1A''             | 2A''             | 3.343            | 0.048 | 0.037 | 0.046  | 2.798            | 0.073 | 0.070 | 0.075  |
| Ammonia         | 1A <sub>2</sub>  | 1E               | 1.520            | 0.323 | 0.324 | 0.325  | 1.417            | 0.333 | 0.326 | 0.330  |
|                 | 1A <sub>2</sub>  | 2A <sub>1</sub>  | 1.965            | 0.296 | 0.293 | 0.295  | 1.790            | 0.307 | 0.301 | 0.304  |
|                 | 1E               | 2A <sub>2</sub>  | 0.990            | 0.141 | 0.144 | 0.142  | 0.860            | 0.159 | 0.160 | 0.159  |
| Benzene         | 2A <sub>1</sub>  | 2A <sub>2</sub>  | 0.544            | 0.249 | 0.276 | 0.262  | 0.487            | 0.210 | 0.266 | 0.236  |
|                 | 1E <sub>1g</sub> | 1A <sub>2u</sub> | 0.530            | 0.134 | 0.100 | -0.127 | 0.518            | 0.143 | 0.139 | -0.146 |
|                 | 1E <sub>1g</sub> | 1E <sub>2u</sub> | 0.606            | 0.142 | 0.139 | 0.153  | 0.576            | 0.148 | 0.132 | 0.146  |
|                 | 1B <sub>g</sub>  | 1A <sub>u</sub>  | 0.317            | 0.128 | 0.070 | -0.131 | 0.318            | 0.139 | 0.126 | -0.143 |
| Butadiene       | 1B <sub>g</sub>  | 2A <sub>u</sub>  | 0.476            | 0.169 | 0.161 | -0.172 | 0.447            | 0.184 | 0.169 | -0.188 |
|                 | 1A <sub>u</sub>  | 2B <sub>g</sub>  | 0.812            | 0.058 | 0.057 | 0.059  | 0.758            | 0.060 | 0.060 | 0.060  |
|                 | 2A <sub>u</sub>  | 2B <sub>g</sub>  | 0.654            | 0.379 | 0.378 | 0.383  | 0.630            | 0.410 | 0.410 | 0.414  |
| Carbon monoxide | 2Σ <sup>+</sup>  | 3Σ <sup>+</sup>  | 0.606            | 0.146 | 0.145 | 0.147  | 0.580            | 0.154 | 0.158 | 0.158  |
|                 | 2Σ <sup>+</sup>  | 2Π               | 0.740            | 0.254 | 0.258 | 0.258  | 0.702            | 0.258 | 0.263 | 0.261  |
|                 | 2Π               | 1Π               | 3.118            | 0.011 | 0.008 | 0.010  | 2.881            | 0.011 | 0.008 | 0.010  |
| Cyclopentadiene | 2Σ <sup>+</sup>  | 1Π               | 2.378            | 0.024 | 0.023 | -0.024 | 2.180            | 0.021 | 0.016 | -0.018 |
|                 | 3Σ <sup>+</sup>  | 1Π               | 2.984            | 0.008 | 0.009 | -0.009 | 2.760            | 0.009 | 0.010 | -0.009 |
|                 | 1B <sub>2</sub>  | 2A <sub>1</sub>  | 1.284            | 0.046 | 0.004 | -0.065 | 1.315            | 0.059 | 0.064 | -0.074 |
|                 | 1A <sub>2</sub>  | 1B <sub>1</sub>  | 0.600            | 0.240 | 0.226 | -0.241 | 0.577            | 0.254 | 0.241 | -0.255 |
|                 | 1A <sub>2</sub>  | 2B <sub>2</sub>  | 0.673            | 0.288 | 0.266 | -0.288 | 0.652            | 0.294 | 0.297 | -0.296 |
|                 |                  |                  |                  |       |       |        |                  |       |       |        |

| Molecule              | State1           | State2           | QR-CCSD/dAVTZ    |       |        |        | QR-CC2/dAVTZ     |       |        |        |
|-----------------------|------------------|------------------|------------------|-------|--------|--------|------------------|-------|--------|--------|
|                       |                  |                  | $\Delta E_{m,n}$ | $f^l$ | $f^v$  | $f^m$  | $\Delta E_{m,n}$ | $f^l$ | $f^v$  | $f^m$  |
| Cyclopropene          | 1A <sub>2</sub>  | 2A <sub>2</sub>  | 0.647            | 0.262 | 0.231  | 0.266  | 0.616            | 0.272 | 0.261  | 0.275  |
|                       | 2B <sub>1</sub>  | 3B <sub>1</sub>  | 0.377            | 0.107 | 0.089  | 0.108  | 0.378            | 0.111 | 0.106  | 0.113  |
|                       | 1B <sub>1</sub>  | 2A <sub>1</sub>  | 3.863            | 0.014 | 0.015  | -0.014 | 3.517            | 0.014 | 0.014  | -0.014 |
|                       | 1B <sub>2</sub>  | 2A <sub>1</sub>  | 0.503            | 0.090 | 0.078  | -0.088 | 0.478            | 0.103 | 0.108  | -0.106 |
| Diazomethane          | 1A <sub>2</sub>  | 1B <sub>1</sub>  | 2.364            | 0.012 | 0.011  | -0.012 | 2.141            | 0.012 | 0.011  | -0.012 |
|                       | 1B <sub>2</sub>  | 2A <sub>1</sub>  | 0.945            | 0.300 | 0.296  | -0.302 | 0.923            | 0.301 | 0.305  | -0.304 |
| Formaldehyde          | 1B <sub>2</sub>  | 2A <sub>2</sub>  | 1.168            | 0.288 | 0.284  | 0.288  | 1.164            | 0.289 | 0.288  | 0.288  |
|                       | 1A <sub>2</sub>  | 1B <sub>2</sub>  | 3.213            | 0.019 | 0.018  | -0.019 | 2.480            | 0.020 | 0.024  | -0.022 |
|                       | 2B <sub>2</sub>  | 2A <sub>2</sub>  | 0.366            | 0.008 | 0.008  | 0.009  | 0.288            | 0.012 | 0.014  | 0.013  |
|                       | 1A <sub>2</sub>  | 2A <sub>2</sub>  | 4.381            | 0.015 | 0.014  | 0.014  | 3.643            | 0.016 | 0.014  | 0.015  |
| Furane                | 1A <sub>2</sub>  | 2B <sub>2</sub>  | 0.819            | 0.264 | 0.255  | -0.264 | 0.813            | 0.257 | 0.255  | -0.256 |
|                       | 1A <sub>2</sub>  | 1B <sub>1</sub>  | 0.533            | 0.220 | 0.205  | -0.221 | 0.519            | 0.235 | 0.221  | -0.236 |
|                       | 1A <sub>2</sub>  | 2A <sub>2</sub>  | 0.693            | 0.274 | 0.255  | 0.277  | 0.661            | 0.282 | 0.277  | 0.284  |
|                       | 1A <sub>u</sub>  | 1B <sub>g</sub>  | 1.408            | 0.019 | -0.021 | 0.022  | 1.524            | 0.035 | -0.009 | 0.038  |
| Glyoxal               | 1A <sub>u</sub>  | 2B <sub>g</sub>  | 4.098            | 0.153 | 0.141  | 0.156  | 3.580            | 0.173 | 0.180  | 0.183  |
|                       | 1B <sub>1</sub>  | 2A <sub>2</sub>  | 1.159            | 0.340 | 0.334  | 0.341  | 1.098            | 0.345 | 0.343  | 0.346  |
| Ketene                | 1B <sub>1</sub>  | 2A <sub>1</sub>  | 1.126            | 0.175 | 0.176  | -0.176 | 1.116            | 0.221 | 0.228  | -0.224 |
| Methylenecyclopropene | 1B <sub>1</sub>  | 1A <sub>2</sub>  | 0.510            | 0.199 | 0.169  | 0.202  | 0.487            | 0.206 | 0.205  | 0.208  |
|                       | 1B <sub>2</sub>  | 1A <sub>2</sub>  | 1.388            | 0.025 | 0.024  | 0.024  | 1.311            | 0.024 | 0.025  | 0.024  |
|                       | 2A <sub>g</sub>  | 2B <sub>1u</sub> | 0.737            | 0.192 | 0.192  | 0.192  | 0.802            | 0.136 | 0.132  | 0.136  |
|                       | 2A <sub>g</sub>  | 2B <sub>2u</sub> | 0.603            | 0.252 | 0.174  | 0.257  | 0.525            | 0.267 | 0.236  | 0.271  |
| Pyrazine              | 1B <sub>1u</sub> | 1B <sub>3g</sub> | 1.143            | 0.007 | 0.007  | 0.007  | 0.522            | 0.141 | 0.137  | 0.143  |
|                       | 2B <sub>2u</sub> | 1B <sub>3g</sub> | 0.686            | 0.200 | 0.198  | 0.199  | 0.683            | 0.238 | 0.233  | 0.238  |
|                       | 1A <sub>2</sub>  | 2B <sub>1</sub>  | 2.014            | 0.011 | -0.021 | -0.012 | 2.074            | 0.018 | 0.019  | -0.020 |
|                       | 1A <sub>2</sub>  | 1B <sub>1</sub>  | 0.690            | 0.098 | 0.108  | -0.103 | 0.678            | 0.061 | 0.054  | -0.059 |
| Pyrrole               | 1A <sub>2</sub>  | 2A <sub>2</sub>  | 0.722            | 0.185 | 0.162  | 0.188  | 0.708            | 0.187 | 0.182  | 0.189  |

| Molecule   | State1           | State2           | QR-CCSD/dAVTZ    |       |        |        | QR-CC2/dAVTZ     |       |        |        |
|------------|------------------|------------------|------------------|-------|--------|--------|------------------|-------|--------|--------|
|            |                  |                  | $\Delta E_{m,n}$ | $f^l$ | $f^v$  | $f^m$  | $\Delta E_{m,n}$ | $f^l$ | $f^v$  | $f^m$  |
| Silylidene | 1A <sub>2</sub>  | 1B <sub>2</sub>  | 1.590            | 0.003 | 0.002  | -0.002 | 1.485            | 0.003 | 0.000  | -0.002 |
| Tetrazine  | 1B <sub>3u</sub> | 1B <sub>1g</sub> | 2.629            | 0.074 | -0.007 | 0.084  | 2.637            | 0.100 | 0.083  | 0.114  |
|            | 1B <sub>3u</sub> | 1B <sub>2g</sub> | 3.201            | 0.027 | 0.016  | 0.033  | 3.262            | 0.034 | 0.030  | 0.038  |
| Thiophene  | 1A <sub>2</sub>  | 1B <sub>1</sub>  | 0.103            | 0.013 | -0.057 | -0.011 | 0.102            | 0.016 | -0.022 | -0.018 |
| Water      | 1B <sub>1</sub>  | 1A <sub>2</sub>  | 1.756            | 0.287 | 0.288  | 0.289  | 1.641            | 0.312 | 0.302  | 0.308  |

### **S3.4 Full testing set, ISR-ADC2 with AVDZ, dAVDZ, AVTZ, and dAVTZ basis sets**

Table S32: Excited State absorption data for ISR-ADC(2) obtained with AVDZ, dAVDZ, AVTZ and dAVTZ basis sets.  $\Delta E_{m,n}$ [eV] and oscillator strengths in length gauge ( $f^l$ ).

| Molecule        | State1           | State2           | AVDZ             |       |                  | dAVDZ            |       |                  | AVTZ             |       |                  | dAVTZ            |       |                  |
|-----------------|------------------|------------------|------------------|-------|------------------|------------------|-------|------------------|------------------|-------|------------------|------------------|-------|------------------|
|                 |                  |                  | $\Delta E_{m,n}$ | $f^l$ | $\Delta E_{m,n}$ | $\Delta E_{m,n}$ | $f^l$ | $\Delta E_{m,n}$ | $\Delta E_{m,n}$ | $f^l$ | $\Delta E_{m,n}$ | $\Delta E_{m,n}$ | $f^l$ | $\Delta E_{m,n}$ |
| Acetone         | 1B <sub>2</sub>  | 2A <sub>1</sub>  | 1.005            | 0.291 | 0.916            | 0.288            | 0.979 | 0.284            | 0.934            | 0.284 | 0.934            | 0.284            |       |                  |
|                 | 1B <sub>2</sub>  | 2B <sub>2</sub>  | 1.214            | 0.298 | 0.923            | 0.294            | 1.119 | 0.304            | 0.944            | 0.290 | 0.944            | 0.290            |       |                  |
|                 | 1B <sub>2</sub>  | 2A <sub>2</sub>  | 0.979            | 0.358 | 0.842            | 0.386            | 0.934 | 0.367            | 0.857            | 0.385 | 0.857            | 0.385            |       |                  |
| Acrolein        | 1A''             | 2A''             | 2.839            | 0.107 | 2.776            | 0.089            | 2.909 | 0.106            | 2.883            | 0.099 | 2.883            | 0.099            |       |                  |
| Ammonia         | 1A <sub>2</sub>  | 1E               | 1.484            | 0.331 | 1.399            | 0.339            | 1.462 | 0.333            | 1.420            | 0.335 | 1.420            | 0.335            |       |                  |
|                 | 1A <sub>2</sub>  | 2A <sub>1</sub>  | 3.124            | 0.330 | 1.762            | 0.312            | 2.647 | 0.347            | 1.786            | 0.307 | 1.786            | 0.307            |       |                  |
|                 | 1E               | 2A <sub>2</sub>  | 2.414            | 0.259 | 0.858            | 0.168            | 1.807 | 0.248            | 0.860            | 0.159 | 0.860            | 0.159            |       |                  |
| Benzene         | 2A <sub>1</sub>  | 2A <sub>2</sub>  | 0.774            | 0.000 | 0.495            | 0.193            | 0.621 | 0.011            | 0.494            | 0.210 | 0.494            | 0.210            |       |                  |
|                 | 1E <sub>1g</sub> | 1A <sub>2u</sub> | 0.530            | 0.140 | 0.503            | 0.146            | 0.533 | 0.142            | 0.519            | 0.146 | 0.519            | 0.146            |       |                  |
|                 | 1E <sub>1g</sub> | 1E <sub>2u</sub> | 0.594            | 0.147 | 0.561            | 0.152            | 0.596 | 0.148            | 0.577            | 0.153 | 0.577            | 0.153            |       |                  |
| Butadiene       | 1B <sub>g</sub>  | 1A <sub>u</sub>  | 0.318            | 0.125 | 0.318            | 0.145            | 0.316 | 0.127            | 0.318            | 0.141 | 0.318            | 0.141            |       |                  |
|                 | 1B <sub>g</sub>  | 2A <sub>u</sub>  | 0.451            | 0.170 | 0.446            | 0.193            | 0.449 | 0.174            | 0.450            | 0.189 | 0.450            | 0.189            |       |                  |
|                 | 1A <sub>u</sub>  | 2B <sub>g</sub>  | 0.902            | 0.065 | 0.749            | 0.062            | 0.857 | 0.071            | 0.762            | 0.060 | 0.762            | 0.060            |       |                  |
| Carbon monoxide | 2A <sub>u</sub>  | 2B <sub>g</sub>  | 0.769            | 0.367 | 0.622            | 0.421            | 0.723 | 0.376            | 0.630            | 0.416 | 0.630            | 0.416            |       |                  |
|                 | 2Σ <sup>+</sup>  | 3Σ <sup>+</sup>  | 0.502            | 0.048 | 0.588            | 0.164            | 0.511 | 0.074            | 0.598            | 0.162 | 0.598            | 0.162            |       |                  |
|                 | 2Σ <sup>+</sup>  | 2Π               | 0.761            | 0.135 | 0.706            | 0.263            | 0.710 | 0.144            | 0.710            | 0.257 | 0.710            | 0.257            |       |                  |
| Cyclopentadiene | 2Π               | 1Π               | 3.264            | 0.014 | 2.795            | 0.011            | 3.344 | 0.012            | 3.059            | 0.010 | 3.059            | 0.010            |       |                  |
|                 | 2Σ <sup>+</sup>  | 1Π               | 2.503            | 0.022 | 2.090            | 0.022            | 2.633 | 0.021            | 2.349            | 0.020 | 2.349            | 0.020            |       |                  |
|                 | 3Σ <sup>+</sup>  | 1Π               | 3.005            | 0.014 | 2.678            | 0.008            | 3.144 | 0.011            | 2.947            | 0.007 | 2.947            | 0.007            |       |                  |
| Cyclopentadiene | 1B <sub>2</sub>  | 2A <sub>1</sub>  | 1.417            | 0.090 | 1.307            | 0.040            | 1.418 | 0.087            | 1.395            | 0.082 | 1.395            | 0.082            |       |                  |
|                 | 1A <sub>2</sub>  | 1B <sub>1</sub>  | 0.595            | 0.242 | 0.561            | 0.260            | 0.595 | 0.246            | 0.576            | 0.259 | 0.576            | 0.259            |       |                  |
|                 | 1A <sub>2</sub>  | 2B <sub>2</sub>  | 0.828            | 0.257 | 0.642            | 0.298            | 0.764 | 0.271            | 0.653            | 0.295 | 0.653            | 0.295            |       |                  |



| Molecule              | State1           | State2           | AVDZ             |       |       | dAVDZ            |       |       | AVTZ             |       |       | dAVTZ            |       |       |
|-----------------------|------------------|------------------|------------------|-------|-------|------------------|-------|-------|------------------|-------|-------|------------------|-------|-------|
|                       |                  |                  | $\Delta E_{m,n}$ | $f^l$ | $f^l$ | $\Delta E_{m,n}$ | $f^l$ | $f^l$ | $\Delta E_{m,n}$ | $f^l$ | $f^l$ | $\Delta E_{m,n}$ | $f^l$ | $f^l$ |
| Cyclopropene          | 1A <sub>2</sub>  | 2A <sub>2</sub>  | 0.651            | 0.270 | 0.602 | 0.284            | 0.272 | 0.616 | 0.644            | 0.272 | 0.616 | 0.282            |       |       |
|                       | 2B <sub>1</sub>  | 3B <sub>1</sub>  | 0.337            | 0.008 | 0.395 | 0.126            | 0.110 | 0.377 | 0.394            | 0.110 | 0.377 | 0.114            |       |       |
|                       | 1B <sub>1</sub>  | 2A <sub>1</sub>  | 3.470            | 0.016 | 3.309 | 0.015            | 0.015 | 3.580 | 3.664            | 0.015 | 3.580 | 0.014            |       |       |
|                       | 1B <sub>2</sub>  | 2A <sub>1</sub>  | 0.600            | 0.089 | 0.478 | 0.112            | 0.088 | 0.473 | 0.543            | 0.088 | 0.473 | 0.100            |       |       |
| Diazomethane          | 1A <sub>2</sub>  | 1B <sub>1</sub>  | 2.036            | 0.013 | 1.993 | 0.013            | 0.012 | 2.269 | 2.289            | 0.012 | 2.269 | 0.012            |       |       |
|                       | 1B <sub>2</sub>  | 2A <sub>1</sub>  | 0.989            | 0.310 | 0.918 | 0.303            | 0.303 | 0.931 | 0.965            | 0.303 | 0.931 | 0.303            |       |       |
| Formaldehyde          | 1B <sub>2</sub>  | 2A <sub>2</sub>  | 1.663            | 0.302 | 1.159 | 0.292            | 0.305 | 1.173 | 1.485            | 0.305 | 1.173 | 0.288            |       |       |
|                       | 1A <sub>2</sub>  | 1B <sub>2</sub>  | 2.355            | 0.023 | 2.343 | 0.021            | 0.021 | 2.577 | 2.583            | 0.021 | 2.577 | 0.020            |       |       |
|                       | 2B <sub>2</sub>  | 2A <sub>2</sub>  | 0.568            | 0.012 | 0.270 | 0.012            | 0.011 | 0.281 | 0.460            | 0.011 | 0.281 | 0.012            |       |       |
|                       | 1A <sub>2</sub>  | 2A <sub>2</sub>  | 4.018            | 0.022 | 3.502 | 0.016            | 0.020 | 3.750 | 4.068            | 0.020 | 3.750 | 0.015            |       |       |
| Furane                | 1A <sub>2</sub>  | 2B <sub>2</sub>  | 1.447            | 0.285 | 0.846 | 0.209            | 0.289 | 0.796 | 1.172            | 0.289 | 0.796 | 0.268            |       |       |
|                       | 1A <sub>2</sub>  | 1B <sub>1</sub>  | 0.520            | 0.230 | 0.501 | 0.237            | 0.232 | 0.514 | 0.524            | 0.232 | 0.514 | 0.235            |       |       |
|                       | 1A <sub>2</sub>  | 2A <sub>2</sub>  | 0.703            | 0.266 | 0.649 | 0.288            | 0.275 | 0.796 | 0.697            | 0.275 | 0.796 | 0.268            |       |       |
|                       | 1A <sub>u</sub>  | 1B <sub>g</sub>  | 1.448            | 0.051 | 1.446 | 0.051            | 0.051 | 1.443 | 1.443            | 0.051 | 1.443 | 0.051            |       |       |
| Glyoxal               | 1A <sub>u</sub>  | 2B <sub>g</sub>  | 3.640            | 0.221 | 3.593 | 0.208            | 0.219 | 3.648 | 3.665            | 0.219 | 3.648 | 0.214            |       |       |
|                       | 1B <sub>1</sub>  | 2A <sub>2</sub>  | 1.158            | 0.354 | 1.079 | 0.352            | 0.352 | 1.110 | 1.155            | 0.352 | 1.110 | 0.350            |       |       |
| Ketene                | 1B <sub>1</sub>  | 2A <sub>1</sub>  | 1.407            | 0.151 | 1.094 | 0.226            | 0.142 | 1.075 | 1.238            | 0.142 | 1.075 | 0.190            |       |       |
|                       | 1B <sub>1</sub>  | 1A <sub>2</sub>  | 0.500            | 0.196 | 0.479 | 0.212            | 0.197 | 0.485 | 0.495            | 0.197 | 0.485 | 0.208            |       |       |
| Methylenecyclopropene | 1B <sub>2</sub>  | 1A <sub>2</sub>  | 1.245            | 0.024 | 1.175 | 0.025            | 0.023 | 1.379 | 1.412            | 0.023 | 1.379 | 0.024            |       |       |
|                       | 2A <sub>g</sub>  | 2B <sub>1u</sub> | 0.903            | 0.102 | 0.708 | 0.226            | 0.220 | 0.765 | 0.808            | 0.220 | 0.765 | 0.227            |       |       |
| Pyrazine              | 2A <sub>g</sub>  | 2B <sub>2u</sub> | 0.532            | 0.284 | 0.515 | 0.281            | 0.283 | 0.526 | 0.538            | 0.283 | 0.526 | 0.280            |       |       |
|                       | 1B <sub>1u</sub> | 1B <sub>3g</sub> | 0.528            | 0.166 | 0.271 | 0.017            | 0.028 | 0.613 | 0.694            | 0.028 | 0.613 | 0.044            |       |       |
|                       | 2B <sub>2u</sub> | 1B <sub>3g</sub> | 0.758            | 0.207 | 0.678 | 0.241            | 0.214 | 0.685 | 0.733            | 0.214 | 0.685 | 0.239            |       |       |
|                       | 1A <sub>2</sub>  | 2B <sub>1</sub>  | 2.102            | 0.025 | 2.101 | 0.024            | 0.024 | 2.073 | 2.074            | 0.024 | 2.073 | 0.024            |       |       |
| Pyridazine            | 1A <sub>2</sub>  | 1B <sub>1</sub>  | 0.626            | 0.015 | 0.622 | 0.033            | 0.003 | 0.642 | 0.622            | 0.003 | 0.642 | 0.037            |       |       |
|                       | 1A <sub>2</sub>  | 2A <sub>2</sub>  | 0.742            | 0.188 | 0.687 | 0.199            | 0.191 | 0.699 | 0.730            | 0.191 | 0.699 | 0.198            |       |       |

| Molecule   | State1           | State2           | AVDZ             |       |                  | dAVDZ            |       |                  | AVTZ             |       |                  | dAVTZ            |       |                  |
|------------|------------------|------------------|------------------|-------|------------------|------------------|-------|------------------|------------------|-------|------------------|------------------|-------|------------------|
|            |                  |                  | $\Delta E_{m,n}$ | $f^l$ | $\Delta E_{m,n}$ | $\Delta E_{m,n}$ | $f^l$ | $\Delta E_{m,n}$ | $\Delta E_{m,n}$ | $f^l$ | $\Delta E_{m,n}$ | $\Delta E_{m,n}$ | $f^l$ | $\Delta E_{m,n}$ |
| Silylidene | 1A <sub>2</sub>  | 1B <sub>2</sub>  | 1.508            | 0.004 | 1.508            | 1.508            | 0.004 | 1.515            | 1.514            | 0.004 | 1.514            | 1.514            | 0.004 | 0.004            |
| Tetrazine  | 1B <sub>3u</sub> | 1B <sub>1g</sub> | 2.660            | 0.158 | 2.659            | 2.659            | 0.158 | 2.621            | 2.621            | 0.154 | 2.621            | 2.621            | 0.154 | 0.154            |
|            | 1B <sub>3u</sub> | 1B <sub>2g</sub> | 3.295            | 0.057 | 3.294            | 3.294            | 0.057 | 3.254            | 3.255            | 0.056 | 3.255            | 3.255            | 0.056 | 0.056            |
| Thiophene  | 1A <sub>2</sub>  | 1B <sub>1</sub>  | 0.210            | 0.052 | 0.234            | 0.234            | 0.066 | 0.097            | 0.112            | 0.015 | 0.112            | 0.112            | 0.019 | 0.019            |
| Water      | 1B <sub>1</sub>  | 1A <sub>2</sub>  | 1.655            | 0.324 | 1.627            | 1.627            | 0.321 | 1.657            | 1.643            | 0.321 | 1.643            | 1.643            | 0.316 | 0.316            |

### S3.5 Full testing set ISR-ADC(3), EOM-CCSD, QR-TDDFT and QR-TDA (dAVTZ)

Table S33: Excited State absorption data for ISR-ADC(3), B3LYP (full TDDFT), and CAM-B3LYP (full TDDFT).  $\Delta E_{m,n}$  [eV] and oscillator strengths in length, velocity gauges,  $f^l$ ,  $f^v$  respectively. All data are obtained with dAVTZ basis set.

| Molecule        | State1           | State2           | ISR-ADC(3)       |       |                  |       | B3LYP            |       |       |                  | CAMB3LYP |       |  |  |
|-----------------|------------------|------------------|------------------|-------|------------------|-------|------------------|-------|-------|------------------|----------|-------|--|--|
|                 |                  |                  | $\Delta E_{m,n}$ | $f^l$ | $\Delta E_{m,n}$ | $f^l$ | $\Delta E_{m,n}$ | $f^l$ | $f^v$ | $\Delta E_{m,n}$ | $f^l$    | $f^v$ |  |  |
| Acetone         | 1B <sub>2</sub>  | 2A <sub>1</sub>  | 0.985            | 0.255 | 0.738            | 0.273 | 0.272            | 0.273 | 0.272 | 0.920            | 0.262    | 0.263 |  |  |
|                 | 1B <sub>2</sub>  | 2B <sub>2</sub>  | 0.981            | 0.277 | 0.878            | 0.257 | 0.256            | 0.257 | 0.256 | 0.946            | 0.269    | 0.271 |  |  |
|                 | 1B <sub>2</sub>  | 2A <sub>2</sub>  | 0.922            | 0.370 | 0.820            | 0.331 | 0.332            | 0.331 | 0.332 | 0.898            | 0.349    | 0.355 |  |  |
| Acrolein        | 1A''             | 2A''             | 3.057            | 0.004 | 2.832            | 0.054 | 0.053            | 0.054 | 0.053 | 3.194            | 0.039    | 0.047 |  |  |
| Ammonia         | 1A <sub>2</sub>  | 1E               | 1.560            | 0.317 | 1.096            | 0.567 | 0.629            | 0.567 | 0.629 | 1.357            | 0.305    | 0.313 |  |  |
|                 | 1A <sub>2</sub>  | 2A <sub>1</sub>  | 2.031            | 0.293 | 1.382            | 0.137 | 0.127            | 0.137 | 0.127 | 1.747            | 0.266    | 0.274 |  |  |
|                 | 1E               | 2A <sub>2</sub>  | 1.019            | 0.135 | 0.324            | 0.216 | 0.219            | 0.216 | 0.219 | 0.717            | 0.153    | 0.157 |  |  |
| Benzene         | 2A <sub>1</sub>  | 2A <sub>2</sub>  | 0.548            | 0.252 | 0.037            | 0.001 | 1.495            | 0.001 | 1.495 | 0.327            | 0.153    | 0.270 |  |  |
|                 | 1E <sub>1g</sub> | 1A <sub>2u</sub> | 0.529            | 0.131 | 0.458            | 0.142 | 0.142            | 0.142 | 0.142 | 0.480            | 0.106    | 0.126 |  |  |
|                 | 1E <sub>1g</sub> | 1E <sub>2u</sub> | 0.609            | 0.140 | 0.480            | 0.144 | 0.144            | 0.144 | 0.144 | 0.575            | 0.130    | 0.139 |  |  |
| Butadiene       | 1B <sub>g</sub>  | 1A <sub>u</sub>  | 0.319            | 0.126 | 0.259            | 0.133 | 0.134            | 0.133 | 0.134 | 0.279            | 0.140    | 0.116 |  |  |
|                 | 1B <sub>g</sub>  | 2A <sub>u</sub>  | 0.470            | 0.162 | 0.317            | 0.195 | 0.195            | 0.195 | 0.195 | 0.427            | 0.126    | 0.172 |  |  |
|                 | 1A <sub>u</sub>  | 2B <sub>g</sub>  | 0.821            | 0.058 | 0.551            | 0.023 | 0.025            | 0.023 | 0.025 | 0.774            | 0.181    | 0.057 |  |  |
| Carbon monoxide | 2A <sub>u</sub>  | 2B <sub>g</sub>  | 0.670            | 0.368 | 0.493            | 0.405 | 0.401            | 0.405 | 0.401 | 0.627            | 0.047    | 0.391 |  |  |
|                 | 2Σ <sup>+</sup>  | 3Σ <sup>+</sup>  | 0.608            | 0.147 | 0.338            | 0.170 | 0.205            | 0.170 | 0.205 | 0.440            | 0.158    | 0.158 |  |  |
|                 | 2Σ <sup>+</sup>  | 2Π               | 0.753            | 0.262 | 0.395            | 0.415 | 0.702            | 0.415 | 0.702 | 0.539            | 0.538    | 0.523 |  |  |
| Cyclopentadiene | 2Π               | 1Π               | 3.044            | 0.011 | 1.868            | 0.006 | 0.006            | 0.006 | 0.006 | 2.502            | 0.011    | 0.010 |  |  |
|                 | 2Σ <sup>+</sup>  | 1Π               | 2.291            | 0.028 | 1.473            | 0.035 | 0.035            | 0.035 | 0.035 | 1.963            | 0.040    | 0.047 |  |  |
|                 | 3Σ <sup>+</sup>  | 1Π               | 2.899            | 0.009 | 1.811            | 0.012 | 0.012            | 0.012 | 0.012 | 2.403            | 0.009    | 0.009 |  |  |
| Cyclopentadiene | 1B <sub>2</sub>  | 2A <sub>1</sub>  | 0.577            | 0.001 | 1.221            | 0.002 | 0.002            | 0.002 | 0.002 | 1.700            | 0.005    | 0.039 |  |  |
|                 | 1A <sub>2</sub>  | 1B <sub>1</sub>  | 0.605            | 0.234 | 0.491            | 0.270 | 0.270            | 0.270 | 0.270 | 0.565            | 0.251    | 0.241 |  |  |
|                 | 1A <sub>2</sub>  | 2B <sub>2</sub>  | 0.683            | 0.287 | 0.603            | 0.288 | 0.287            | 0.288 | 0.287 | 0.658            | 0.287    | 0.283 |  |  |

| Molecule              | State1           | State2           | ISR-ADC(3)       |       |       |                  | B3LYP |       |                  |       | CAMB3LYP |                  |       |       |
|-----------------------|------------------|------------------|------------------|-------|-------|------------------|-------|-------|------------------|-------|----------|------------------|-------|-------|
|                       |                  |                  | $\Delta E_{m,n}$ | $f^l$ | $f^v$ | $\Delta E_{m,n}$ | $f^l$ | $f^v$ | $\Delta E_{m,n}$ | $f^l$ | $f^v$    | $\Delta E_{m,n}$ | $f^l$ | $f^v$ |
| Cyclopropene          | 1A <sub>2</sub>  | 2A <sub>2</sub>  | 0.657            | 0.257 | 0.501 | 0.270            | 0.270 | 0.270 | 0.623            | 0.267 | 0.259    |                  |       |       |
|                       | 2B <sub>1</sub>  | 3B <sub>1</sub>  | 0.370            | 0.104 | 0.334 | 0.092            | 0.091 | 0.091 | 0.353            | 0.128 | 0.107    |                  |       |       |
|                       | 1B <sub>1</sub>  | 2A <sub>1</sub>  | 4.081            | 0.014 | 3.380 | 0.010            | 0.010 | 0.010 | 3.809            | 0.014 | 0.015    |                  |       |       |
|                       | 1B <sub>2</sub>  | 2A <sub>1</sub>  | 0.569            | 0.083 | 0.556 | 0.153            | 0.149 | 0.149 | 0.581            | 0.081 | 0.080    |                  |       |       |
| Diazomethane          | 1A <sub>2</sub>  | 1B <sub>1</sub>  | 2.471            | 0.012 | 2.087 | 0.015            | 0.015 | 0.015 | 2.349            | 0.013 | 0.014    |                  |       |       |
|                       | 1B <sub>2</sub>  | 2A <sub>1</sub>  | 0.950            | 0.310 | 0.707 | 0.304            | 0.305 | 0.305 | 0.841            | 0.306 | 0.304    |                  |       |       |
| Formaldehyde          | 1B <sub>2</sub>  | 2A <sub>2</sub>  | 1.151            | 0.292 | 0.902 | 0.284            | 0.272 | 0.272 | 1.044            | 0.293 | 0.289    |                  |       |       |
|                       | 1A <sub>2</sub>  | 1B <sub>2</sub>  | 3.711            | 0.021 | 2.497 | 0.020            | 0.020 | 0.020 | 2.957            | 0.026 | 0.021    |                  |       |       |
|                       | 2B <sub>2</sub>  | 2A <sub>2</sub>  | 0.402            | 0.006 | 0.168 | 0.012            | 0.014 | 0.014 | 0.304            | 0.011 | 0.010    |                  |       |       |
|                       | 1A <sub>2</sub>  | 2A <sub>2</sub>  | 4.863            | 0.012 | 3.399 | 0.008            | 0.008 | 0.008 | 4.002            | 0.009 | 0.011    |                  |       |       |
| Furane                | 1A <sub>2</sub>  | 2B <sub>2</sub>  | 0.808            | 0.280 | 0.778 | 0.220            | 0.210 | 0.210 | 0.788            | 0.284 | 0.280    |                  |       |       |
|                       | 1A <sub>2</sub>  | 1B <sub>1</sub>  | 0.537            | 0.218 | 0.417 | 0.260            | 0.261 | 0.261 | 0.492            | 0.238 | 0.225    |                  |       |       |
|                       | 1A <sub>2</sub>  | 2A <sub>2</sub>  | 0.696            | 0.273 | 0.530 | 0.282            | 0.282 | 0.282 | 0.662            | 0.279 | 0.274    |                  |       |       |
|                       | 1A <sub>u</sub>  | 1B <sub>g</sub>  | 1.400            | 0.016 | 1.513 | 0.037            | 0.036 | 0.036 | 1.507            | 0.026 | 0.026    |                  |       |       |
| Glyoxal               | 1A <sub>u</sub>  | 2B <sub>g</sub>  | 3.966            | 0.039 | 3.407 | 0.096            | 0.095 | 0.095 | 3.800            | 0.138 | 0.124    |                  |       |       |
|                       | 1B <sub>1</sub>  | 2A <sub>2</sub>  | 1.154            | 0.340 | 0.844 | 0.315            | 0.313 | 0.313 | 1.026            | 0.324 | 0.327    |                  |       |       |
| Ketene                | 1B <sub>1</sub>  | 2A <sub>1</sub>  | 1.142            | 0.174 | 0.933 | 0.275            | 0.269 | 0.269 | 1.095            | 0.227 | 0.220    |                  |       |       |
|                       | 1B <sub>1</sub>  | 1A <sub>2</sub>  | 0.513            | 0.198 | 0.382 | 0.212            | 0.213 | 0.213 | 0.479            | 0.217 | 0.200    |                  |       |       |
| Methylenecyclopropene | 1B <sub>2</sub>  | 1A <sub>2</sub>  | 1.572            | 0.024 | 1.224 | 0.018            | 0.018 | 0.018 | 1.309            | 0.023 | 0.023    |                  |       |       |
|                       | 2A <sub>g</sub>  | 2B <sub>1u</sub> | 0.628            | 0.113 | 0.640 | 0.259            | 0.259 | 0.259 | 0.662            | 0.098 | 0.180    |                  |       |       |
| Pyrazine              | 2A <sub>g</sub>  | 2B <sub>2u</sub> | 0.610            | 0.250 | 0.395 | 0.253            | 0.254 | 0.254 | 0.552            | 0.244 | 0.243    |                  |       |       |
|                       | 1B <sub>1u</sub> | 1B <sub>3g</sub> | 1.570            | 0.003 | 0.568 | 0.008            | 0.008 | 0.008 | 1.348            | 0.001 | 0.003    |                  |       |       |
|                       | 2B <sub>2u</sub> | 1B <sub>3g</sub> | 0.677            | 0.188 | 0.555 | 0.220            | 0.219 | 0.219 | 0.648            | 0.220 | 0.201    |                  |       |       |
|                       | 1A <sub>2</sub>  | 2B <sub>1</sub>  | 2.014            | 0.013 | 1.990 | 0.010            | 0.009 | 0.009 | 1.983            | 0.003 | 0.006    |                  |       |       |
| Pyrrolone             | 1A <sub>2</sub>  | 1B <sub>1</sub>  | 0.736            | 0.151 | 0.662 | 0.227            | 0.227 | 0.227 | 0.706            | 0.225 | 0.190    |                  |       |       |
|                       | 1A <sub>2</sub>  | 2A <sub>2</sub>  | 0.745            | 0.177 | 0.660 | 0.165            | 0.165 | 0.165 | 0.726            | 0.183 | 0.174    |                  |       |       |

| Molecule   | State1           | State2           | ISR-ADC(3)       |       |       | B3LYP            |       |       | CAMB3LYP         |       |       |
|------------|------------------|------------------|------------------|-------|-------|------------------|-------|-------|------------------|-------|-------|
|            |                  |                  | $\Delta E_{m,n}$ | $f^l$ | $f^v$ | $\Delta E_{m,n}$ | $f^l$ | $f^v$ | $\Delta E_{m,n}$ | $f^l$ | $f^v$ |
| Silylidene | 1A <sub>2</sub>  | 1B <sub>2</sub>  | 1.514            | 0.004 | 0.004 | 1.614            | 0.003 | 0.002 | 1.580            | 0.003 | 0.002 |
| Tetrazine  | 1B <sub>3u</sub> | 1B <sub>1g</sub> | 2.555            | 0.073 |       | 2.484            | 0.054 | 0.054 | 2.552            | 0.049 | 0.054 |
|            | 1B <sub>3u</sub> | 1B <sub>2g</sub> | 2.718            | 0.012 |       | 2.552            | 0.054 | 0.054 | 3.300            | 0.025 | 0.024 |
| Thiophene  | 1A <sub>2</sub>  | 1B <sub>1</sub>  | 0.010            | 0.001 |       | 0.151            | 0.035 | 0.035 | 0.134            | 0.036 | 0.021 |
| Water      | 1B <sub>1</sub>  | 1A <sub>2</sub>  | 1.782            | 0.267 |       | 1.336            | 0.281 | 0.279 | 1.558            | 0.266 | 0.287 |

Table S34: Excited State absorption data for LC-BLYP33 (full TDDFT), and LC-BLYP47 (full TDDFT).  $\Delta E_{m,n}$ [eV] and oscillator strengths in length and velocity gauges,  $f^l$ ,  $f^v$  respectively. All data are obtained with dAVTZ basis set.

| Molecule        | State1           | State2           | LC-BLYP33        |       |       | LC-BLYP47        |       |       |
|-----------------|------------------|------------------|------------------|-------|-------|------------------|-------|-------|
|                 |                  |                  | $\Delta E_{m,n}$ | $f^l$ | $f^v$ | $\Delta E_{m,n}$ | $f^l$ | $f^v$ |
| Acetone         | 1B <sub>2</sub>  | 2A <sub>1</sub>  | 1.075            | 0.247 | 0.247 | 1.107            | 0.262 | 0.234 |
|                 | 1B <sub>2</sub>  | 2B <sub>2</sub>  | 1.039            | 0.258 | 0.258 | 1.064            | 0.269 | 0.253 |
|                 | 1B <sub>2</sub>  | 2A <sub>2</sub>  | 0.940            | 0.349 | 0.350 | 0.962            | 0.349 | 0.348 |
| Acrolein        | 1A''             | 2A''             | 3.183            | 0.042 | 0.041 | 3.597            | 0.039 | 0.023 |
| Ammonia         | 1A <sub>2</sub>  | 1E               | 1.442            | 0.314 | 0.315 | 1.540            | 0.305 | 0.305 |
|                 | 1A <sub>2</sub>  | 2A <sub>1</sub>  | 1.916            | 0.275 | 0.276 | 2.053            | 0.266 | 0.273 |
|                 | 1E               | 2A <sub>2</sub>  | 0.987            | 0.126 | 0.131 | 1.082            | 0.153 | 0.116 |
| Benzene         | 2A <sub>1</sub>  | 2A <sub>2</sub>  | 0.987            | 0.126 | 0.131 | 1.082            | 0.153 | 0.116 |
|                 | 1E <sub>1g</sub> | 1A <sub>2u</sub> | 0.514            | 0.253 | 0.272 | 0.568            | 0.106 | 0.275 |
|                 | 1E <sub>1g</sub> | 1E <sub>2u</sub> | 0.496            | 0.115 | 0.115 | 0.481            | 0.130 | 0.111 |
| Butadiene       | 1B <sub>g</sub>  | 1A <sub>u</sub>  | 0.647            | 0.134 | 0.134 | 0.667            | 0.140 | 0.134 |
|                 | 1B <sub>g</sub>  | 2A <sub>u</sub>  | 0.295            | 0.107 | 0.108 | 0.311            | 0.126 | 0.110 |
|                 | 1A <sub>u</sub>  | 2B <sub>g</sub>  | 0.501            | 0.155 | 0.155 | 0.519            | 0.181 | 0.152 |
| Carbon monoxide | 2A <sub>u</sub>  | 2B <sub>g</sub>  | 0.876            | 0.091 | 0.091 | 0.888            | 0.047 | 0.143 |
|                 | 2Σ <sup>+</sup>  | 3Σ <sup>+</sup>  | 0.460            | 0.129 | 0.128 | 0.508            | 0.158 | 0.122 |
|                 | 2Σ <sup>+</sup>  | 2Π               | 0.581            | 0.434 | 0.432 | 0.627            | 0.538 | 0.413 |
|                 | 2Π               | 1Π               | 2.480            | 0.013 | 0.012 | 3.211            | 0.011 | 0.015 |
|                 | 2Σ <sup>+</sup>  | 1Π               | 1.898            | 0.058 | 0.058 | 2.584            | 0.040 | 0.052 |
|                 | 3Σ <sup>+</sup>  | 1Π               | 2.359            | 0.008 | 0.007 | 3.092            | 0.009 | 0.005 |
| Cyclopentadiene | 1B <sub>2</sub>  | 2A <sub>1</sub>  | 1.750            | 0.055 | 0.054 | 2.124            | 0.005 | 0.069 |
|                 | 1A <sub>2</sub>  | 1B <sub>1</sub>  | 0.613            | 0.218 | 0.218 | 0.613            | 0.251 | 0.215 |
|                 | 1A <sub>2</sub>  | 2B <sub>2</sub>  | 0.678            | 0.277 | 0.277 | 0.687            | 0.287 | 0.278 |

| Molecule              | State1           | State2           | LC-BLYP33        |       |       |                  | LC-BLYP47 |       |                  |       |
|-----------------------|------------------|------------------|------------------|-------|-------|------------------|-----------|-------|------------------|-------|
|                       |                  |                  | $\Delta E_{m,n}$ | $f^l$ | $f^v$ | $\Delta E_{m,n}$ | $f^l$     | $f^v$ | $\Delta E_{m,n}$ | $f^l$ |
| Cyclopropene          | 1A <sub>2</sub>  | 2A <sub>2</sub>  | 0.713            | 0.245 | 0.245 | 0.747            | 0.267     | 0.244 |                  |       |
|                       | 2B <sub>1</sub>  | 3B <sub>1</sub>  | 0.380            | 0.104 | 0.104 | 0.378            | 0.128     | 0.096 |                  |       |
| Diazirine             | 1B <sub>1</sub>  | 2A <sub>1</sub>  | 3.829            | 0.040 | 0.042 | 4.316            | 0.014     | 0.014 |                  |       |
|                       | 1B <sub>2</sub>  | 2A <sub>1</sub>  | 0.575            | 0.053 | 0.053 | 0.697            | 0.081     | 0.022 |                  |       |
| Diazomethane          | 1A <sub>2</sub>  | 1B <sub>1</sub>  | 2.329            | 0.014 | 0.014 | 2.742            | 0.013     | 0.013 |                  |       |
|                       | 1B <sub>2</sub>  | 2A <sub>1</sub>  | 0.891            | 0.291 | 0.293 | 0.938            | 0.306     | 0.290 |                  |       |
| Formaldehyde          | 1B <sub>2</sub>  | 2A <sub>2</sub>  | 1.062            | 0.287 | 0.287 | 1.137            | 0.293     | 0.284 |                  |       |
|                       | 1A <sub>2</sub>  | 1B <sub>2</sub>  | 2.889            | 0.017 | 0.017 | 3.504            | 0.026     | 0.018 |                  |       |
| Furane                | 2B <sub>2</sub>  | 2A <sub>2</sub>  | 0.297            | 0.004 | 0.004 | 0.363            | 0.011     | 0.003 |                  |       |
|                       | 1A <sub>2</sub>  | 2A <sub>2</sub>  | 3.951            | 0.013 | 0.013 | 4.641            | 0.009     | 0.013 |                  |       |
| Glyoxal               | 1A <sub>2</sub>  | 2B <sub>2</sub>  | 0.815            | 0.283 | 0.283 | 0.803            | 0.284     | 0.291 |                  |       |
|                       | 1A <sub>2</sub>  | 1B <sub>1</sub>  | 0.536            | 0.197 | 0.197 | 0.545            | 0.238     | 0.192 |                  |       |
| Ketene                | 1A <sub>2</sub>  | 2A <sub>2</sub>  | 0.750            | 0.265 | 0.265 | 0.792            | 0.279     | 0.263 |                  |       |
|                       | 1A <sub>u</sub>  | 1B <sub>g</sub>  | 1.499            | 0.022 | 0.022 | 1.465            | 0.026     | 0.017 |                  |       |
| Methylenecyclopropene | 1A <sub>u</sub>  | 2B <sub>g</sub>  | 3.743            | 0.129 | 0.128 | 4.362            | 0.138     | 0.149 |                  |       |
|                       | 1B <sub>1</sub>  | 2A <sub>2</sub>  | 1.101            | 0.326 | 0.327 | 1.171            | 0.324     | 0.323 |                  |       |
| Pyrazine              | 1B <sub>1</sub>  | 2A <sub>1</sub>  | 1.155            | 0.192 | 0.191 | 1.076            | 0.227     | 0.112 |                  |       |
|                       | 1B <sub>1</sub>  | 1A <sub>2</sub>  | 0.547            | 0.199 | 0.199 | 0.584            | 0.217     | 0.202 |                  |       |
| Pyradazine            | 1B <sub>2</sub>  | 1A <sub>2</sub>  | 1.377            | 0.024 | 0.024 | 1.362            | 0.023     | 0.025 |                  |       |
|                       | 2A <sub>g</sub>  | 2B <sub>1u</sub> | 0.660            | 0.139 | 0.139 | 0.804            | 0.098     | 0.127 |                  |       |
| Pyrrole               | 2A <sub>g</sub>  | 2B <sub>2u</sub> | 0.687            | 0.231 | 0.231 | 0.728            | 0.244     | 0.228 |                  |       |
|                       | 1B <sub>1u</sub> | 1B <sub>3g</sub> | 1.336            | 0.005 | 0.005 | 2.148            | 0.001     | 0.002 |                  |       |
| Pyrrolone             | 2B <sub>2u</sub> | 1B <sub>3g</sub> | 0.626            | 0.159 | 0.159 | 0.624            | 0.220     | 0.160 |                  |       |
|                       | 1A <sub>2</sub>  | 2B <sub>1</sub>  | 1.978            | 0.008 | 0.007 | 1.997            | 0.003     | 0.004 |                  |       |
| Pyrrole               | 1A <sub>2</sub>  | 1B <sub>1</sub>  | 0.722            | 0.143 | 0.142 | 0.704            | 0.225     | 0.167 |                  |       |
|                       | 1A <sub>2</sub>  | 2A <sub>2</sub>  | 0.763            | 0.171 | 0.171 | 0.757            | 0.183     | 0.185 |                  |       |



| Molecule   | State1           | State2           | LC-BLYP33        |       |       |                  | LC-BLYP47 |       |       |       |
|------------|------------------|------------------|------------------|-------|-------|------------------|-----------|-------|-------|-------|
|            |                  |                  | $\Delta E_{m,n}$ | $f^l$ | $f^v$ | $\Delta E_{m,n}$ | $f^l$     | $f^v$ | $f^l$ | $f^v$ |
| Silylidene | 1A <sub>2</sub>  | 1B <sub>2</sub>  | 1.458            | 0.002 | 0.002 | 1.480            | 0.003     | 0.002 | 0.003 | 0.002 |
| Tetrazine  | 1B <sub>3u</sub> | 1B <sub>1g</sub> | 2.509            | 0.058 | 0.058 | 2.546            | 0.049     | 0.057 | 0.049 | 0.057 |
|            | 1B <sub>3u</sub> | 1B <sub>2g</sub> | 3.345            | 0.027 | 0.026 | 3.411            | 0.025     | 0.026 | 0.025 | 0.026 |
| Thiophene  | 1A <sub>2</sub>  | 1B <sub>1</sub>  | 0.143            | 0.016 | 0.016 | 0.301            | 0.036     | 0.000 | 0.036 | 0.000 |
| Water      | 1B <sub>1</sub>  | 1A <sub>2</sub>  | 1.624            | 0.289 | 0.290 | 1.734            | 0.266     | 0.270 | 0.266 | 0.270 |

Table S35: Excited State absorption data for BHandHLYP (full TDDFT), BHandHLYP (TDA) and EOM-CCSD.  $\Delta E_{m,n}$  [eV] and oscillator strengths in length, and velocity gauges,  $f^l$ ,  $f^v$  respectively. All data are obtained with dAVTZ basis set.

| Molecule        | State1           | State2           | BHandHLYP        |       |       |                  | BHandHLYP (TDA) |       |                  |       | EOM-CCSD         |       |
|-----------------|------------------|------------------|------------------|-------|-------|------------------|-----------------|-------|------------------|-------|------------------|-------|
|                 |                  |                  | $\Delta E_{m,n}$ | $f^l$ | $f^v$ | $\Delta E_{m,n}$ | $f^l$           | $f^v$ | $\Delta E_{m,n}$ | $f^v$ | $\Delta E_{m,n}$ | $f^v$ |
| Acetone         | 1B <sub>2</sub>  | 2A <sub>1</sub>  | 0.853            | 0.262 | 0.262 | 0.858            | 0.304           | 0.294 | 1.011            | 0.270 |                  |       |
|                 | 1B <sub>2</sub>  | 2B <sub>2</sub>  | 0.913            | 0.269 | 0.269 | 0.912            | 0.310           | 0.305 | 0.989            | 0.283 |                  |       |
|                 | 1B <sub>2</sub>  | 2A <sub>2</sub>  | 0.869            | 0.349 | 0.349 | 0.867            | 0.404           | 0.385 | 0.910            | 0.377 |                  |       |
| Acrolein        | 1A''             | 2A''             | 3.500            | 0.039 | 0.039 | 3.459            | 0.081           | 0.052 | 3.343            | 0.061 |                  |       |
| Ammonia         | 1A <sub>2</sub>  | 1E               | 1.342            | 0.305 | 0.306 | 1.333            | 0.330           | 0.358 | 1.520            | 0.327 |                  |       |
|                 | 1A <sub>2</sub>  | 2A <sub>1</sub>  | 1.724            | 0.266 | 0.266 | 1.730            | 0.285           | 0.255 | 1.965            | 0.300 |                  |       |
|                 | 1E               | 2A <sub>2</sub>  | 0.608            | 0.153 | 0.157 | 0.604            | 0.149           | 0.158 | 0.989            | 0.142 |                  |       |
| Benzene         | 2A <sub>1</sub>  | 2A <sub>2</sub>  | 0.608            | 0.153 | 0.157 | 0.207            | 0.101           | 0.321 | 0.543            | 0.243 |                  |       |
|                 | 1E <sub>1g</sub> | 1A <sub>2u</sub> | 0.227            | 0.106 | 0.310 | 0.461            | 0.152           | 0.110 | 0.530            | 0.138 |                  |       |
|                 | 1E <sub>1g</sub> | 1E <sub>2u</sub> | 0.459            | 0.130 | 0.130 | 0.543            | 0.171           | 0.220 | 0.606            | 0.146 |                  |       |
|                 | 1B <sub>g</sub>  | 1A <sub>u</sub>  | 0.544            | 0.140 | 0.140 | 0.283            | 0.147           | 0.164 | 0.317            | 0.130 |                  |       |
| Butadiene       | 1B <sub>g</sub>  | 2A <sub>u</sub>  | 0.284            | 0.126 | 0.126 | 0.394            | 0.207           | 0.214 | 0.476            | 0.173 |                  |       |
|                 | 1A <sub>u</sub>  | 2B <sub>g</sub>  | 0.394            | 0.181 | 0.181 | 0.705            | 0.053           | 0.055 | 0.813            | 0.059 |                  |       |
|                 | 2A <sub>u</sub>  | 2B <sub>g</sub>  | 0.706            | 0.047 | 0.047 | 0.594            | 0.440           | 0.445 | 0.654            | 0.384 |                  |       |
|                 | 2Σ <sup>+</sup>  | 3Σ <sup>+</sup>  | 0.448            | 0.158 | 0.169 | 0.426            | 0.175           | 0.264 | 0.606            | 0.145 |                  |       |
|                 | 2Σ <sup>+</sup>  | 2Π               | 0.534            | 0.538 | 0.635 | 0.514            | 0.487           | 0.693 | 0.740            | 0.255 |                  |       |
|                 | 2Π               | 1Π               | 2.885            | 0.011 | 0.010 | 2.664            | 0.008           | 0.010 | 3.119            | 0.010 |                  |       |
|                 | 2Σ <sup>+</sup>  | 1Π               | 2.351            | 0.040 | 0.041 | 2.150            | 0.043           | 0.028 | 2.379            | 0.024 |                  |       |
| Carbon monoxide | 3Σ <sup>+</sup>  | 1Π               | 2.798            | 0.009 | 0.008 | 2.576            | 0.006           | 0.005 | 2.985            | 0.008 |                  |       |
|                 | 1B <sub>2</sub>  | 2A <sub>1</sub>  | 1.626            | 0.005 | 0.005 | 1.306            | 0.007           | 0.009 | 1.284            | 0.055 |                  |       |
|                 | 1A <sub>2</sub>  | 1B <sub>1</sub>  | 0.531            | 0.251 | 0.251 | 0.532            | 0.284           | 0.284 | 0.600            | 0.244 |                  |       |
|                 | 1A <sub>2</sub>  | 2B <sub>2</sub>  | 0.645            | 0.287 | 0.288 | 0.647            | 0.322           | 0.309 | 0.673            | 0.290 |                  |       |
|                 |                  |                  |                  |       |       |                  |                 |       |                  |       |                  |       |
| Cyclopentadiene |                  |                  |                  |       |       |                  |                 |       |                  |       |                  |       |
|                 |                  |                  |                  |       |       |                  |                 |       |                  |       |                  |       |
|                 |                  |                  |                  |       |       |                  |                 |       |                  |       |                  |       |

| Molecule              | State1           | State2           | BHandHLYP        |       |       |                  | BHandHLYP (TDA) |       |                  |       | EOM-CCSD |  |
|-----------------------|------------------|------------------|------------------|-------|-------|------------------|-----------------|-------|------------------|-------|----------|--|
|                       |                  |                  | $\Delta E_{m,n}$ | $f^l$ | $f^v$ | $\Delta E_{m,n}$ | $f^l$           | $f^v$ | $\Delta E_{m,n}$ | $f^v$ |          |  |
| Cyclopropene          | 1A <sub>2</sub>  | 2A <sub>2</sub>  | 0.584            | 0.267 | 0.267 | 0.583            | 0.323           | 0.318 | 0.647            | 0.268 |          |  |
|                       | 2B <sub>1</sub>  | 3B <sub>1</sub>  | 0.351            | 0.128 | 0.127 | 0.354            | 0.144           | 0.146 | 0.377            | 0.109 |          |  |
|                       | 1B <sub>1</sub>  | 2A <sub>1</sub>  | 3.988            | 0.014 | 0.015 | 3.943            | 0.013           | 0.014 | 3.864            | 0.015 |          |  |
|                       | 1B <sub>2</sub>  | 2A <sub>1</sub>  | 0.622            | 0.081 | 0.080 | 0.591            | 0.129           | 0.107 | 0.503            | 0.091 |          |  |
| Diazomethane          | 1A <sub>2</sub>  | 1B <sub>1</sub>  | 2.469            | 0.013 | 0.013 | 2.397            | 0.013           | 0.009 | 2.364            | 0.012 |          |  |
|                       | 1B <sub>2</sub>  | 2A <sub>1</sub>  | 0.839            | 0.306 | 0.309 | 0.840            | 0.332           | 0.326 | 0.945            | 0.305 |          |  |
| Formaldehyde          | 1B <sub>2</sub>  | 2A <sub>2</sub>  | 1.054            | 0.293 | 0.292 | 1.049            | 0.307           | 0.301 | 1.168            | 0.290 |          |  |
|                       | 1A <sub>2</sub>  | 1B <sub>2</sub>  | 3.334            | 0.026 | 0.026 | 3.278            | 0.024           | 0.016 | 3.214            | 0.020 |          |  |
|                       | 2B <sub>2</sub>  | 2A <sub>2</sub>  | 0.318            | 0.011 | 0.012 | 0.313            | 0.010           | 0.012 | 0.366            | 0.008 |          |  |
|                       | 1A <sub>2</sub>  | 2A <sub>2</sub>  | 4.388            | 0.009 | 0.009 | 4.327            | 0.010           | 0.011 | 4.382            | 0.014 |          |  |
| Furane                | 1A <sub>2</sub>  | 2B <sub>2</sub>  | 0.766            | 0.284 | 0.283 | 0.845            | 0.234           | 0.213 | 0.819            | 0.266 |          |  |
|                       | 1A <sub>2</sub>  | 1B <sub>1</sub>  | 0.466            | 0.238 | 0.238 | 0.467            | 0.266           | 0.265 | 0.533            | 0.224 |          |  |
|                       | 1A <sub>2</sub>  | 2A <sub>2</sub>  | 0.625            | 0.279 | 0.279 | 0.624            | 0.325           | 0.318 | 0.693            | 0.279 |          |  |
|                       | 1A <sub>u</sub>  | 1B <sub>g</sub>  | 1.496            | 0.026 | 0.026 | 1.497            | 0.078           | 0.067 | 1.408            | 0.028 |          |  |
| Glyoxal               | 1A <sub>u</sub>  | 2B <sub>g</sub>  | 4.296            | 0.138 | 0.137 | 4.241            | 0.313           | 0.251 | 4.098            | 0.173 |          |  |
|                       | 1B <sub>1</sub>  | 2A <sub>2</sub>  | 1.009            | 0.324 | 0.325 | 1.004            | 0.363           | 0.372 | 1.159            | 0.343 |          |  |
| Ketene                | 1B <sub>1</sub>  | 2A <sub>1</sub>  | 1.091            | 0.227 | 0.225 | 1.121            | 0.270           | 0.266 | 1.126            | 0.175 |          |  |
|                       | 1B <sub>1</sub>  | 1A <sub>2</sub>  | 0.453            | 0.217 | 0.216 | 0.452            | 0.238           | 0.253 | 0.510            | 0.202 |          |  |
| Methylenecyclopropene | 1B <sub>2</sub>  | 1A <sub>2</sub>  | 1.105            | 0.023 | 0.024 | 0.986            | 0.025           | 0.020 | 1.388            | 0.025 |          |  |
|                       | 2A <sub>g</sub>  | 2B <sub>1u</sub> | 0.558            | 0.098 | 0.097 | 0.657            | 0.206           | 0.235 | 0.737            | 0.196 |          |  |
| Pyrazine              | 2A <sub>g</sub>  | 2B <sub>2u</sub> | 0.505            | 0.244 | 0.244 | 0.504            | 0.303           | 0.301 | 0.603            | 0.263 |          |  |
|                       | 1B <sub>1u</sub> | 1B <sub>3g</sub> | 1.781            | 0.001 | 0.001 | 1.524            | 0.004           | 0.003 | 1.145            | 0.007 |          |  |
|                       | 2B <sub>2u</sub> | 1B <sub>3g</sub> | 0.631            | 0.220 | 0.219 | 0.630            | 0.219           | 0.226 | 0.686            | 0.203 |          |  |
|                       | 1A <sub>2</sub>  | 2B <sub>1</sub>  | 2.022            | 0.003 | 0.002 | 1.994            | 0.023           | 0.042 | 2.014            | 0.014 |          |  |
| Pyrrolone             | 1A <sub>2</sub>  | 1B <sub>1</sub>  | 0.669            | 0.225 | 0.225 | 0.670            | 0.248           | 0.260 | 0.690            | 0.099 |          |  |
|                       | 1A <sub>2</sub>  | 2A <sub>2</sub>  | 0.693            | 0.183 | 0.182 | 0.693            | 0.225           | 0.219 | 0.722            | 0.190 |          |  |

| Molecule   | State1           | State2           | BHandHLYP        |       |       |                  | BHandHLYP (TDA) |       |                  |       | EOM-CCSD |  |
|------------|------------------|------------------|------------------|-------|-------|------------------|-----------------|-------|------------------|-------|----------|--|
|            |                  |                  | $\Delta E_{m,n}$ | $f^l$ | $f^v$ | $\Delta E_{m,n}$ | $f^l$           | $f^v$ | $\Delta E_{m,n}$ | $f^v$ |          |  |
| Silylidene | 1A <sub>2</sub>  | 1B <sub>2</sub>  | 1.700            | 0.003 | 0.002 | 1.822            | 0.005           | 0.000 | 1.584            | 0.003 |          |  |
| Tetrazine  | 1B <sub>3u</sub> | 1B <sub>1g</sub> | 2.626            | 0.049 | 0.050 | 2.642            | 0.218           | 0.149 | 2.629            | 0.094 |          |  |
|            | 1B <sub>3u</sub> | 1B <sub>2g</sub> | 3.274            | 0.025 | 0.024 | 3.258            | 0.117           | 0.136 | 3.201            | 0.036 |          |  |
| Thiophene  | 1A <sub>2</sub>  | 1B <sub>1</sub>  | 0.179            | 0.036 | 0.037 | 0.192            | 0.048           | 0.035 | 0.102            | 0.013 |          |  |
| Water      | 1B <sub>1</sub>  | 1A <sub>2</sub>  | 1.575            | 0.266 | 0.267 | 1.563            | 0.297           | 0.325 | 1.756            | 0.293 |          |  |

Table S36: Excited State absorption data for B3LYP (TDA), and CAM-B3LYP (TDA).  $\Delta E_{m,n}$  [eV] and oscillator strengths in length, and velocity gauges,  $f^l$ ,  $f^v$  respectively. All data are obtained with dAVTZ basis set.

| Molecule        | State1           | State2           | B3LYP (TDA)      |       |       | CAM-B3LYP (TDA)  |       |       |
|-----------------|------------------|------------------|------------------|-------|-------|------------------|-------|-------|
|                 |                  |                  | $\Delta E_{m,n}$ | $f^l$ | $f^v$ | $\Delta E_{m,n}$ | $f^l$ | $f^v$ |
| Acetone         | 1B <sub>2</sub>  | 2A <sub>1</sub>  | 0.742            | 0.316 | 0.296 | 0.924            | 0.307 | 0.291 |
|                 | 1B <sub>2</sub>  | 2B <sub>2</sub>  | 0.878            | 0.284 | 0.283 | 0.944            | 0.311 | 0.306 |
|                 | 1B <sub>2</sub>  | 2A <sub>2</sub>  | 0.818            | 0.368 | 0.361 | 0.894            | 0.413 | 0.391 |
| Acrolein        | 1A''             | 2A''             | 2.817            | 0.175 | 0.149 | 3.174            | 0.118 | 0.087 |
| Ammonia         | 1A <sub>2</sub>  | 1E               | 1.084            | 0.308 | 0.322 | 1.345            | 0.343 | 0.357 |
|                 | 1A <sub>2</sub>  | 2A <sub>1</sub>  | 1.380            | 0.131 | 0.109 | 1.757            | 0.300 | 0.258 |
|                 | 1E               | 2A <sub>2</sub>  | 0.326            | 0.097 | 0.089 | 0.716            | 0.147 | 0.154 |
| Benzene         | 2A <sub>1</sub>  | 2A <sub>2</sub>  | 0.030            | 0.000 | 1.815 | 0.304            | 0.149 | 0.272 |
|                 | 1E <sub>1g</sub> | 1A <sub>2u</sub> | 0.458            | 0.142 | 0.142 | 0.480            | 0.126 | 0.126 |
|                 | 1E <sub>1g</sub> | 1E <sub>2u</sub> | 0.480            | 0.144 | 0.144 | 0.575            | 0.139 | 0.139 |
| Butadiene       | 1B <sub>g</sub>  | 1A <sub>u</sub>  | 0.259            | 0.151 | 0.162 | 0.279            | 0.136 | 0.151 |
|                 | 1B <sub>g</sub>  | 2A <sub>u</sub>  | 0.317            | 0.229 | 0.234 | 0.428            | 0.195 | 0.204 |
|                 | 1A <sub>u</sub>  | 2B <sub>g</sub>  | 0.550            | 0.026 | 0.028 | 0.774            | 0.063 | 0.066 |
| Carbon monoxide | 2A <sub>u</sub>  | 2B <sub>g</sub>  | 0.492            | 0.421 | 0.424 | 0.625            | 0.420 | 0.426 |
|                 | 2Σ <sup>+</sup>  | 3Σ <sup>+</sup>  | 0.321            | 0.175 | 0.297 | 0.413            | 0.158 | 0.255 |
|                 | 2Σ <sup>+</sup>  | 2Π               | 0.381            | 0.427 | 0.838 | 0.516            | 0.476 | 0.655 |
| Cyclopentadiene | 2Π               | 1Π               | 1.669            | 0.005 | 0.006 | 2.294            | 0.007 | 0.009 |
|                 | 2Σ <sup>+</sup>  | 1Π               | 1.287            | 0.040 | 0.015 | 1.779            | 0.053 | 0.026 |
|                 | 3Σ <sup>+</sup>  | 1Π               | 1.608            | 0.012 | 0.012 | 2.192            | 0.008 | 0.007 |
| Cyclopentadiene | 1B <sub>2</sub>  | 2A <sub>1</sub>  | 0.870            | 0.001 | 0.003 | 1.362            | 0.092 | 0.157 |
|                 | 1A <sub>2</sub>  | 1B <sub>1</sub>  | 0.491            | 0.305 | 0.306 | 0.565            | 0.272 | 0.272 |
|                 | 1A <sub>2</sub>  | 2B <sub>2</sub>  | 0.607            | 0.310 | 0.306 | 0.661            | 0.321 | 0.306 |

| Molecule              | State1           | State2           | B3LYP (TDA)      |       |       | CAM-B3LYP (TDA)  |       |       |
|-----------------------|------------------|------------------|------------------|-------|-------|------------------|-------|-------|
|                       |                  |                  | $\Delta E_{m,n}$ | $f^l$ | $f^v$ | $\Delta E_{m,n}$ | $f^l$ | $f^v$ |
| Cyclopropene          | 1A <sub>2</sub>  | 2A <sub>2</sub>  | 0.501            | 0.318 | 0.320 | 0.622            | 0.319 | 0.314 |
|                       | 2B <sub>1</sub>  | 3B <sub>1</sub>  | 0.350            | 0.074 | 0.076 | 0.350            | 0.072 | 0.085 |
|                       | 1B <sub>1</sub>  | 2A <sub>1</sub>  | 3.337            | 0.010 | 0.011 | 3.773            | 0.013 | 0.015 |
| Diazirine             | 1B <sub>2</sub>  | 2A <sub>1</sub>  | 0.564            | 0.178 | 0.164 | 0.563            | 0.123 | 0.106 |
|                       | 1A <sub>2</sub>  | 1B <sub>1</sub>  | 2.073            | 0.015 | 0.012 | 2.314            | 0.014 | 0.008 |
| Diazomethane          | 1B <sub>2</sub>  | 2A <sub>1</sub>  | 0.707            | 0.321 | 0.320 | 0.842            | 0.329 | 0.325 |
|                       | 1B <sub>2</sub>  | 2A <sub>2</sub>  | 0.898            | 0.293 | 0.284 | 1.040            | 0.309 | 0.306 |
|                       | 1A <sub>2</sub>  | 1B <sub>2</sub>  | 2.475            | 0.019 | 0.017 | 2.928            | 0.020 | 0.018 |
| Formaldehyde          | 2B <sub>2</sub>  | 2A <sub>2</sub>  | 0.165            | 0.012 | 0.014 | 0.298            | 0.009 | 0.010 |
|                       | 1A <sub>2</sub>  | 2A <sub>2</sub>  | 3.373            | 0.009 | 0.009 | 3.968            | 0.011 | 0.011 |
|                       | 1A <sub>2</sub>  | 2B <sub>2</sub>  | 0.942            | 0.096 | 0.079 | 0.873            | 0.242 | 0.216 |
| Furane                | 1A <sub>2</sub>  | 1B <sub>1</sub>  | 0.418            | 0.292 | 0.295 | 0.492            | 0.252 | 0.252 |
|                       | 1A <sub>2</sub>  | 2A <sub>2</sub>  | 0.530            | 0.321 | 0.322 | 0.662            | 0.326 | 0.320 |
| Glyoxal               | 1A <sub>u</sub>  | 1B <sub>g</sub>  | 1.509            | 0.143 | 0.136 | 1.503            | 0.091 | 0.082 |
|                       | 1A <sub>u</sub>  | 2B <sub>g</sub>  | 3.380            | 0.282 | 0.266 | 3.764            | 0.312 | 0.273 |
| Ketene                | 1B <sub>1</sub>  | 2A <sub>2</sub>  | 0.838            | 0.342 | 0.353 | 1.019            | 0.369 | 0.372 |
|                       | 1B <sub>1</sub>  | 2A <sub>1</sub>  | 0.944            | 0.301 | 0.288 | 1.127            | 0.269 | 0.265 |
| Methylenecyclopropene | 1B <sub>1</sub>  | 1A <sub>2</sub>  | 0.382            | 0.237 | 0.247 | 0.478            | 0.235 | 0.247 |
|                       | 1B <sub>2</sub>  | 1A <sub>2</sub>  | 1.112            | 0.019 | 0.017 | 1.183            | 0.025 | 0.022 |
|                       | 2A <sub>g</sub>  | 2B <sub>1u</sub> | 0.714            | 0.133 | 0.133 | 0.694            | 0.181 | 0.197 |
| Pyrazine              | 2A <sub>g</sub>  | 2B <sub>2u</sub> | 0.394            | 0.308 | 0.311 | 0.551            | 0.305 | 0.301 |
|                       | 1B <sub>1u</sub> | 1B <sub>3g</sub> | 0.368            | 0.175 | 0.179 | 1.084            | 0.012 | 0.012 |
| Pyridazine            | 2B <sub>2u</sub> | 1B <sub>3g</sub> | 0.553            | 0.229 | 0.232 | 0.647            | 0.189 | 0.197 |
|                       | 1A <sub>2</sub>  | 2B <sub>1</sub>  | 1.980            | 0.056 | 0.060 | 1.971            | 0.035 | 0.045 |
| Pyrrole               | 1A <sub>2</sub>  | 1B <sub>1</sub>  | 0.663            | 0.258 | 0.263 | 0.707            | 0.209 | 0.234 |
|                       | 1A <sub>2</sub>  | 2A <sub>2</sub>  | 0.660            | 0.201 | 0.201 | 0.726            | 0.218 | 0.214 |

| Molecule   | State1           | State2           | B3LYP (TDA)      |       |       | CAM-B3LYP (TDA)  |       |       |
|------------|------------------|------------------|------------------|-------|-------|------------------|-------|-------|
|            |                  |                  | $\Delta E_{m,n}$ | $f^l$ | $f^v$ | $\Delta E_{m,n}$ | $f^l$ | $f^v$ |
| Silylidene | 1A <sub>2</sub>  | 1B <sub>2</sub>  | 1.744            | 0.005 | 0.000 | 1.706            | 0.004 | 0.000 |
| Tetrazine  | 1B <sub>3u</sub> | 1B <sub>1g</sub> | 2.496            | 0.341 | 0.295 | 2.568            | 0.263 | 0.205 |
|            | 1B <sub>3u</sub> | 1B <sub>2g</sub> | 3.187            | 0.133 | 0.142 | 3.264            | 0.131 | 0.142 |
| Thiophene  | 1A <sub>2</sub>  | 1B <sub>1</sub>  | 0.158            | 0.044 | 0.039 | 0.148            | 0.027 | 0.013 |
| Water      | 1B <sub>1</sub>  | 1A <sub>2</sub>  | 1.324            | 0.301 | 0.311 | 1.542            | 0.318 | 0.328 |

Table S37: Excited State absorption data for LC-BLYP33 (TDA), and LC-BLYP47 (TDA).  $\Delta E_{m,n}$ [eV] and oscillator strengths in length, and velocity gauges,  $f^l$ ,  $f^v$  respectively. All data are obtained with dAVTZ basis set.

| Molecule        | State1           | State2           | LC-BLYP33 (TDA)  |       |       | LC-BLYP47 (TDA)  |       |       |
|-----------------|------------------|------------------|------------------|-------|-------|------------------|-------|-------|
|                 |                  |                  | $\Delta E_{m,n}$ | $f^l$ | $f^v$ | $\Delta E_{m,n}$ | $f^l$ | $f^v$ |
| Acetone         | 1B <sub>2</sub>  | 2A <sub>1</sub>  | 1.079            | 0.297 | 0.277 | 1.111            | 0.281 | 0.272 |
|                 | 1B <sub>2</sub>  | 2B <sub>2</sub>  | 1.035            | 0.302 | 0.295 | 1.060            | 0.294 | 0.288 |
|                 | 1B <sub>2</sub>  | 2A <sub>2</sub>  | 0.934            | 0.421 | 0.388 | 0.955            | 0.420 | 0.385 |
| Acrolein        | 1A''             | 2A''             | 3.165            | 0.090 | 0.068 | 3.577            | 0.037 | 0.026 |
| Ammonia         | 1A <sub>2</sub>  | 1E               | 1.427            | 0.356 | 0.357 | 1.523            | 0.347 | 0.357 |
|                 | 1A <sub>2</sub>  | 2A <sub>1</sub>  | 1.932            | 0.316 | 0.263 | 2.068            | 0.310 | 0.269 |
|                 | 1E               | 2A <sub>2</sub>  | 0.989            | 0.122 | 0.125 | 1.082            | 0.109 | 0.112 |
| Benzene         | 2A <sub>1</sub>  | 2A <sub>2</sub>  | 0.484            | 0.250 | 0.279 | 0.537            | 0.263 | 0.284 |
|                 | 1E <sub>1g</sub> | 1A <sub>2u</sub> | 0.497            | 0.130 | 0.078 | 0.482            | 0.126 | 0.075 |
|                 | 1E <sub>1g</sub> | 1E <sub>2u</sub> | 0.647            | 0.164 | 0.238 | 0.666            | 0.165 | 0.238 |
| Butadiene       | 1B <sub>g</sub>  | 1A <sub>u</sub>  | 0.294            | 0.131 | 0.146 | 0.311            | 0.132 | 0.154 |
|                 | 1B <sub>g</sub>  | 2A <sub>u</sub>  | 0.503            | 0.171 | 0.183 | 0.520            | 0.167 | 0.181 |
|                 | 1A <sub>u</sub>  | 2B <sub>g</sub>  | 0.876            | 0.098 | 0.105 | 0.887            | 0.145 | 0.159 |
| Carbon monoxide | 2A <sub>u</sub>  | 2B <sub>g</sub>  | 0.667            | 0.338 | 0.342 | 0.677            | 0.262 | 0.262 |
|                 | 2Σ <sup>+</sup>  | 3Σ <sup>+</sup>  | 0.426            | 0.132 | 0.238 | 0.473            | 0.128 | 0.221 |
|                 | 2Σ <sup>+</sup>  | 2Π               | 0.551            | 0.451 | 0.586 | 0.592            | 0.440 | 0.564 |
|                 | 2Π               | 1Π               | 2.268            | 0.008 | 0.010 | 2.986            | 0.010 | 0.012 |
|                 | 2Σ <sup>+</sup>  | 1Π               | 1.717            | 0.067 | 0.029 | 2.394            | 0.059 | 0.034 |
|                 | 3Σ <sup>+</sup>  | 1Π               | 2.142            | 0.006 | 0.006 | 2.867            | 0.003 | 0.002 |
| Cyclopentadiene | 1B <sub>2</sub>  | 2A <sub>1</sub>  | 1.407            | 0.147 | 0.257 | 1.805            | 0.155 | 0.211 |
|                 | 1A <sub>2</sub>  | 1B <sub>1</sub>  | 0.613            | 0.244 | 0.244 | 0.613            | 0.240 | 0.241 |
|                 | 1A <sub>2</sub>  | 2B <sub>2</sub>  | 0.682            | 0.326 | 0.305 | 0.692            | 0.327 | 0.303 |



| Molecule              | State1           | State2           | LC-BLYP33 (TDA)  |       |       | LC-BLYP47 (TDA)  |       |       |
|-----------------------|------------------|------------------|------------------|-------|-------|------------------|-------|-------|
|                       |                  |                  | $\Delta E_{m,n}$ | $f^l$ | $f^v$ | $\Delta E_{m,n}$ | $f^l$ | $f^v$ |
| Cyclopropene          | 1A <sub>2</sub>  | 2A <sub>2</sub>  | 0.712            | 0.310 | 0.302 | 0.746            | 0.309 | 0.299 |
|                       | 2B <sub>1</sub>  | 3B <sub>1</sub>  | 0.384            | 0.121 | 0.126 | 0.383            | 0.112 | 0.118 |
| Diazirine             | 1B <sub>1</sub>  | 2A <sub>1</sub>  | 3.790            | 0.015 | 0.017 | 4.282            | 0.014 | 0.017 |
|                       | 1B <sub>2</sub>  | 2A <sub>1</sub>  | 0.534            | 0.098 | 0.083 | 0.555            | 0.064 | 0.043 |
| Diazomethane          | 1A <sub>2</sub>  | 1B <sub>1</sub>  | 2.294            | 0.014 | 0.006 | 2.664            | 0.012 | 0.005 |
| Formaldehyde          | 1B <sub>2</sub>  | 2A <sub>1</sub>  | 0.892            | 0.325 | 0.322 | 0.940            | 0.323 | 0.319 |
|                       | 1B <sub>2</sub>  | 2A <sub>2</sub>  | 1.057            | 0.313 | 0.310 | 1.131            | 0.311 | 0.305 |
|                       | 1A <sub>2</sub>  | 1B <sub>2</sub>  | 2.862            | 0.018 | 0.019 | 3.464            | 0.018 | 0.016 |
|                       | 2B <sub>2</sub>  | 2A <sub>2</sub>  | 0.288            | 0.004 | 0.005 | 0.352            | 0.003 | 0.005 |
| Furane                | 1A <sub>2</sub>  | 2A <sub>2</sub>  | 3.918            | 0.012 | 0.011 | 4.595            | 0.011 | 0.011 |
|                       | 1A <sub>2</sub>  | 2B <sub>2</sub>  | 0.891            | 0.278 | 0.240 | 0.844            | 0.318 | 0.283 |
|                       | 1A <sub>2</sub>  | 1B <sub>1</sub>  | 0.537            | 0.219 | 0.219 | 0.545            | 0.213 | 0.214 |
|                       | 1A <sub>2</sub>  | 2A <sub>2</sub>  | 0.750            | 0.323 | 0.313 | 0.790            | 0.320 | 0.308 |
| Glyoxal               | 1A <sub>u</sub>  | 1B <sub>g</sub>  | 1.492            | 0.079 | 0.073 | 1.455            | 0.057 | 0.049 |
|                       | 1A <sub>u</sub>  | 2B <sub>g</sub>  | 3.707            | 0.309 | 0.275 | 4.315            | 0.307 | 0.252 |
| Ketene                | 1B <sub>1</sub>  | 2A <sub>2</sub>  | 1.090            | 0.379 | 0.371 | 1.159            | 0.377 | 0.370 |
|                       | 1B <sub>1</sub>  | 2A <sub>1</sub>  | 1.196            | 0.247 | 0.248 | 1.160            | 0.170 | 0.184 |
| Methylenecyclopropene | 1B <sub>1</sub>  | 1A <sub>2</sub>  | 0.544            | 0.240 | 0.250 | 0.581            | 0.243 | 0.259 |
|                       | 1B <sub>2</sub>  | 1A <sub>2</sub>  | 1.240            | 0.026 | 0.023 | 1.216            | 0.028 | 0.022 |
| Pyrazine              | 2A <sub>g</sub>  | 2B <sub>1u</sub> | 0.703            | 0.119 | 0.136 | 0.622            | 0.099 | 0.140 |
|                       | 2A <sub>g</sub>  | 2B <sub>2u</sub> | 0.684            | 0.297 | 0.288 | 0.724            | 0.289 | 0.282 |
|                       | 1B <sub>1u</sub> | 1B <sub>3g</sub> | 1.067            | 0.026 | 0.024 | 0.724            | 0.218 | 0.215 |
|                       | 2B <sub>2u</sub> | 1B <sub>3g</sub> | 0.625            | 0.135 | 0.143 | 0.623            | 0.137 | 0.148 |
| Pyridazine            | 1A <sub>2</sub>  | 2B <sub>1</sub>  | 1.971            | 0.034 | 0.044 | 1.981            | 0.023 | 0.043 |
| Pyrrole               | 1A <sub>2</sub>  | 1B <sub>1</sub>  | 0.724            | 0.155 | 0.199 | 0.705            | 0.184 | 0.220 |
|                       | 1A <sub>2</sub>  | 2A <sub>2</sub>  | 0.762            | 0.219 | 0.215 | 0.756            | 0.235 | 0.228 |

| Molecule   | State1           | State2           | LC-BLYP33 (TDA)  |       |       |  | LC-BLYP47 (TDA)  |       |       |  |
|------------|------------------|------------------|------------------|-------|-------|--|------------------|-------|-------|--|
|            |                  |                  | $\Delta E_{m,n}$ | $f^l$ | $f^v$ |  | $\Delta E_{m,n}$ | $f^l$ | $f^v$ |  |
| Silylidene | 1A <sub>2</sub>  | 1B <sub>2</sub>  | 1.585            | 0.003 | 0.003 |  | 1.594            | 0.003 | 0.003 |  |
| Tetrazine  | 1B <sub>3u</sub> | 1B <sub>1g</sub> | 2.524            | 0.255 | 0.201 |  | 2.559            | 0.197 | 0.136 |  |
|            | 1B <sub>3u</sub> | 1B <sub>2g</sub> | 3.294            | 0.136 | 0.135 |  | 3.375            | 0.125 | 0.142 |  |
| Thiophene  | 1A <sub>2</sub>  | 1B <sub>1</sub>  | 0.161            | 0.022 | 0.002 |  | 0.294            | 0.001 | 0.070 |  |
| Water      | 1B <sub>1</sub>  | 1A <sub>2</sub>  | 1.603            | 0.331 | 0.328 |  | 1.709            | 0.312 | 0.317 |  |

Table S38: Theoretical  $f$  in different gauges and  $\Delta E_{m,n}$  of the  $1A_2$  (Ryd,  $\pi$ -3s)  $\rightarrow$   $1B_1$  (Ryd,  $\pi$ -3p) transition of thiophene obtained with different basis sets and QR-CC3.

| Basis Set | $\Delta E_{m,n}$ [eV] | $f^l$ | $f^v$  | $f^m$  |
|-----------|-----------------------|-------|--------|--------|
| AVDZ      | 0.119                 | 0.017 | 0.008  | -0.012 |
| dAVDZ     | 0.146                 | 0.023 | 0.022  | -0.023 |
| AVTZ      | 0.005                 | 0.001 | 0.005  | 0.003  |
| dAVTZ     | 0.009                 | 0.001 | -0.004 | -0.001 |

## S4 Statistics

### S4.1 Reference Value

Table S39: MSE, MAE, RMSE, and SDE of transition dipole moments  $\mu$  [a.u.] and oscillator strengths in length gauge ( $f^l$ ) computed for small set of transitions and seven basis sets. All values are compared with CC3/dAVQZ.

| Basis Set | $f^l$  |       |       |       | $\mu$  |       |       |       |
|-----------|--------|-------|-------|-------|--------|-------|-------|-------|
|           | MSE    | MAE   | RMSE  | SDE   | MSE    | MAE   | RMSE  | SDE   |
| AVDZ      | -0.032 | 0.061 | 0.101 | 0.096 | -0.701 | 0.726 | 1.383 | 1.192 |
| dAVDZ     | 0.002  | 0.008 | 0.012 | 0.012 | 0.035  | 0.082 | 0.123 | 0.118 |
| tAVDZ     | 0.006  | 0.008 | 0.014 | 0.012 | 0.070  | 0.079 | 0.135 | 0.116 |
| AVTZ      | -0.028 | 0.055 | 0.091 | 0.087 | -0.517 | 0.530 | 1.078 | 0.945 |
| dAVTZ     | 0.000  | 0.002 | 0.004 | 0.004 | 0.006  | 0.023 | 0.040 | 0.040 |
| tAVTZ     | 0.004  | 0.007 | 0.016 | 0.015 | 0.036  | 0.059 | 0.127 | 0.122 |
| AVQZ      | -0.022 | 0.047 | 0.078 | 0.075 | -0.389 | 0.406 | 0.843 | 0.747 |

Table S40: MSE, MAE, RMSE, SDE, MSPE, and MAPE of oscillator strengths in velocity ( $f^v$ ) and mixed ( $f^m$ ) gauges obtained with QR-CC3, QR-CCSD, and QR-CC2 and dAVTZ basis set. oscillator strengths in length gauge ( $f^l$ ) obtained at the corresponding level of theory serve as references.

| Method  | MSE     | MAE    | RMSE   | SDE    | MSPE    | MAPE   |
|---------|---------|--------|--------|--------|---------|--------|
| $f^v$   |         |        |        |        |         |        |
| QR-CC3  | 0.0018  | 0.0021 | 0.0043 | 0.0039 | -0.0062 | 0.0471 |
| QR-CCSD | -0.0097 | 0.0137 | 0.0225 | 0.0203 | -0.3028 | 0.3552 |
| QR-CC2  | -0.0031 | 0.0072 | 0.0116 | 0.0112 | -0.1162 | 0.1553 |
| $f^m$   |         |        |        |        |         |        |
| QR-CC3  | 0.0009  | 0.0011 | 0.0021 | 0.0019 | 0.0205  | 0.0339 |
| QR-CCSD | 0.0019  | 0.0027 | 0.0044 | 0.0040 | 0.1052  | 0.1483 |
| QR-CC2  | 0.0021  | 0.0031 | 0.0053 | 0.0048 | -0.0290 | 0.1102 |

### S4.2 Basis Set Effect

Table S41: MSE, MAE, RMSE, and SDE of oscillator strengths in length gauge ( $f^l$ ) computed for QR-CC3 (QR-CC3/dAVTZ reference) and ISR-ADC(2) (ISR-ADC(2)/dAVTZ reference) on all transitions.

| Basis Set | QR-CC3 |       |       |       | ISR-ADC(2) |       |       |       |
|-----------|--------|-------|-------|-------|------------|-------|-------|-------|
|           | MSE    | MAE   | RMSE  | SDE   | MSE        | MAE   | RMSE  | SDE   |
| AVDZ      | -0.011 | 0.020 | 0.047 | 0.045 | -0.011     | 0.027 | 0.051 | 0.049 |
| dAVDZ     | 0.002  | 0.004 | 0.007 | 0.007 | 0.001      | 0.007 | 0.014 | 0.014 |
| AVTZ      | -0.009 | 0.017 | 0.042 | 0.040 | -0.009     | 0.018 | 0.039 | 0.037 |

Table S42: MSE, MAE, RMSE, and SDE of oscillator strengths in length gauge ( $f^l$ ) computed for QR-CCSD (QR-CCSD/dAVTZ reference) and QR-CC2 (QR-CC2/dAVTZ reference) on all transitions.

| Basis Set | QR-CCSD |       |       |       | QR-CC2 |       |       |       |
|-----------|---------|-------|-------|-------|--------|-------|-------|-------|
|           | MSE     | MAE   | RMSE  | SDE   | MSE    | MAE   | RMSE  | SDE   |
| AVDZ      | -0.011  | 0.021 | 0.046 | 0.045 | -0.013 | 0.025 | 0.047 | 0.045 |
| dAVDZ     | 0.002   | 0.005 | 0.009 | 0.008 | -0.001 | 0.011 | 0.028 | 0.028 |
| AVTZ      | -0.009  | 0.017 | 0.041 | 0.040 | -0.009 | 0.020 | 0.041 | 0.040 |

Table S43: MSE, MAE, RMSE, and SDE of oscillator strengths in length gauge ( $f^l$ ) computed for QR-CC3 with different basis sets on all transitions, and divided by transition character. All values are compared with QR-CC3/dAVTZ.

| Basis Set       | MSE    | MAE   | RMSE  | SDE   |
|-----------------|--------|-------|-------|-------|
| Rydberg-Rydberg |        |       |       |       |
| AVDZ            | -0.017 | 0.028 | 0.058 | 0.055 |
| dAVDZ           | 0.002  | 0.004 | 0.007 | 0.007 |
| AVTZ            | -0.013 | 0.024 | 0.051 | 0.049 |
| Rydberg-valence |        |       |       |       |
| AVDZ            | -0.003 | 0.009 | 0.017 | 0.017 |
| dAVDZ           | 0.005  | 0.005 | 0.009 | 0.008 |
| AVTZ            | -0.004 | 0.007 | 0.016 | 0.015 |
| valence-valence |        |       |       |       |
| AVDZ            | 0.001  | 0.001 | 0.002 | 0.001 |
| dAVDZ           | 0.001  | 0.001 | 0.001 | 0.001 |
| AVTZ            | 0.000  | 0.000 | 0.001 | 0.000 |

### S4.3 Methods Benchmarks

Table S44: MSE, MAE, RMSE, SDE, MSPE, and MAPE of oscillator strengths in length gauge ( $f^l$ ) computed for all methods, and on all transitions. All values are compared with QR-CC3/dAVTZ.

| Method          | MSE    | MAE   | RMSE  | SDE   | MSPE   | MAPE  |
|-----------------|--------|-------|-------|-------|--------|-------|
| EOM-CCSD        | 0.008  | 0.009 | 0.014 | 0.011 | 0.387  | 0.408 |
| QR-CCSD         | 0.005  | 0.006 | 0.009 | 0.008 | 0.323  | 0.348 |
| QR-CC2          | 0.014  | 0.020 | 0.029 | 0.026 | 1.134  | 1.175 |
| ISR-ADC(3)      | -0.002 | 0.009 | 0.019 | 0.019 | -0.049 | 0.132 |
| ISR-ADC(2)      | 0.018  | 0.022 | 0.031 | 0.025 | 0.831  | 0.881 |
| B3LYP           | 0.012  | 0.036 | 0.067 | 0.065 | 0.834  | 1.039 |
| CAM-B3LYP       | 0.007  | 0.015 | 0.037 | 0.036 | 0.461  | 0.548 |
| BHandHLYP       | 0.004  | 0.031 | 0.068 | 0.068 | 0.795  | 1.003 |
| LC-BLYP33       | -0.003 | 0.027 | 0.056 | 0.056 | 0.412  | 0.600 |
| LC-BLYP47       | -0.006 | 0.031 | 0.055 | 0.054 | 0.012  | 0.328 |
| B3LYP (TDA)     | 0.031  | 0.062 | 0.091 | 0.086 | 2.304  | 2.533 |
| CAM-B3LYP (TDA) | 0.036  | 0.044 | 0.066 | 0.056 | 1.126  | 1.196 |
| BHandHLYP (TDA) | 0.036  | 0.045 | 0.067 | 0.057 | 1.422  | 1.522 |
| LC-BLYP33 (TDA) | 0.033  | 0.042 | 0.063 | 0.053 | 1.102  | 1.195 |
| LC-BLYP47 (TDA) | 0.030  | 0.044 | 0.067 | 0.061 | 1.452  | 1.596 |

Table S45: MSE, MAE, RMSE, and SDE of  $\Delta E_{m,n}$  [eV] and  $\Delta E_{0,n}$  [eV] computed for all methods, and on all transitions. All values are compared with QR-CC3/dAVTZ.

| Method          | $\Delta E_{m,n}$ |       |       |       | $\Delta E_{0,n}$ |       |       |       |
|-----------------|------------------|-------|-------|-------|------------------|-------|-------|-------|
|                 | MSE              | MAE   | RMSE  | SDE   | MSE              | MAE   | RMSE  | SDE   |
| EOM-CCSD        | 0.024            | 0.057 | 0.106 | 0.104 | 0.126            | 0.127 | 0.169 | 0.113 |
| QR-CCSD         | 0.023            | 0.057 | 0.106 | 0.104 | 0.125            | 0.126 | 0.169 | 0.114 |
| QR-CC2          | -0.083           | 0.123 | 0.203 | 0.185 | -0.138           | 0.206 | 0.284 | 0.249 |
| ISR-ADC(3)      | 0.025            | 0.078 | 0.151 | 0.149 | -0.018           | 0.192 | 0.229 | 0.228 |
| ISR-ADC(2)      | -0.058           | 0.117 | 0.181 | 0.171 | -0.111           | 0.202 | 0.292 | 0.270 |
| B3LYP           | -0.268           | 0.287 | 0.385 | 0.276 | -0.637           | 0.638 | 0.722 | 0.340 |
| CAM-B3LYP       | -0.065           | 0.137 | 0.190 | 0.178 | -0.188           | 0.229 | 0.288 | 0.219 |
| BHandHLYP       | -0.017           | 0.173 | 0.235 | 0.235 | 0.002            | 0.255 | 0.306 | 0.306 |
| LC-BLYP33       | -0.023           | 0.143 | 0.209 | 0.208 | -0.148           | 0.217 | 0.301 | 0.262 |
| LC-BLYP47       | 0.132            | 0.192 | 0.307 | 0.277 | 0.319            | 0.349 | 0.413 | 0.263 |
| B3LYP (TDA)     | -0.276           | 0.305 | 0.422 | 0.319 | -0.610           | 0.618 | 0.710 | 0.364 |
| CAM-B3LYP (TDA) | -0.091           | 0.142 | 0.204 | 0.183 | -0.157           | 0.222 | 0.280 | 0.232 |
| BHandHLYP (TDA) | -0.046           | 0.155 | 0.206 | 0.201 | 0.037            | 0.261 | 0.316 | 0.314 |
| LC-BLYP33 (TDA) | -0.057           | 0.122 | 0.201 | 0.192 | -0.115           | 0.206 | 0.293 | 0.270 |
| LC-BLYP47 (TDA) | 0.066            | 0.130 | 0.214 | 0.203 | 0.363            | 0.373 | 0.437 | 0.244 |

Table S46: MSE, MAE, RMSE, and SDE of oscillator strengths in length gauge ( $f^l$ ) computed for all methods, on all transitions, divided by transition character. All values are compared with QR-CC3/dAVTZ.

| Method          | MSE    | MAE   | RMSE  | SDE   |
|-----------------|--------|-------|-------|-------|
| Rydberg-Rydberg |        |       |       |       |
| EOM-CCSD        | 0.008  | 0.009 | 0.010 | 0.007 |
| QR-CCSD         | 0.004  | 0.006 | 0.007 | 0.005 |
| QR-CC2          | 0.009  | 0.018 | 0.022 | 0.020 |
| ISR-ADC(3)      | 0.001  | 0.009 | 0.019 | 0.019 |
| ISR-ADC(2)      | 0.014  | 0.020 | 0.024 | 0.020 |
| B3LYP           | 0.013  | 0.047 | 0.080 | 0.079 |
| CAM-B3LYP       | 0.009  | 0.019 | 0.045 | 0.044 |
| BHandHLYP       | 0.004  | 0.044 | 0.085 | 0.084 |
| LC-BLYP33       | -0.007 | 0.037 | 0.069 | 0.069 |
| LC-BLYP47       | -0.009 | 0.040 | 0.066 | 0.065 |
| B3LYP (TDA)     | 0.012  | 0.058 | 0.082 | 0.081 |
| CAM-B3LYP (TDA) | 0.029  | 0.040 | 0.057 | 0.050 |
| BHandHLYP (TDA) | 0.035  | 0.048 | 0.066 | 0.056 |
| LC-BLYP33 (TDA) | 0.025  | 0.037 | 0.051 | 0.045 |
| LC-BLYP47 (TDA) | 0.022  | 0.042 | 0.056 | 0.052 |
| Rydberg-valence |        |       |       |       |
| EOM-CCSD        | 0.001  | 0.002 | 0.002 | 0.002 |
| QR-CCSD         | 0.001  | 0.001 | 0.002 | 0.002 |
| QR-CC2          | 0.020  | 0.021 | 0.046 | 0.041 |
| ISR-ADC(3)      | -0.000 | 0.002 | 0.002 | 0.002 |
| ISR-ADC(2)      | 0.006  | 0.008 | 0.015 | 0.013 |
| B3LYP           | 0.017  | 0.020 | 0.038 | 0.034 |
| CAM-B3LYP       | 0.006  | 0.008 | 0.016 | 0.015 |
| BHandHLYP       | 0.006  | 0.009 | 0.017 | 0.016 |
| LC-BLYP33       | 0.002  | 0.009 | 0.015 | 0.015 |
| LC-BLYP47       | -0.010 | 0.017 | 0.029 | 0.028 |
| B3LYP (TDA)     | 0.039  | 0.043 | 0.073 | 0.062 |
| CAM-B3LYP (TDA) | 0.016  | 0.018 | 0.033 | 0.029 |
| BHandHLYP (TDA) | 0.015  | 0.017 | 0.034 | 0.030 |
| LC-BLYP33 (TDA) | 0.014  | 0.016 | 0.027 | 0.023 |
| LC-BLYP47 (TDA) | 0.022  | 0.029 | 0.069 | 0.065 |
| valence-valence |        |       |       |       |
| EOM-CCSD        | 0.020  | 0.020 | 0.028 | 0.019 |
| QR-CCSD         | 0.011  | 0.011 | 0.017 | 0.013 |
| QR-CC2          | 0.024  | 0.024 | 0.031 | 0.020 |
| ISR-ADC(3)      | -0.013 | 0.017 | 0.028 | 0.025 |
| ISR-ADC(2)      | 0.044  | 0.044 | 0.057 | 0.035 |
| B3LYP           | 0.002  | 0.014 | 0.018 | 0.017 |

| Method          | MSE   | MAE   | RMSE  | SDE   |
|-----------------|-------|-------|-------|-------|
| CAM-B3LYP       | 0.005 | 0.007 | 0.009 | 0.008 |
| BHandHLYP       | 0.001 | 0.009 | 0.012 | 0.012 |
| LC-BLYP33       | 0.009 | 0.011 | 0.015 | 0.012 |
| LC-BLYP47       | 0.007 | 0.014 | 0.021 | 0.019 |
| B3LYP (TDA)     | 0.094 | 0.100 | 0.132 | 0.093 |
| CAM-B3LYP (TDA) | 0.085 | 0.085 | 0.111 | 0.072 |
| BHandHLYP (TDA) | 0.062 | 0.065 | 0.094 | 0.071 |
| LC-BLYP33 (TDA) | 0.086 | 0.086 | 0.112 | 0.072 |
| LC-BLYP47 (TDA) | 0.069 | 0.069 | 0.098 | 0.070 |

Table S47: MSE, MAE, RMSE, and SDE of oscillator strengths in length gauge ( $f^l$ ) computed for all methods, on all transitions, and divided by molecular size. All values are compared with QR-CC3/dAVTZ.

| Method                 | MSE    | MAE   | RMSE  | SDE   |
|------------------------|--------|-------|-------|-------|
| 1-3 non-hydrogen atoms |        |       |       |       |
| EOM-CCSD               | 0.002  | 0.003 | 0.005 | 0.004 |
| QR-CCSD                | 0.001  | 0.002 | 0.003 | 0.003 |
| QR-CC2                 | 0.007  | 0.008 | 0.014 | 0.012 |
| ISR-ADC(3)             | 0.001  | 0.004 | 0.006 | 0.006 |
| ISR-ADC(2)             | 0.006  | 0.007 | 0.011 | 0.009 |
| B3LYP                  | 0.018  | 0.024 | 0.048 | 0.044 |
| CAM-B3LYP              | 0.017  | 0.019 | 0.053 | 0.050 |
| BHandHLYP              | 0.021  | 0.025 | 0.068 | 0.065 |
| LC-BLYP33              | 0.011  | 0.019 | 0.044 | 0.043 |
| LC-BLYP47              | 0.000  | 0.023 | 0.046 | 0.046 |
| B3LYP (TDA)            | 0.026  | 0.030 | 0.056 | 0.050 |
| CAM-B3LYP (TDA)        | 0.027  | 0.031 | 0.060 | 0.054 |
| BHandHLYP (TDA)        | 0.031  | 0.032 | 0.062 | 0.054 |
| LC-BLYP33 (TDA)        | 0.026  | 0.029 | 0.054 | 0.047 |
| LC-BLYP47 (TDA)        | 0.016  | 0.023 | 0.047 | 0.044 |
| 4-6 non-hydrogen atoms |        |       |       |       |
| EOM-CCSD               | 0.012  | 0.013 | 0.018 | 0.013 |
| QR-CCSD                | 0.007  | 0.008 | 0.011 | 0.009 |
| QR-CC2                 | 0.018  | 0.026 | 0.036 | 0.031 |
| ISR-ADC(3)             | -0.002 | 0.012 | 0.024 | 0.024 |
| ISR-ADC(2)             | 0.026  | 0.029 | 0.038 | 0.028 |
| B3LYP                  | 0.013  | 0.025 | 0.036 | 0.033 |
| CAM-B3LYP              | 0.007  | 0.010 | 0.020 | 0.019 |
| BHandHLYP              | -0.002 | 0.035 | 0.071 | 0.071 |
| LC-BLYP33              | -0.006 | 0.031 | 0.062 | 0.062 |
| LC-BLYP47              | -0.004 | 0.034 | 0.058 | 0.058 |
| B3LYP (TDA)            | 0.051  | 0.071 | 0.095 | 0.080 |
| CAM-B3LYP (TDA)        | 0.047  | 0.051 | 0.071 | 0.053 |
| BHandHLYP (TDA)        | 0.048  | 0.052 | 0.070 | 0.050 |
| LC-BLYP33 (TDA)        | 0.040  | 0.051 | 0.071 | 0.059 |
| LC-BLYP47 (TDA)        | 0.042  | 0.061 | 0.081 | 0.070 |



Table S48: MAPE of oscillator strengths in length gauge ( $f^l$ ) computed for all methods, on all transitions, and divided by the magnitude of  $f$ . All values are compared with QR-QR-CC3/dAVTZ.

| Method          | $f < 0.05$ | $0.05 < f < 0.15$ | $f > 0.15$ |
|-----------------|------------|-------------------|------------|
| EOM-CCSD        | 1.125      | 0.140             | 0.039      |
| QR-CCSD         | 0.995      | 0.084             | 0.024      |
| QR-CC2          | 3.390      | 0.211             | 0.092      |
| ISR-ADC(3)      | 0.252      | 0.153             | 0.041      |
| ISR-ADC(2)      | 2.385      | 0.361             | 0.088      |
| B3LYP           | 2.677      | 0.383             | 0.214      |
| CAM-B3LYP       | 1.479      | 0.156             | 0.088      |
| BHandHLYP       | 2.589      | 0.425             | 0.178      |
| LC-BLYP33       | 1.421      | 0.368             | 0.143      |
| LC-BLYP47       | 0.480      | 0.470             | 0.163      |
| B3LYP (TDA)     | 6.851      | 0.975             | 0.282      |
| CAM-B3LYP (TDA) | 2.990      | 0.678             | 0.205      |
| BHandHLYP (TDA) | 3.950      | 0.726             | 0.221      |
| LC-BLYP33 (TDA) | 3.041      | 0.639             | 0.185      |
| LC-BLYP47 (TDA) | 4.281      | 0.666             | 0.180      |

## References

- (1) V  ril, M.; Scemama, A.; Caffarel, M.; Lipparini, F.; Boggio-Pasqua, M.; Jacquemin, D.; Loos, P.-F. QUESTDB: A Database of Highly Accurate Excitation Energies for the Electronic Structure Community. *WIREs Comput. Mol. Sci.* **2021**, *11*, e1517.
